# Supplementary material for: Estimating the Impact of BGP Prefix Hijacking
Source: arXiv:2105.02346 source file (2021-05-05)
Supplement: Supplementary file 1 [file appendix.tex]

\section{Visualization of the predictions of the regression models for hijack impact predictions}\label{appendix:visualization-ML-boundaries}
Figure~\ref{fig:ML-2D-visualization-Impact-closeness}
\begin{figure}
\centering
\subfigure[MLP Regression]{\includegraphics[width=0.49\linewidth]{./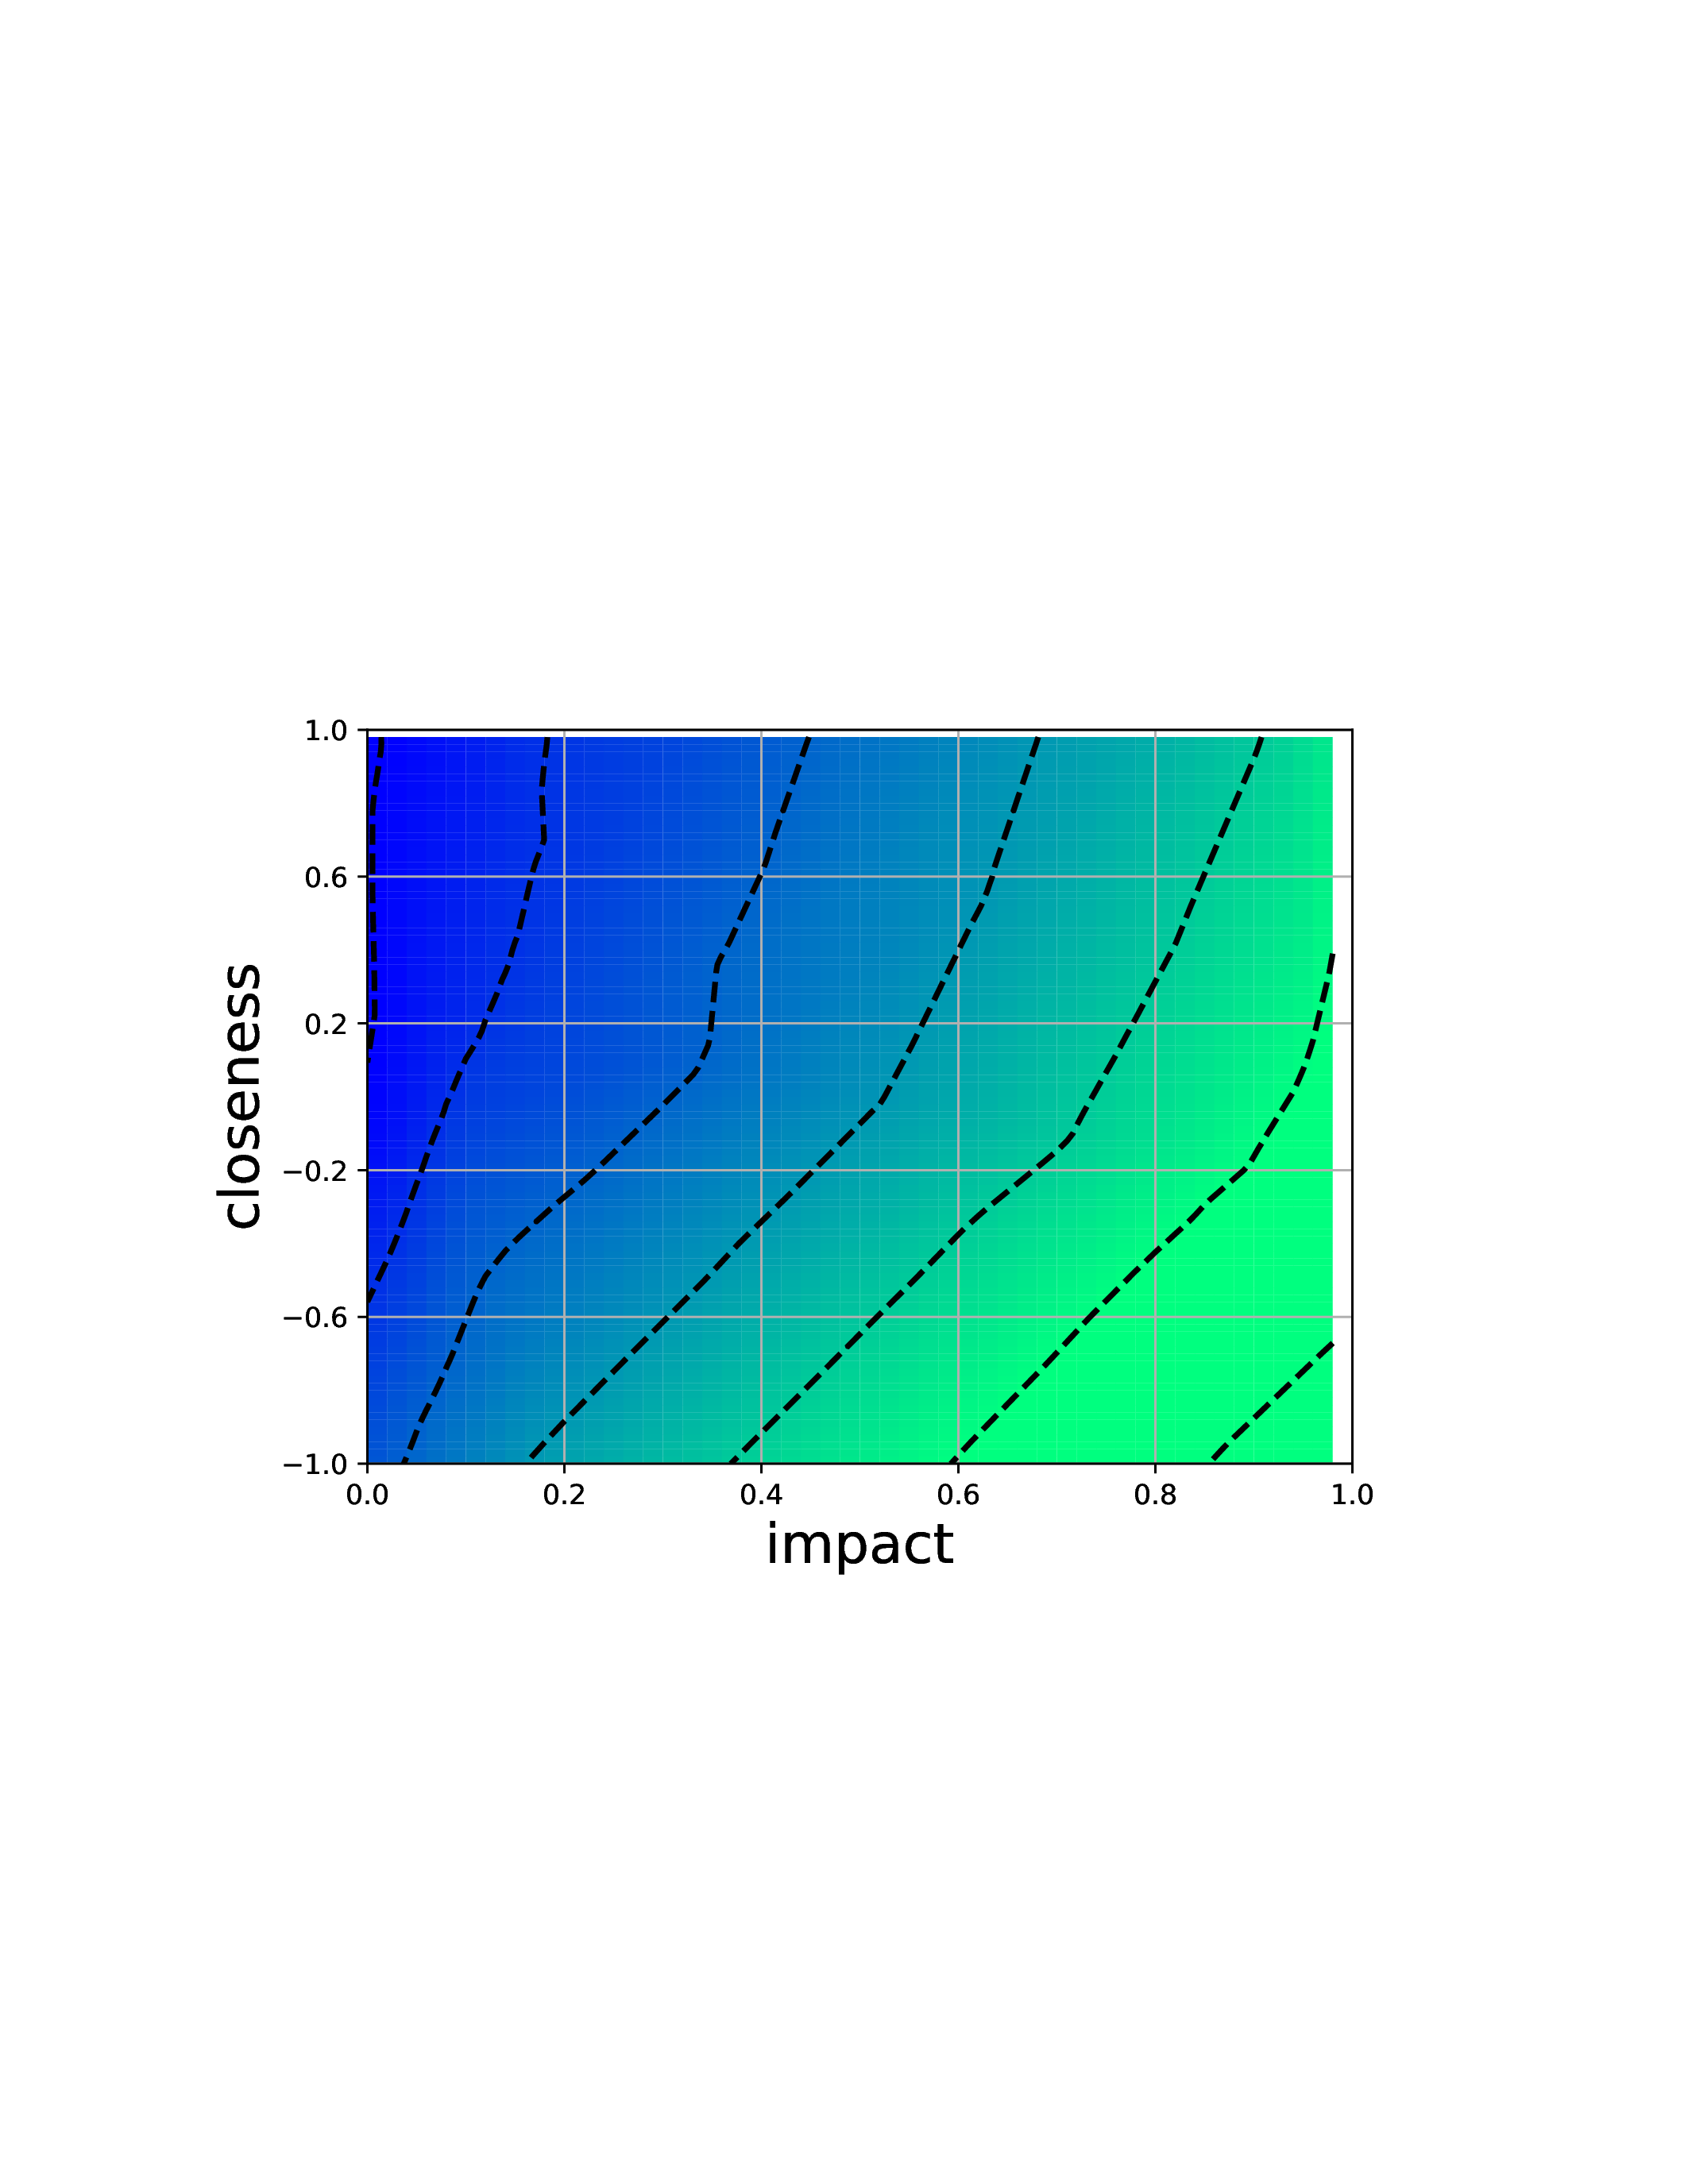}\label{fig:ML-2D-visualization-Impact-closeness-MLPR}}
\subfigure[Linear Regression]{\includegraphics[width=0.49\linewidth]{./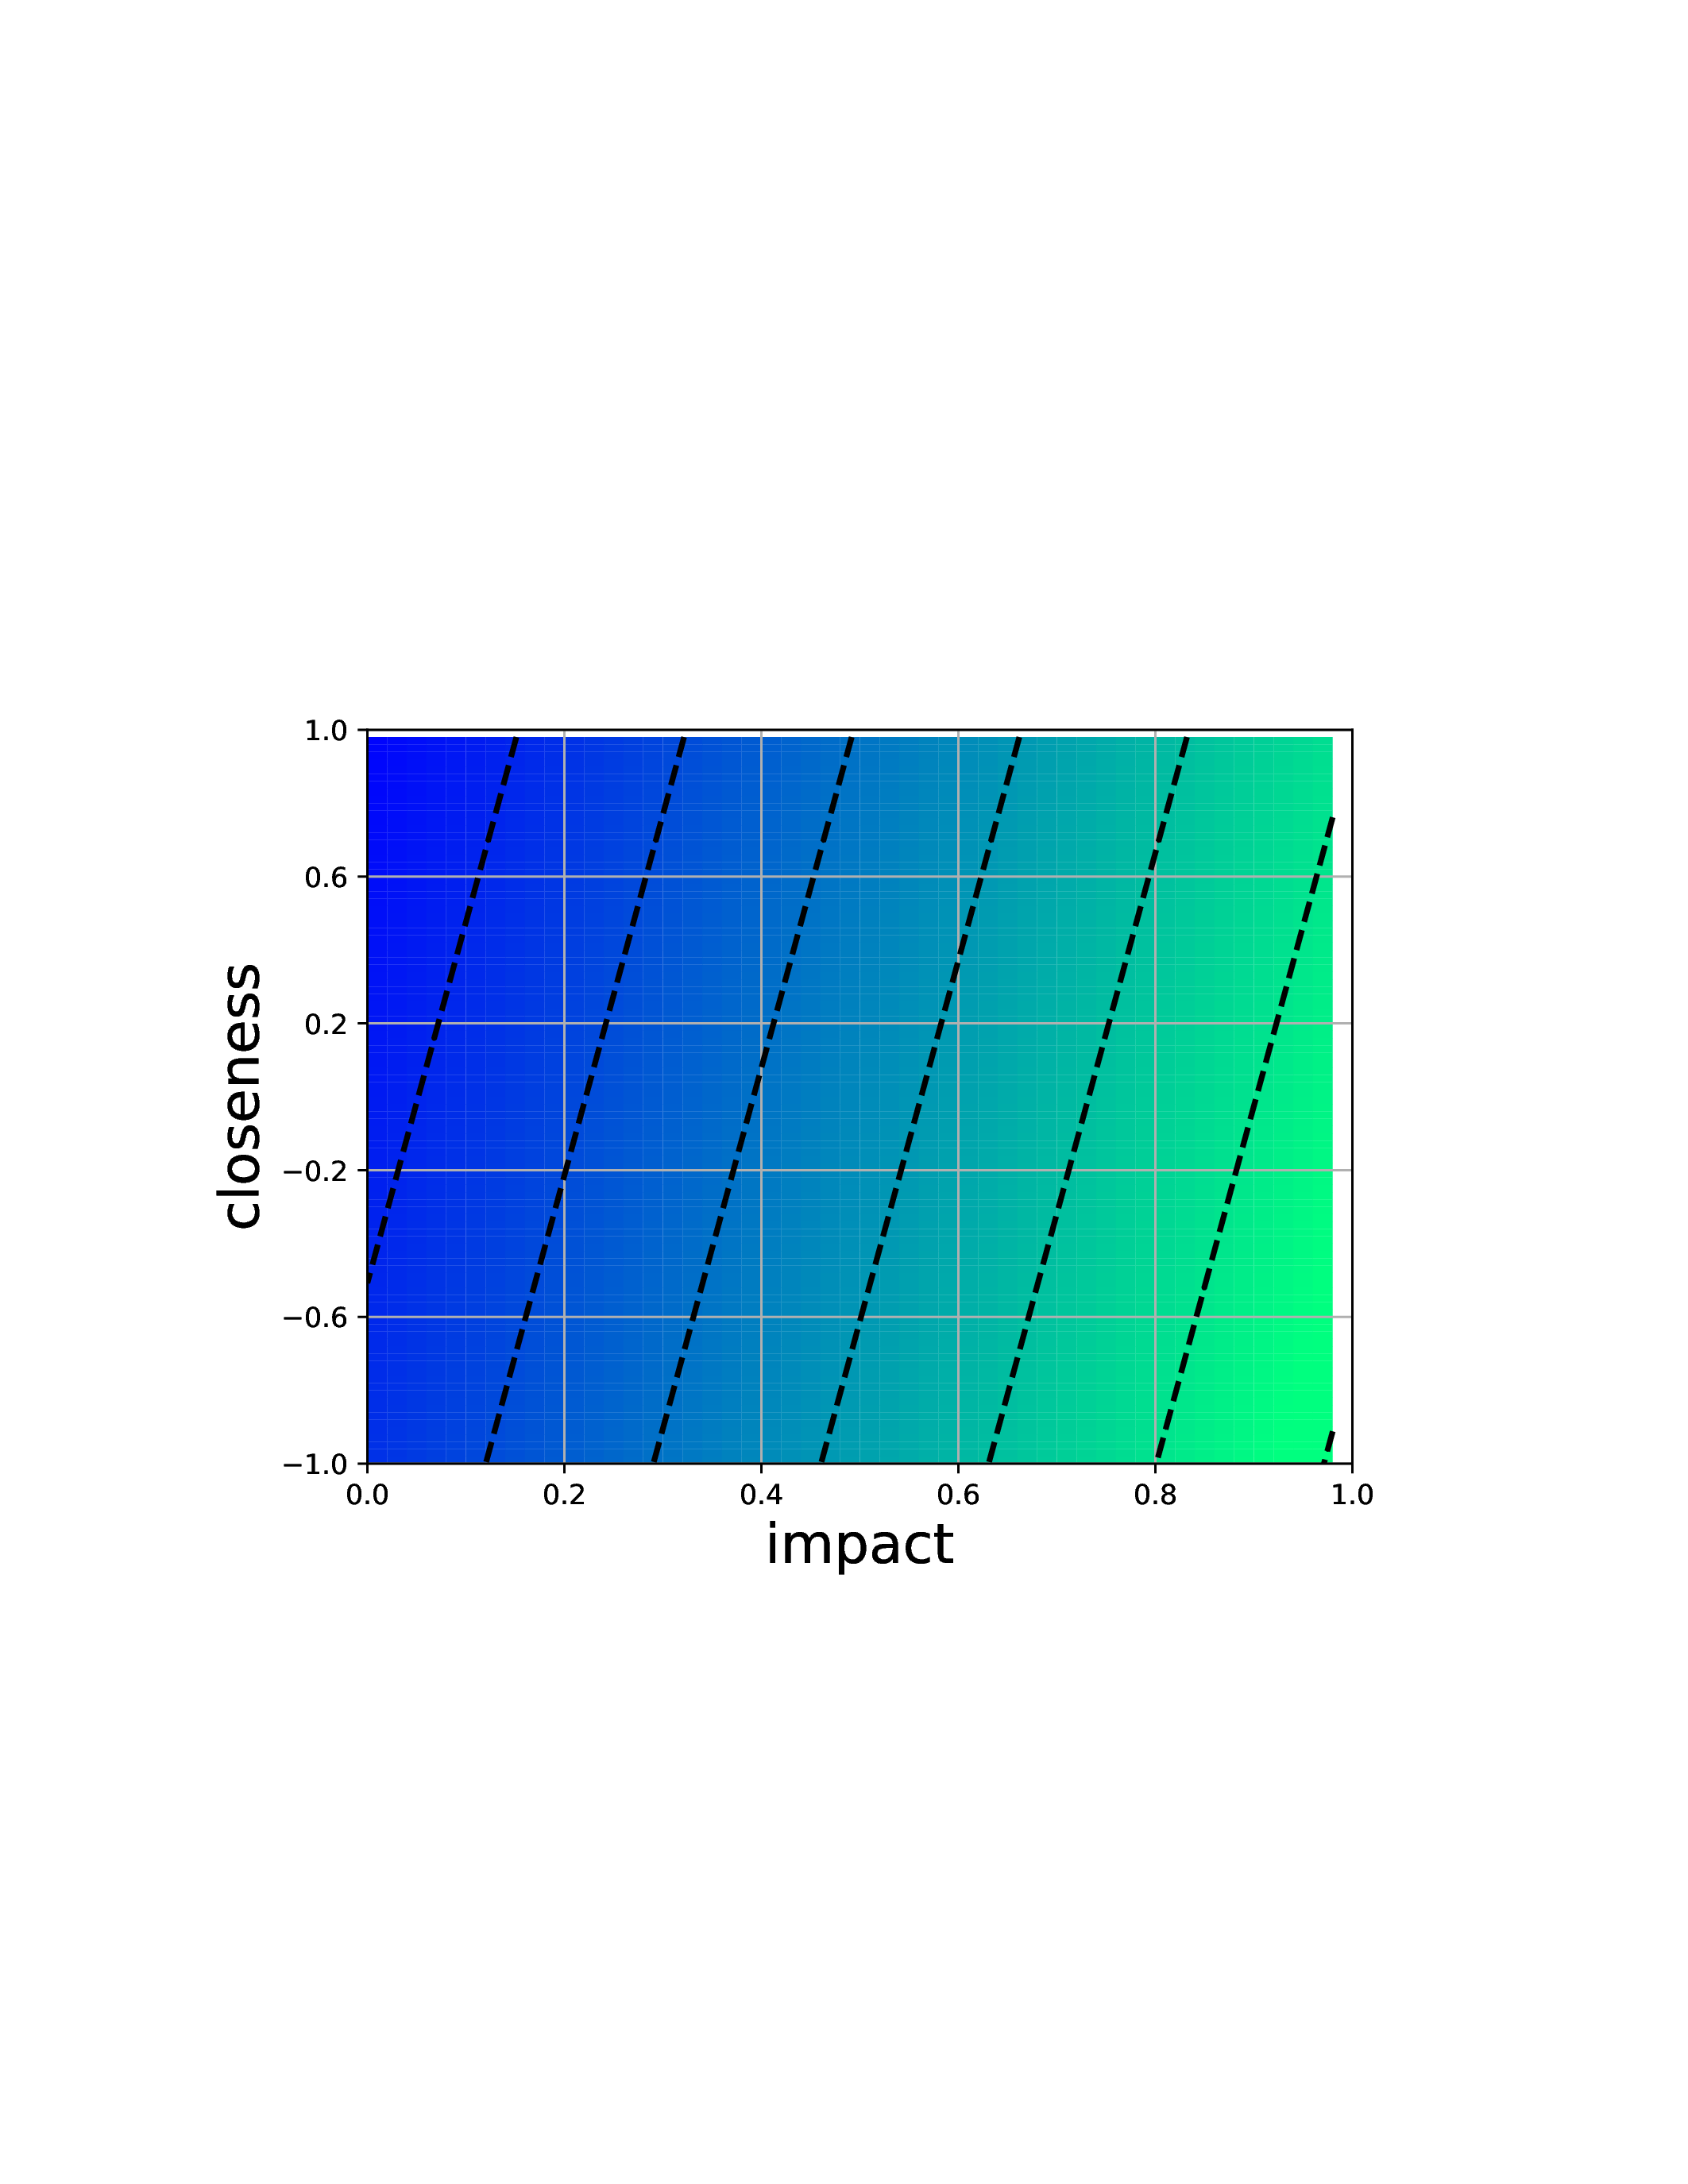}\label{fig:ML-2D-visualization-Impact-closeness-LinR}}
\caption{Visualization of the impact predictions of a (a) MLP regression model (with a neural network with 3 hidden layers of 32 nodes each, with ReLu activation functions) and (b) a Linear regression model, as a function of the two input features, namely, the measured impact (x-axis) and the (normalized in [0,1]) closeness of monitors to the victim (y-axis). Dark blue areas correspond to lower values, close to 0, and light green to higher values, close to 1.}
\label{fig:ML-2D-visualization-Impact-closeness}
\end{figure}

\section{Impact Estimation with the Naive Method}\label{appendix:naive-method}

See Fig.~\ref{fig:sims-impact-cdf-vs-hijack-types-relative-error}, Fig.~\ref{fig:sims-impact-cdf-vs-hijack-types-absolute-error}, Fig.~\ref{fig:sims-impact-cdfs},  Fig.~\ref{fig:sims-impact-scatter}, and Fig.~\ref{fig:RMSE-NIE-rnd-RC-RA-vs-nb-monitors}.

\begin{figure}[h]
\centering
\subfigure[RC]{\includegraphics[width=0.49\linewidth]{./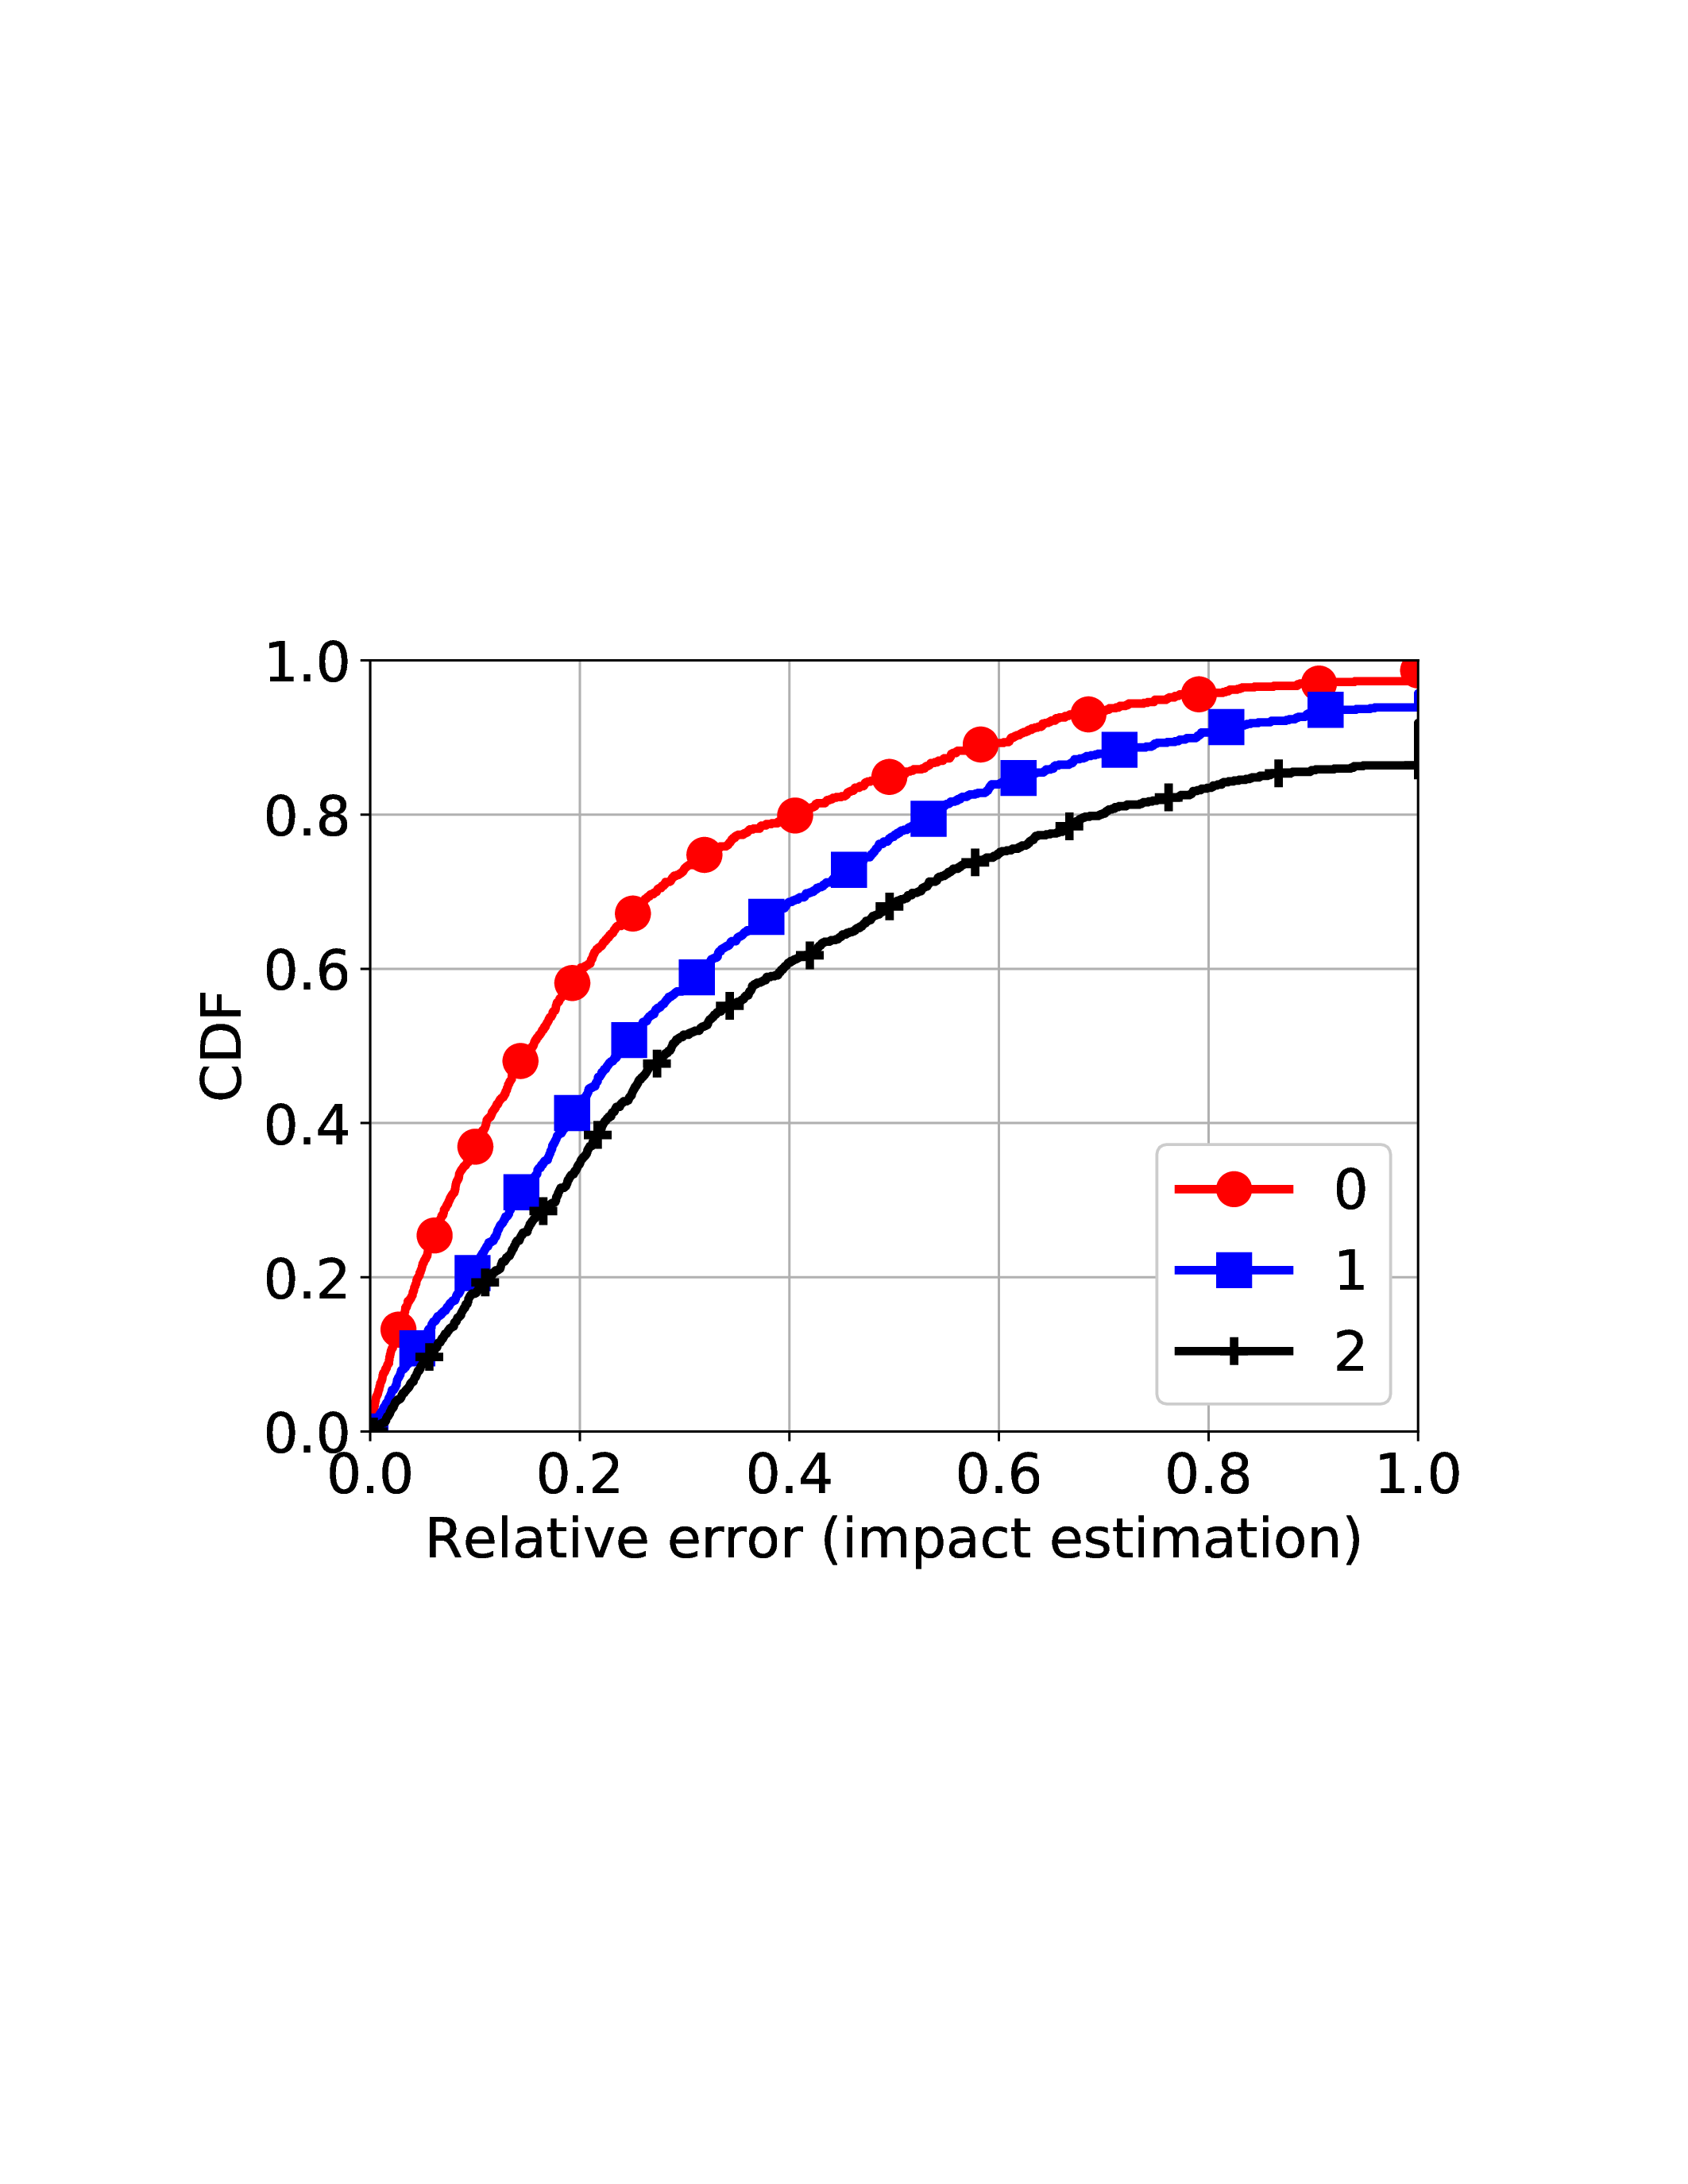}\label{fig:sims-impact-rc-vs-hijack-types-appendix}}
%\hspace{0.05\linewidth}
\subfigure[RA]{\includegraphics[width=0.49\linewidth]{./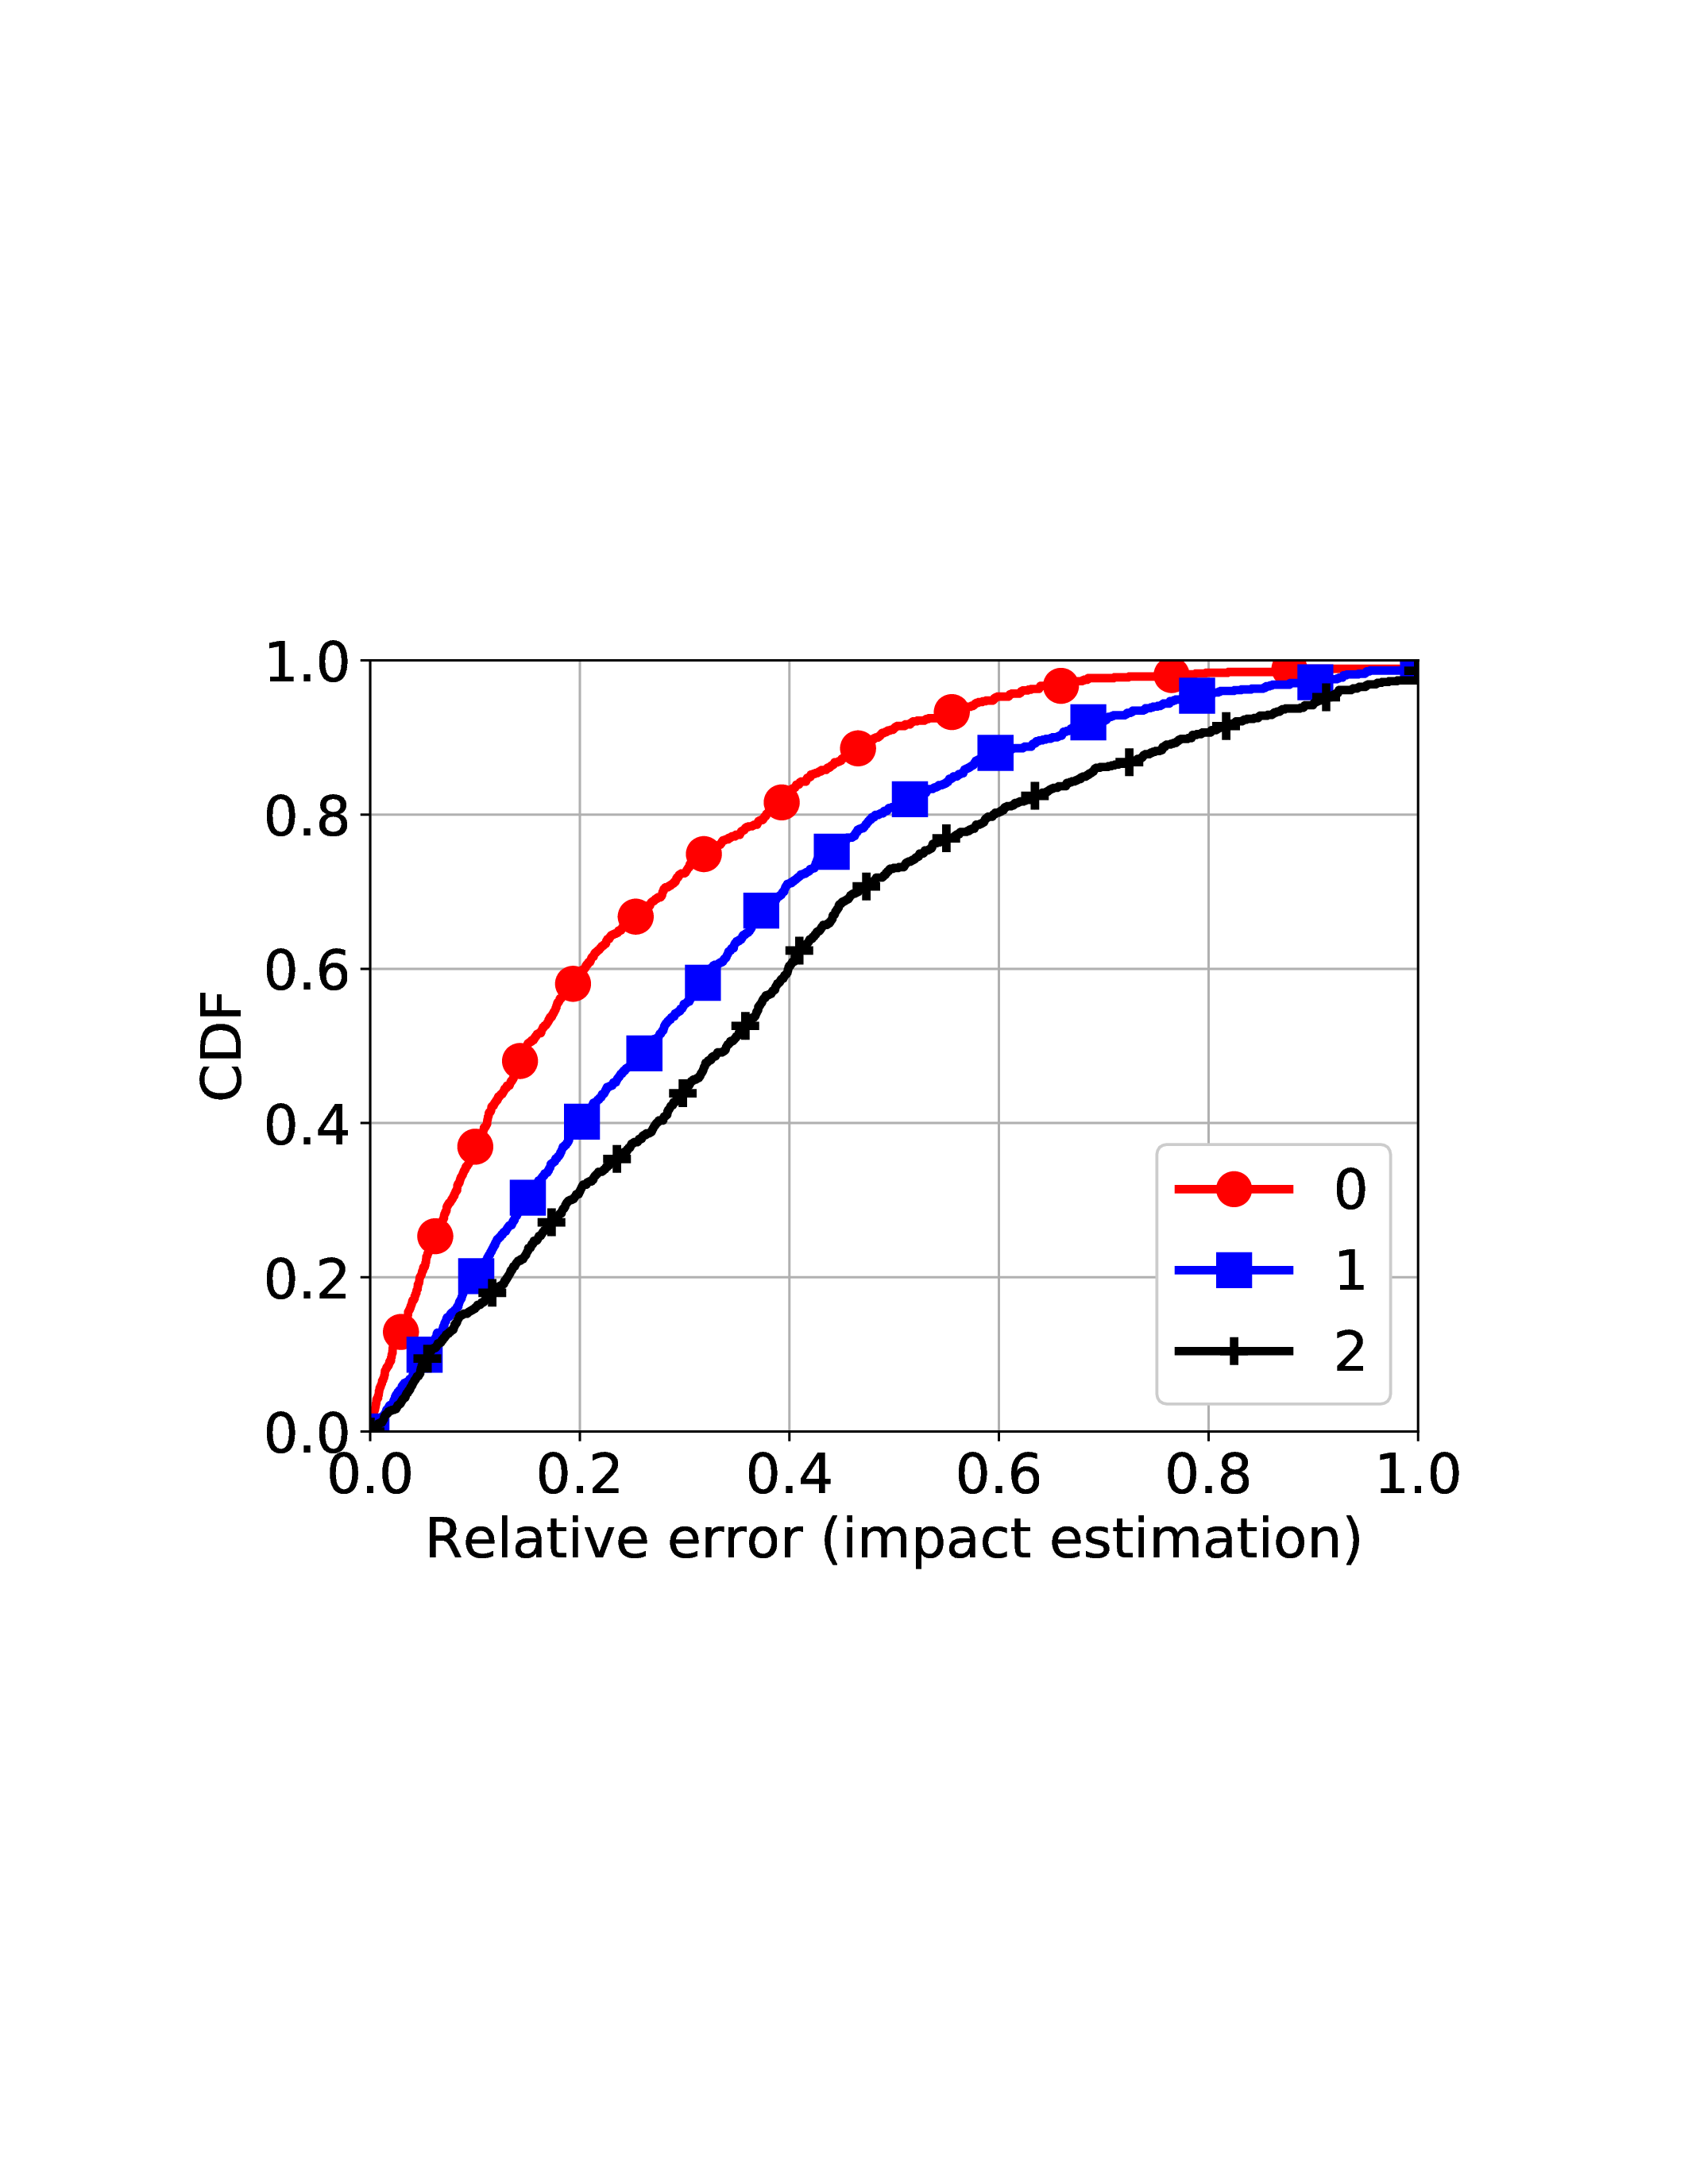}\label{fig:sims-impact-ra-vs-hijack-types-appendix}}
\caption{CDF of the relative error of impact estimated by measurements from (a) Route collectors and (b) RIPE Atlas probes, for hijacks of Types-0, 1, and 2. }
\label{fig:sims-impact-cdf-vs-hijack-types-relative-error}
\end{figure}

\begin{figure}[h]
\centering
\subfigure[RC]{\includegraphics[width=0.49\linewidth]{./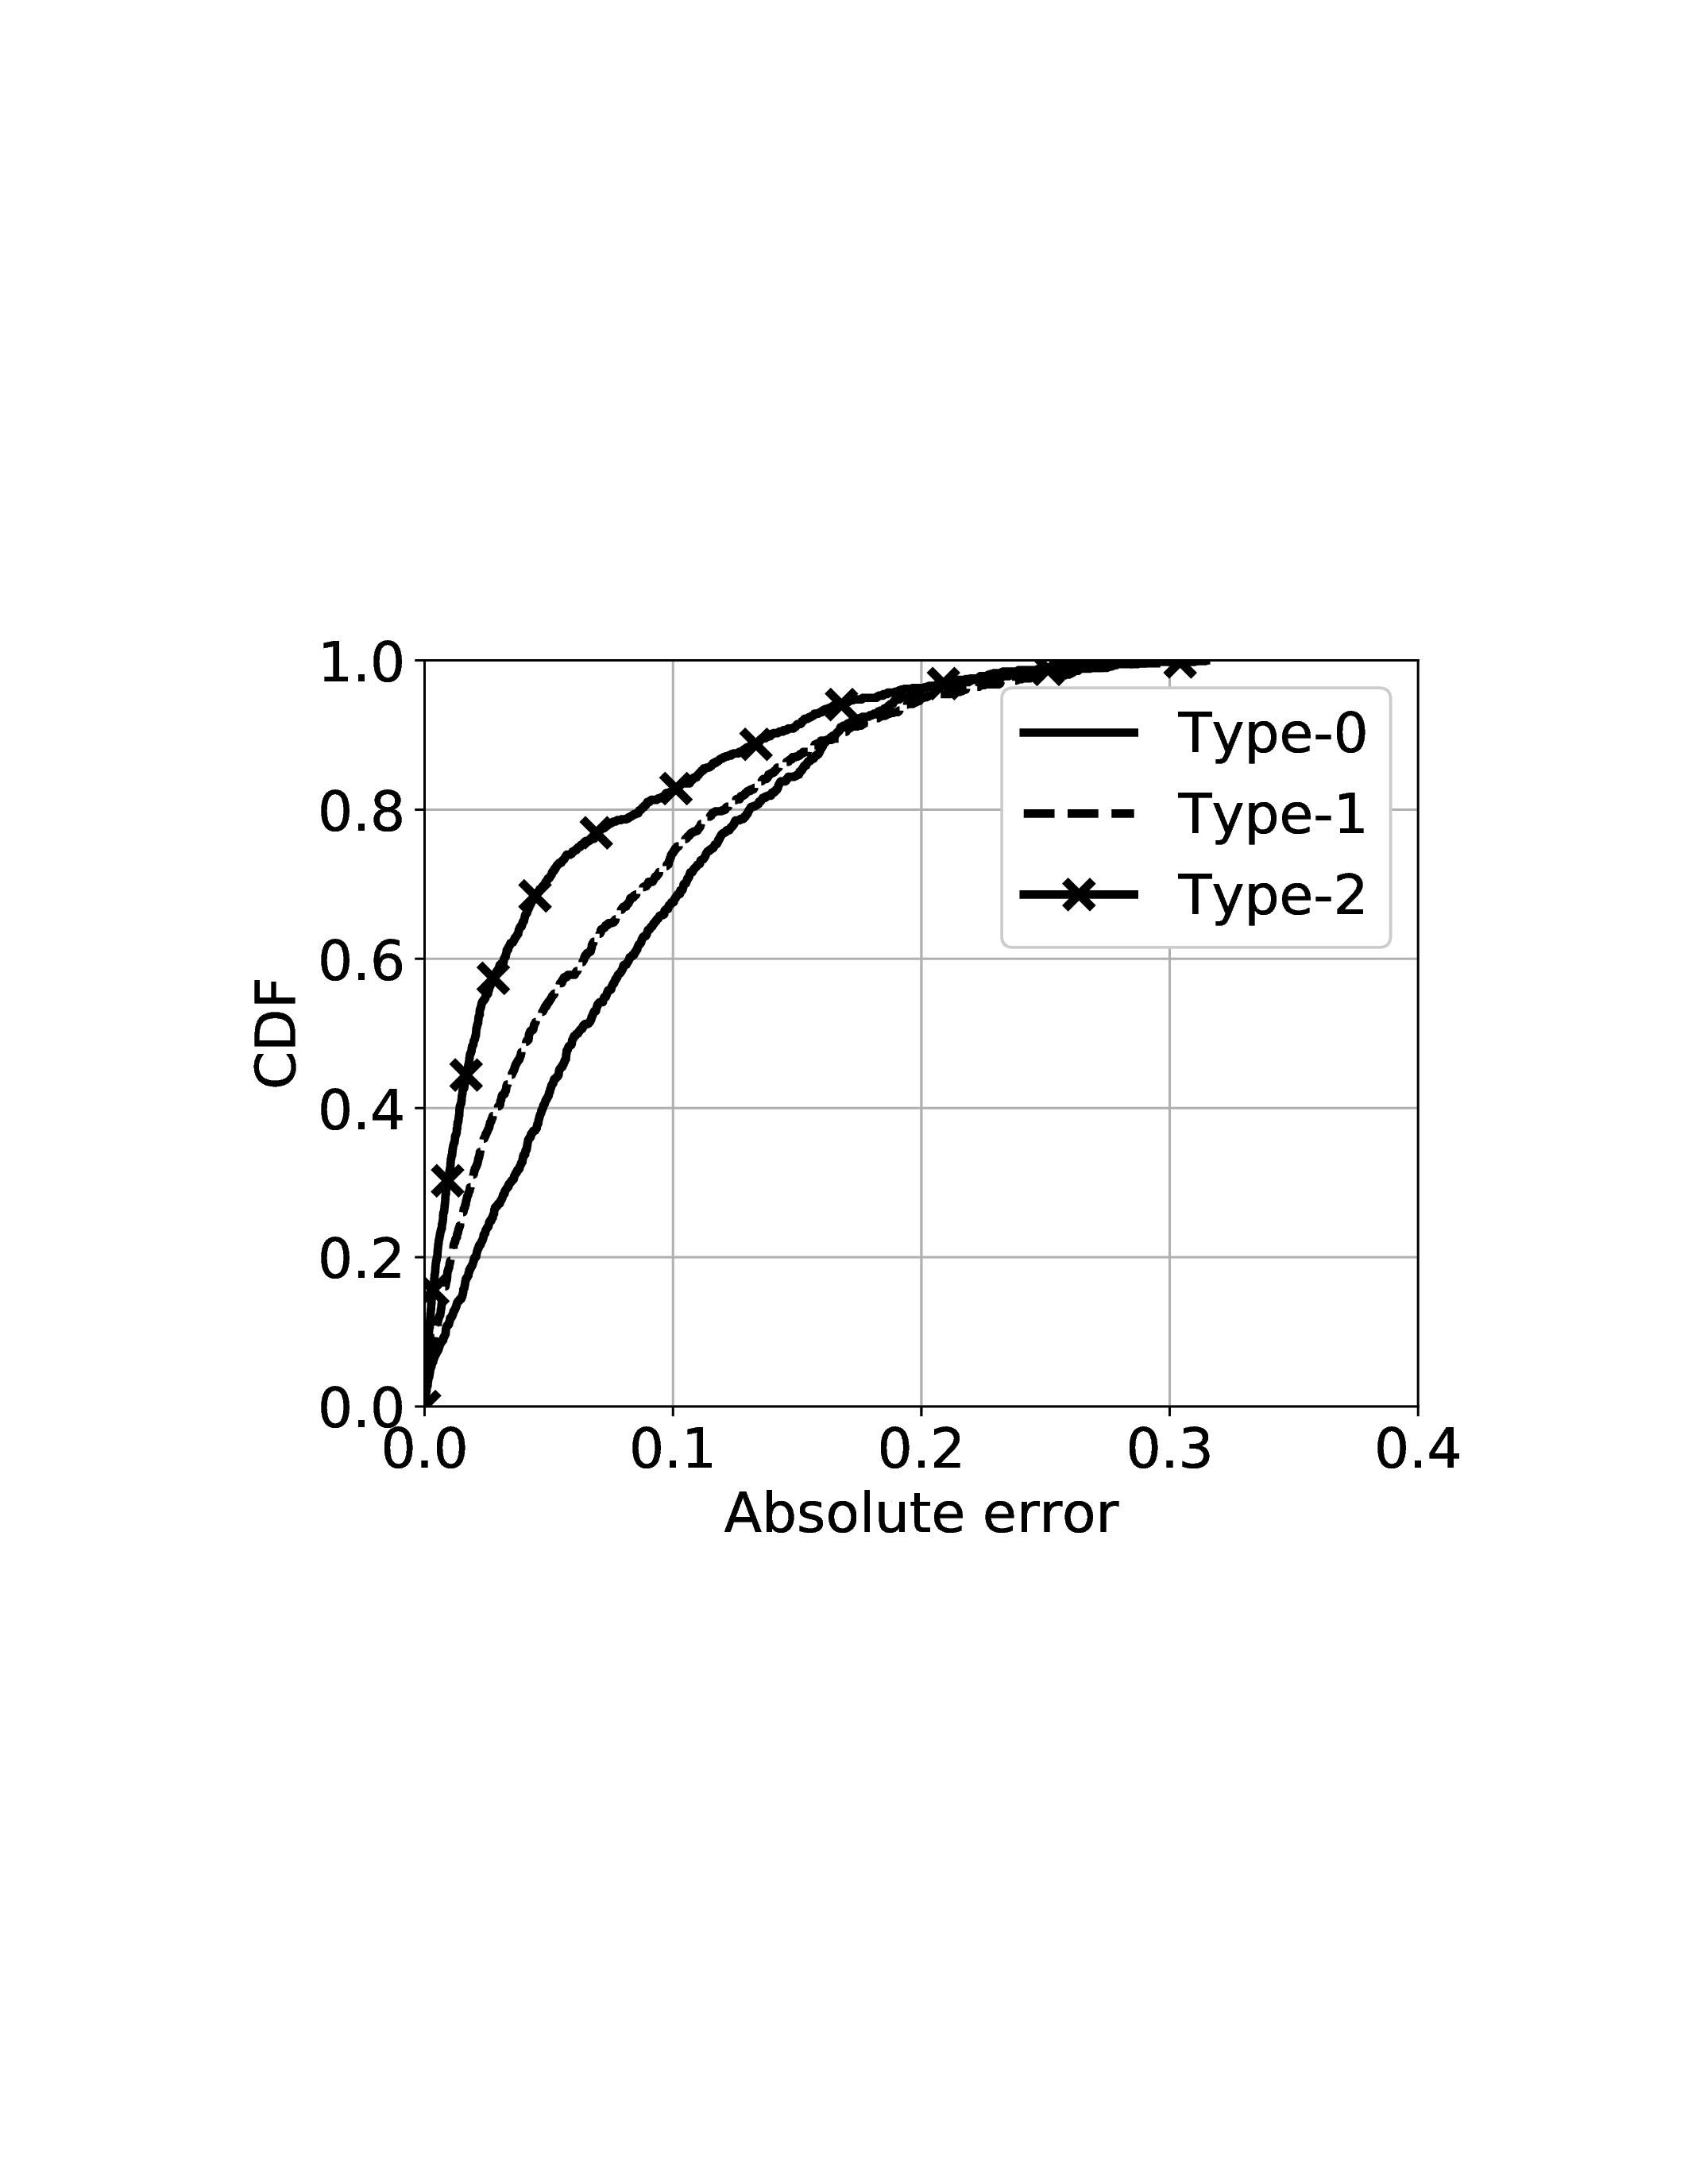}\label{fig:sims-impact-rc-vs-hijack-types--absolute-error-appendix}}
%\hspace{0.05\linewidth}
\subfigure[RA]{\includegraphics[width=0.49\linewidth]{./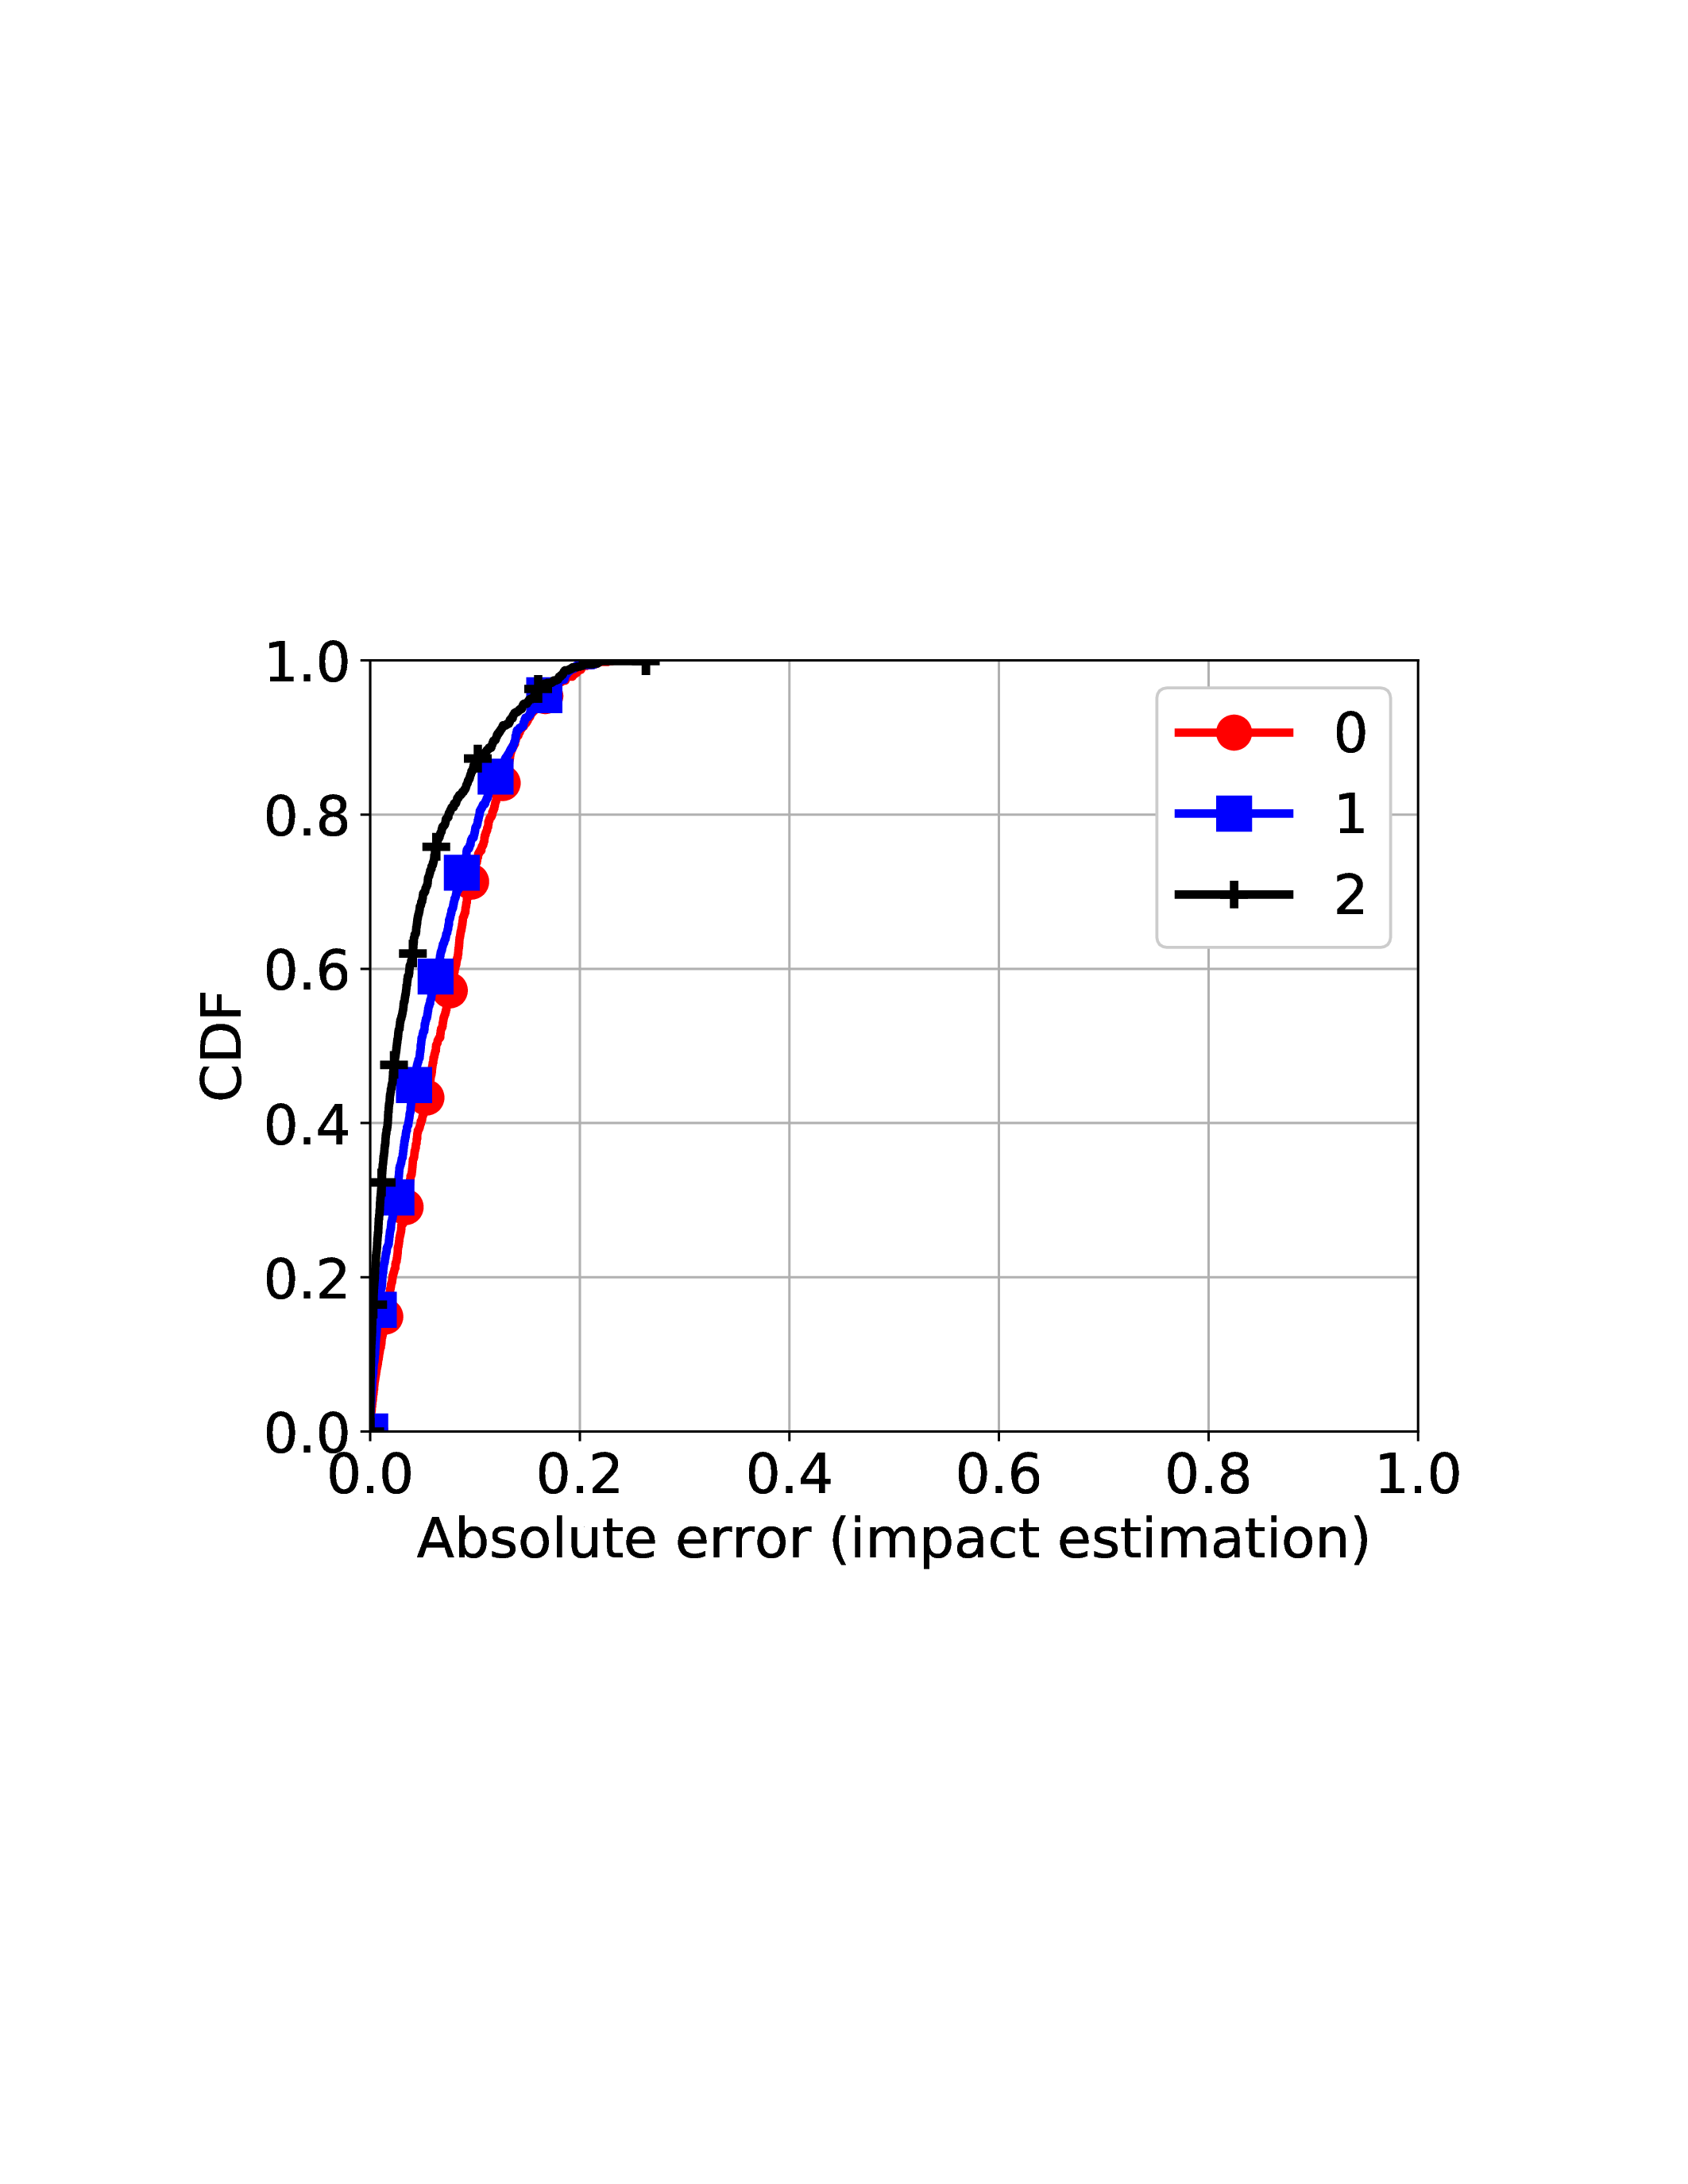}\label{fig:sims-impact-ra-vs-hijack-types-absolute-error-appendix}}
\caption{CDF of the absolute error of impact estimated by measurements from (a) Route collectors and (b) RIPE Atlas probes, for hijacks of Types-0, 1, and 2.}
\label{fig:sims-impact-cdf-vs-hijack-types-absolute-error}
\end{figure}

\begin{figure*}
\centering
\subfigure[Hijack Type-0]{\includegraphics[width=0.33\linewidth]{./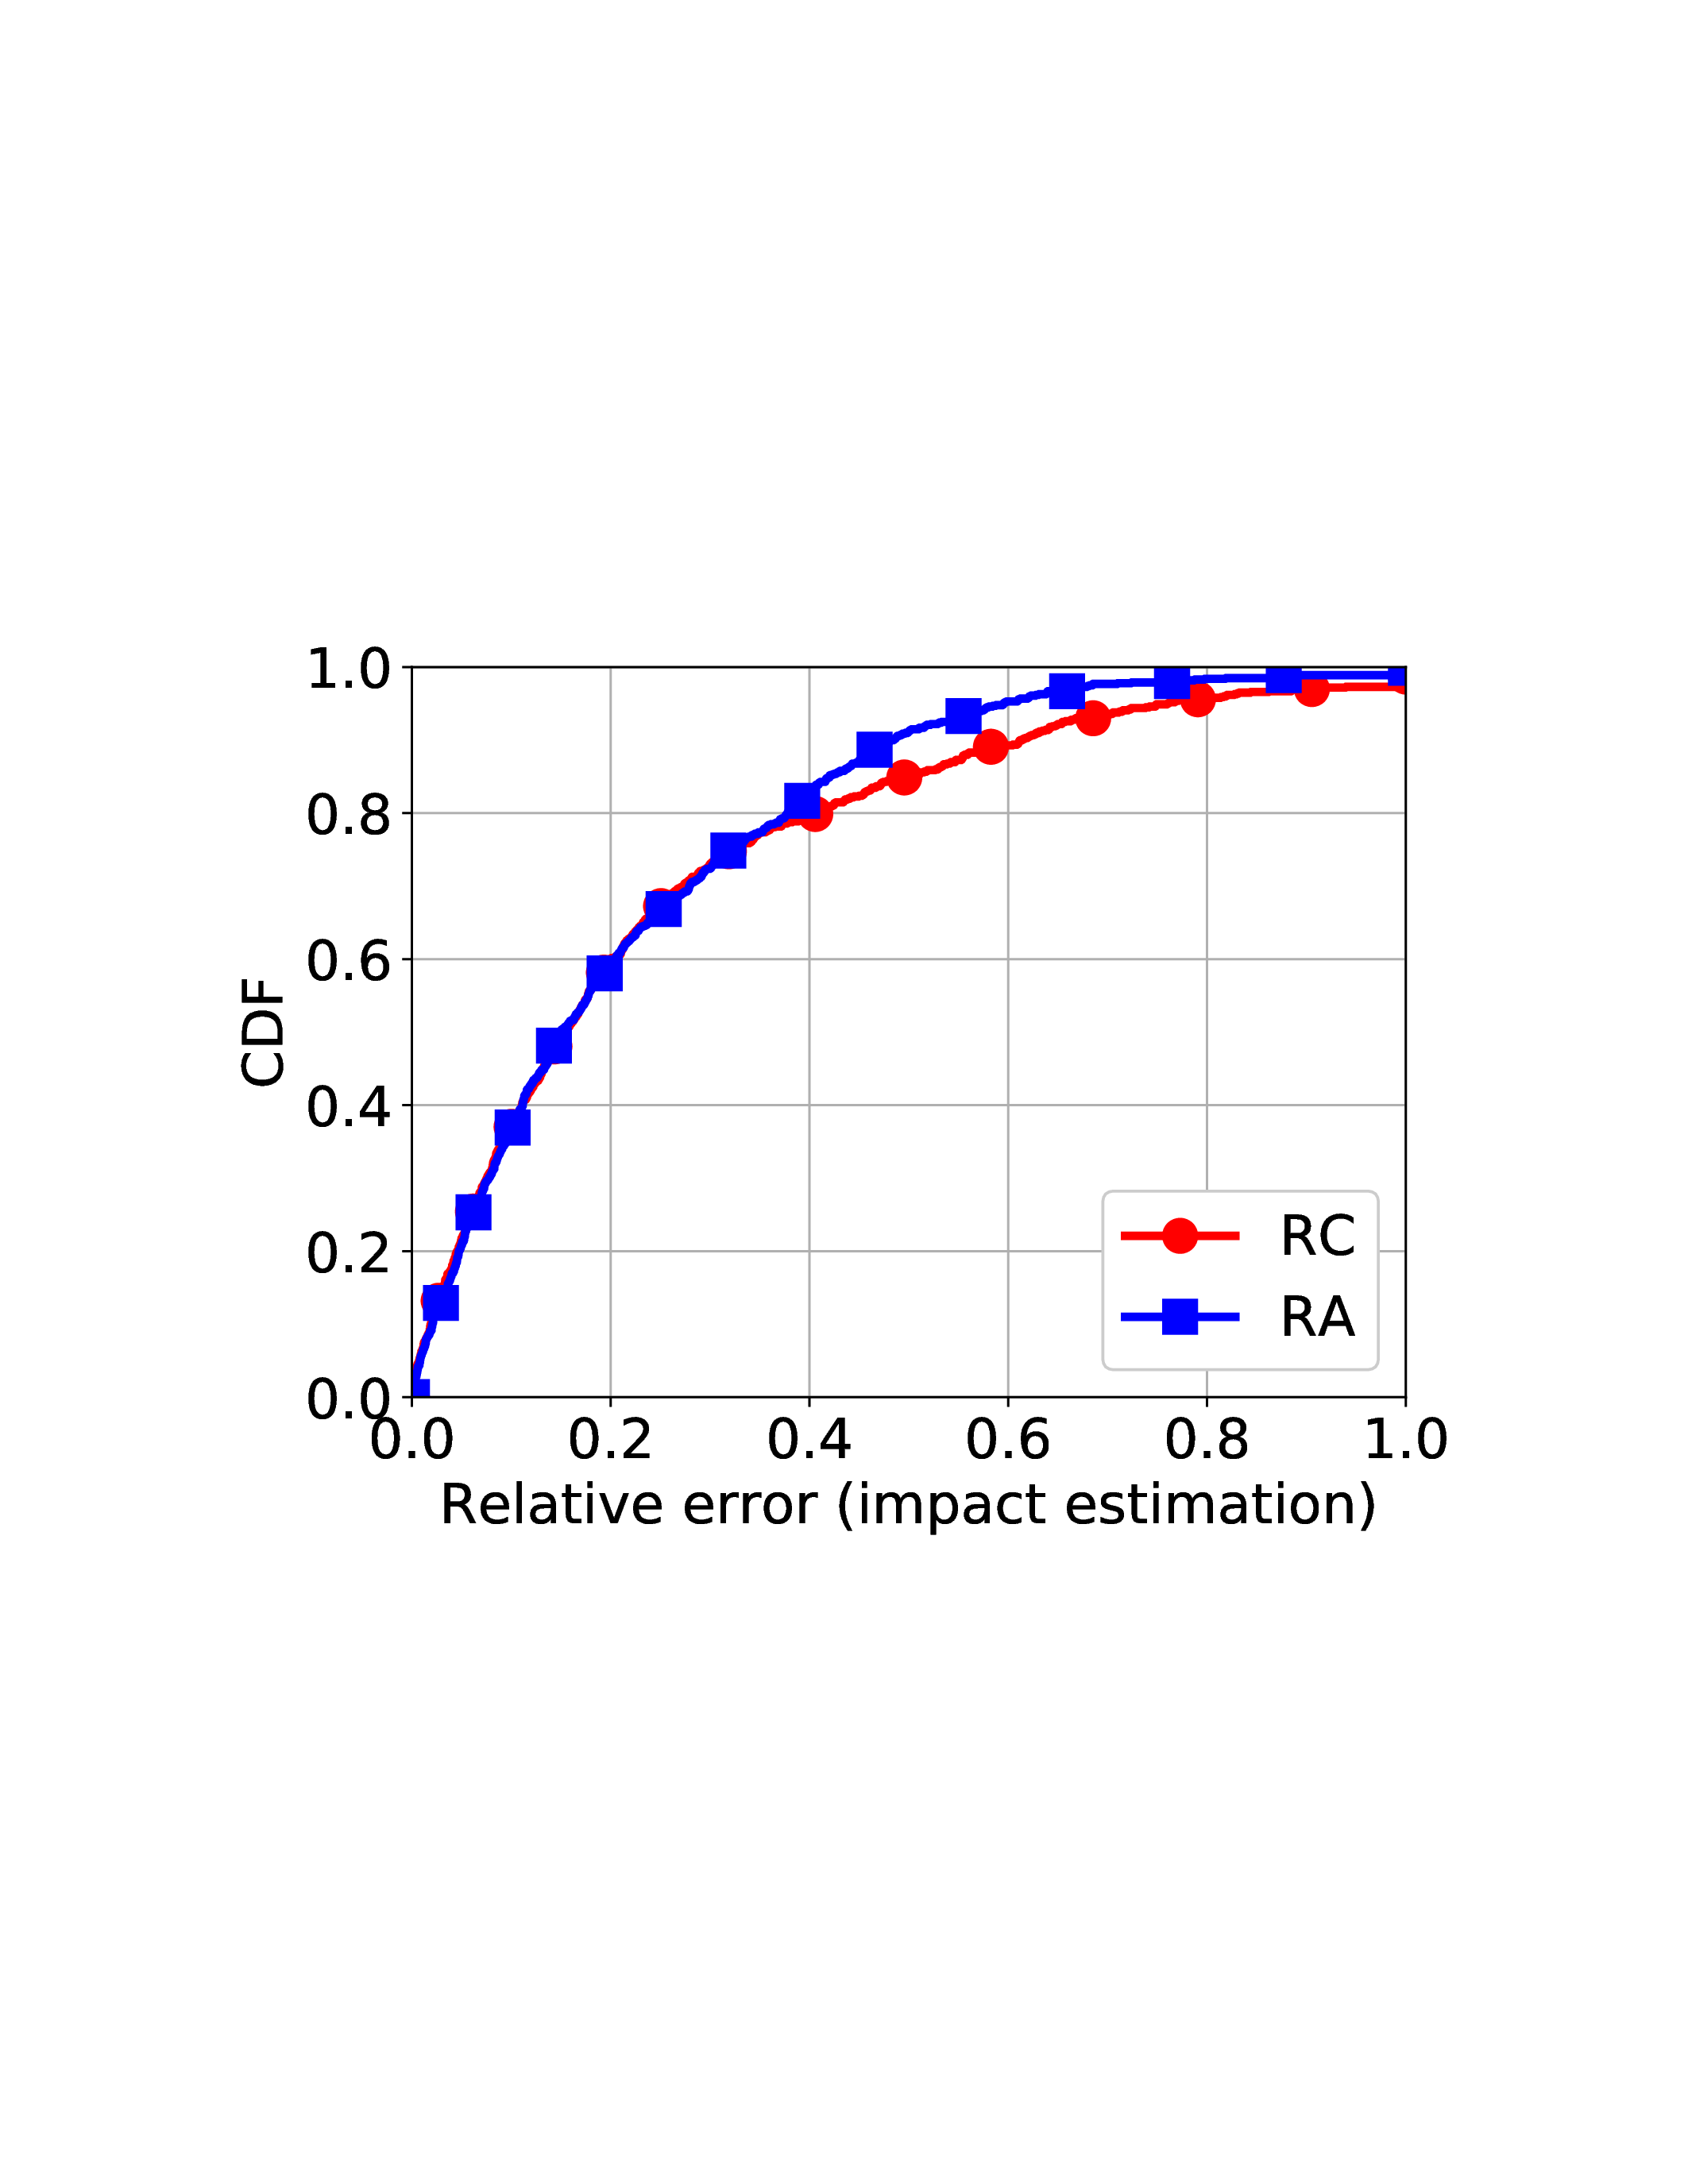}\label{fig:sims-impact-rc-vs-ra-hijack-type-0}}
\subfigure[Hijack Type-1]{\includegraphics[width=0.33\linewidth]{./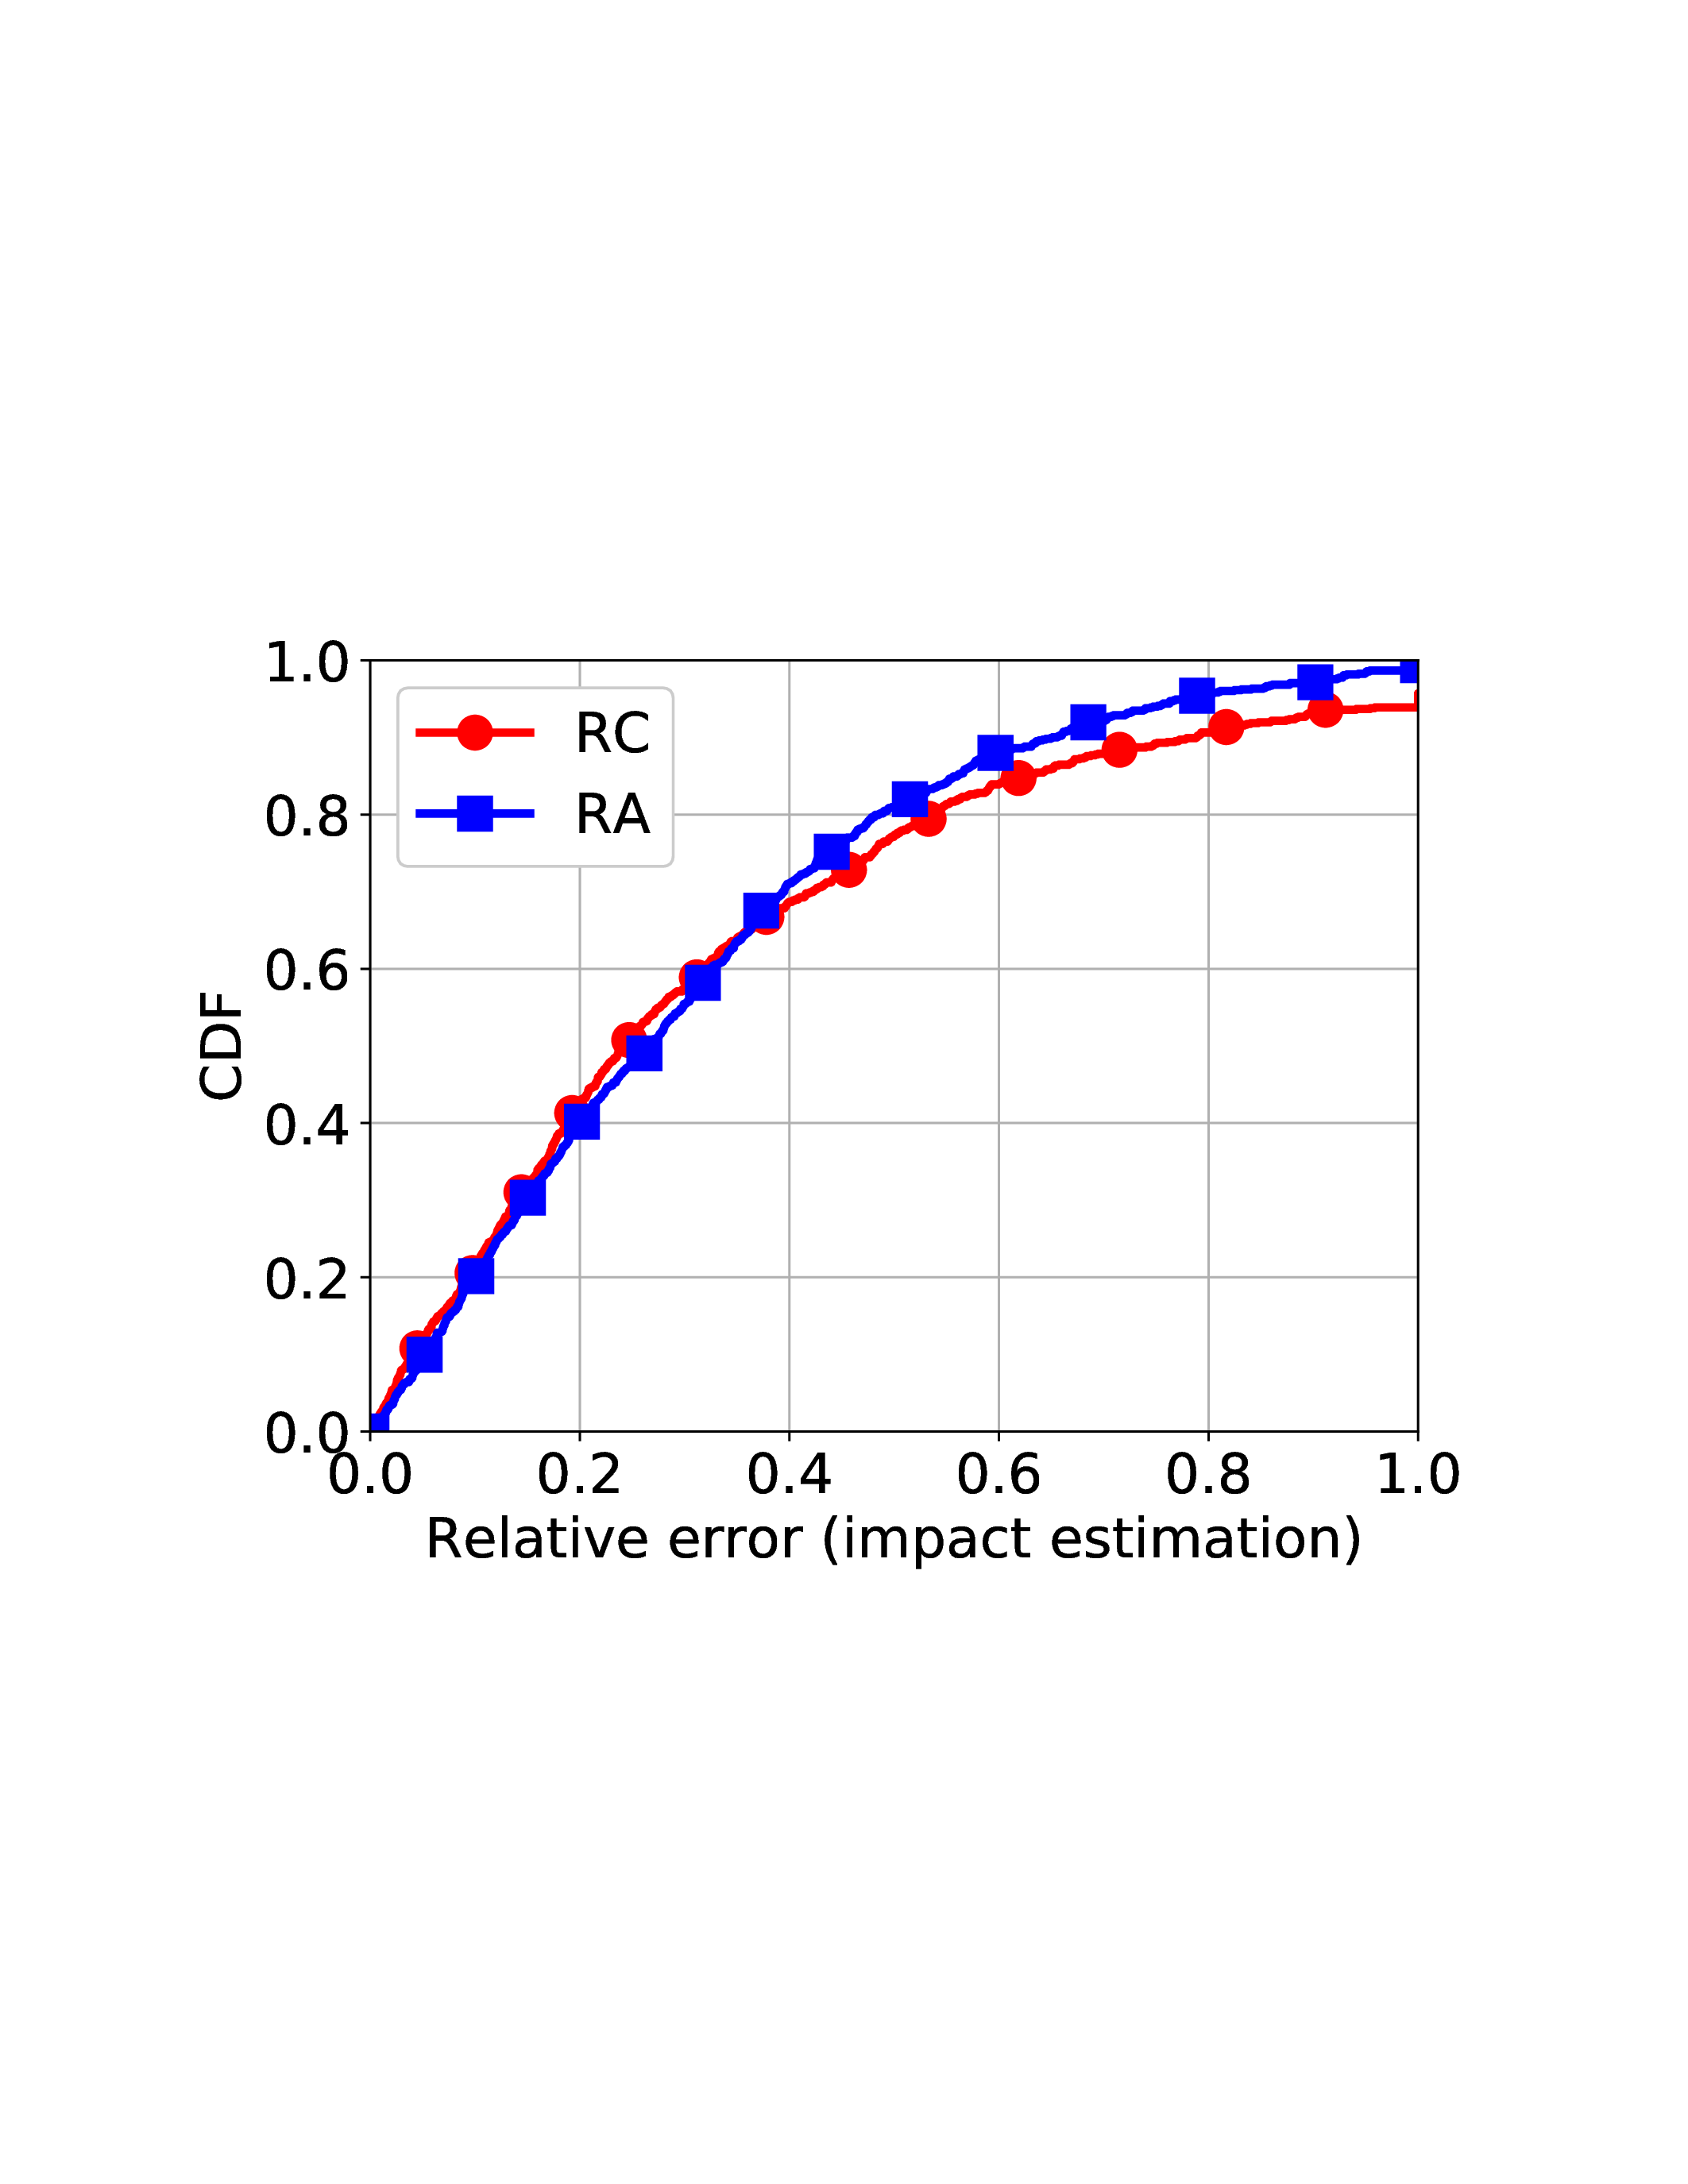}\label{fig:sims-impact-rc-vs-ra-hijack-type-1}}
\subfigure[Hijack Type-2]{\includegraphics[width=0.33\linewidth]{./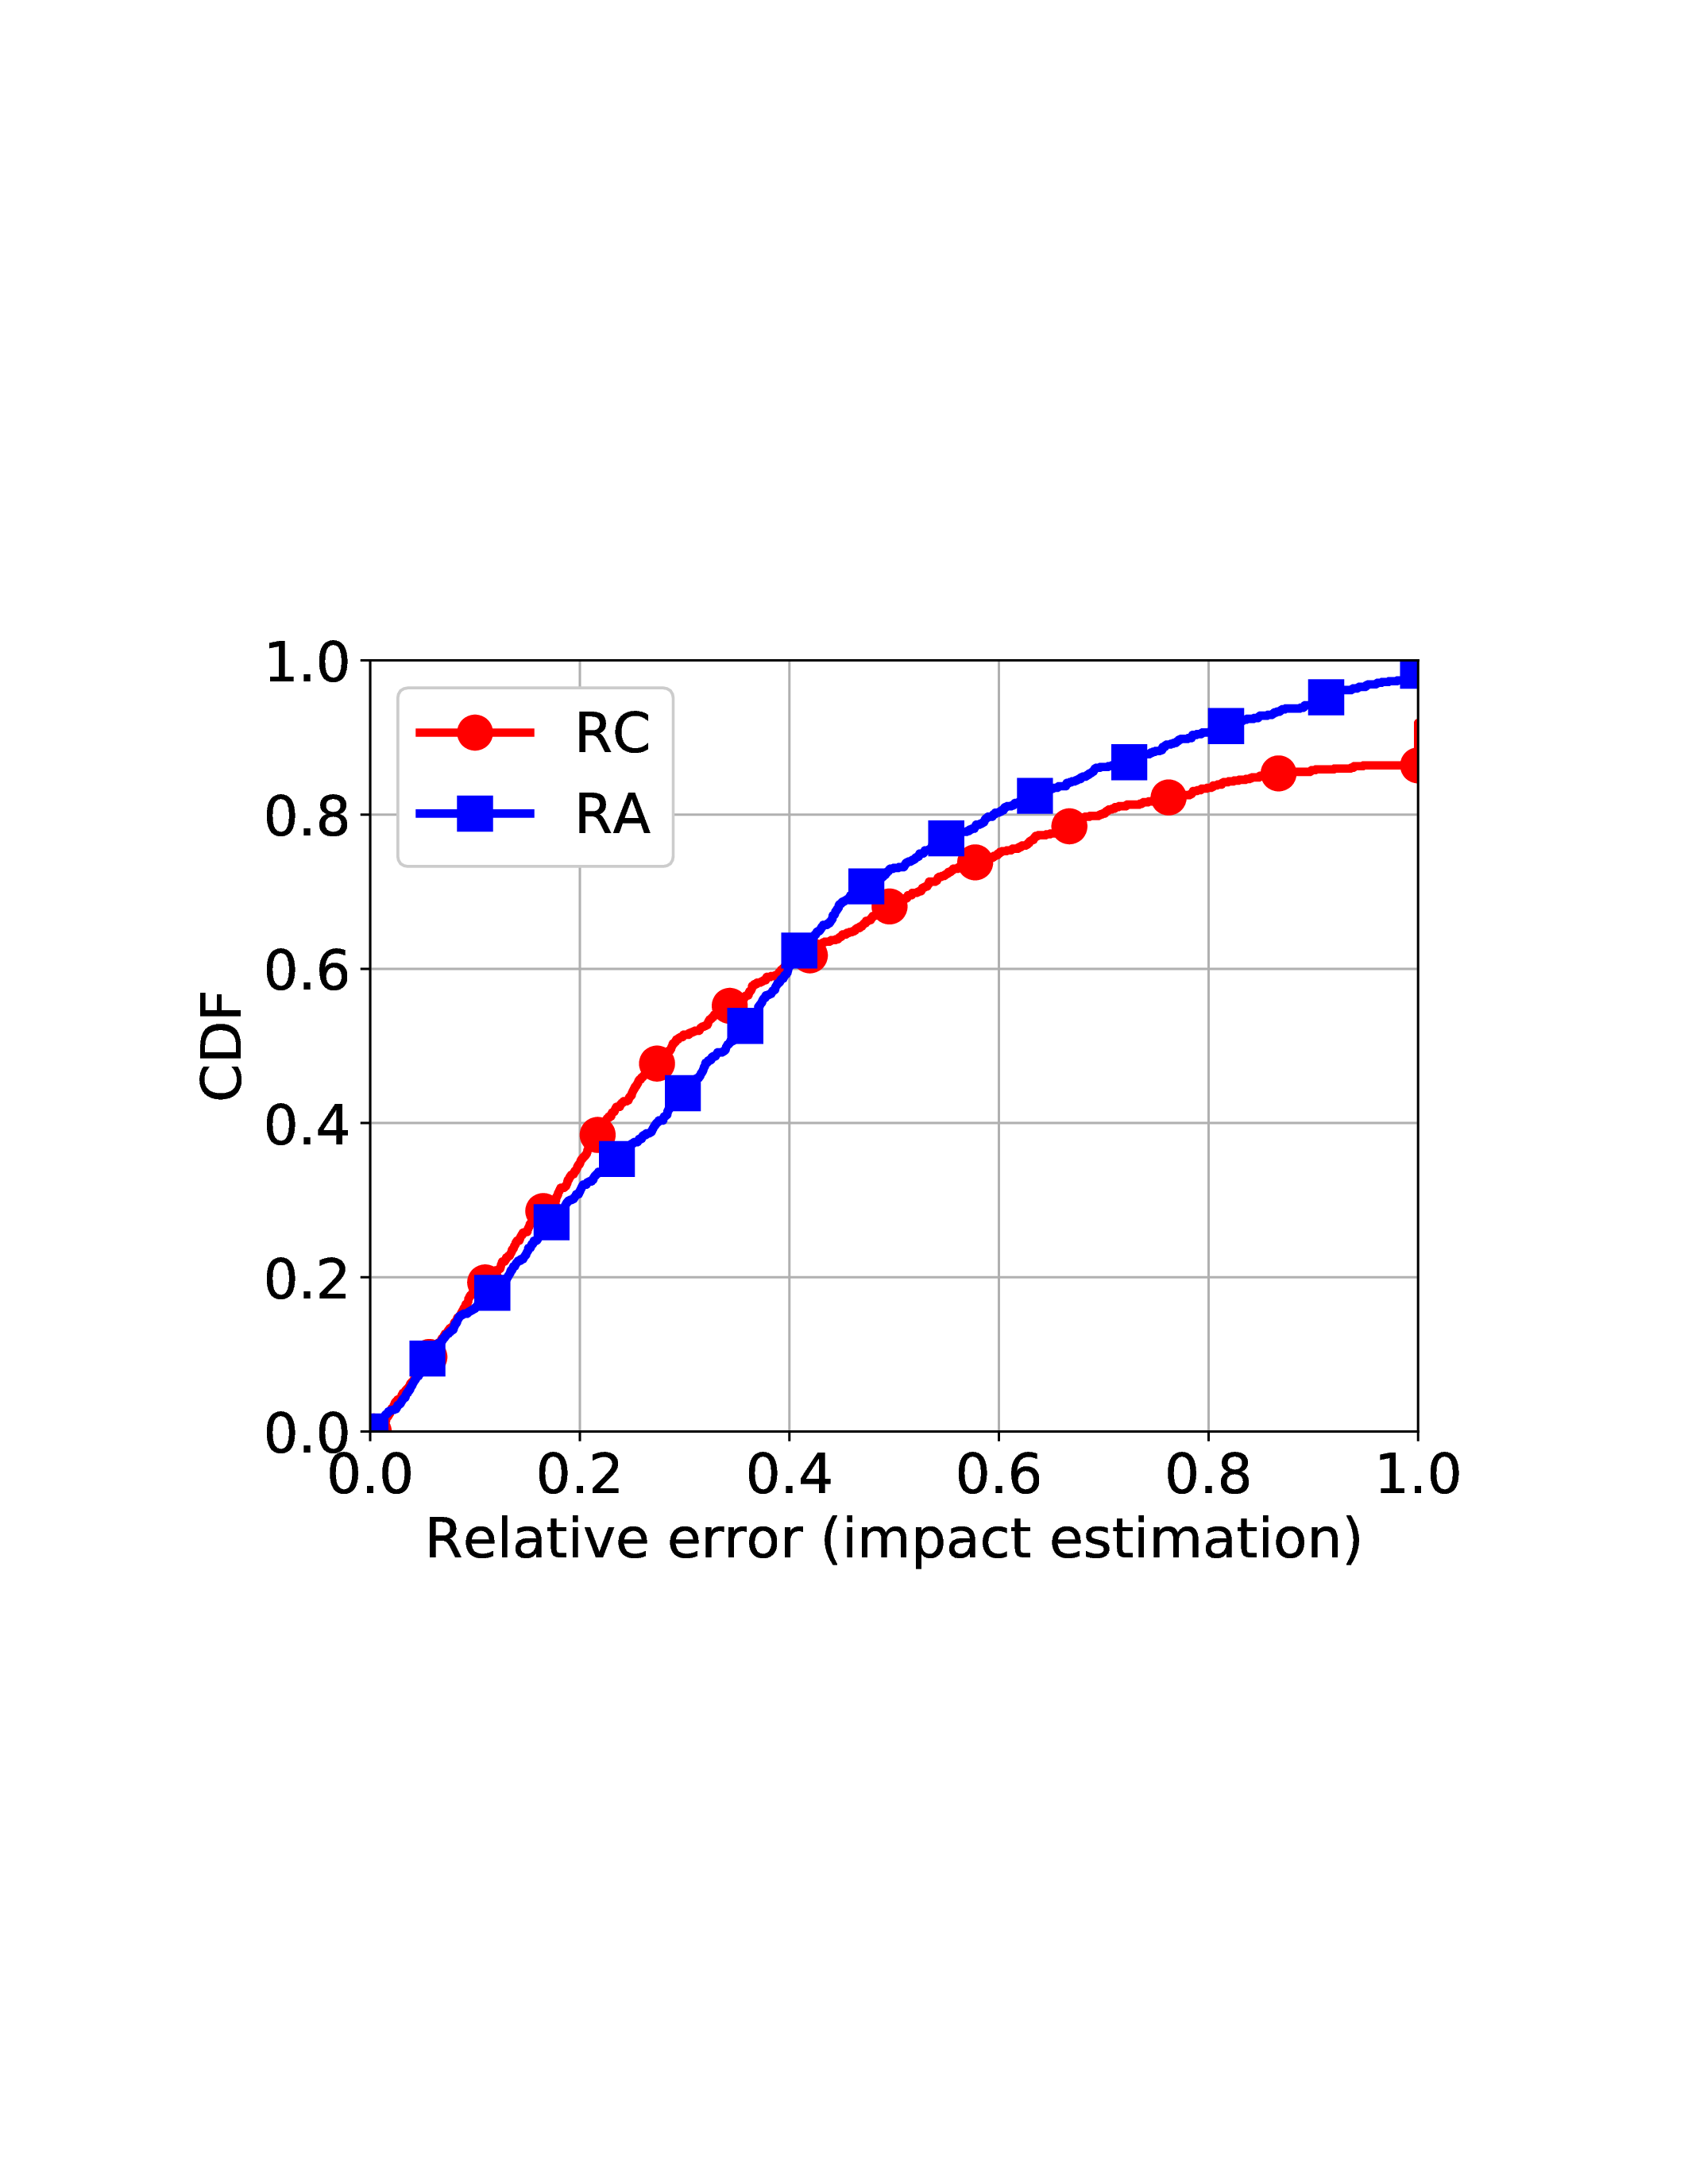}\label{fig:sims-impact-rc-vs-ra-hijack-type-2}}
\subfigure[Hijack Type-0]{\includegraphics[width=0.33\linewidth]{./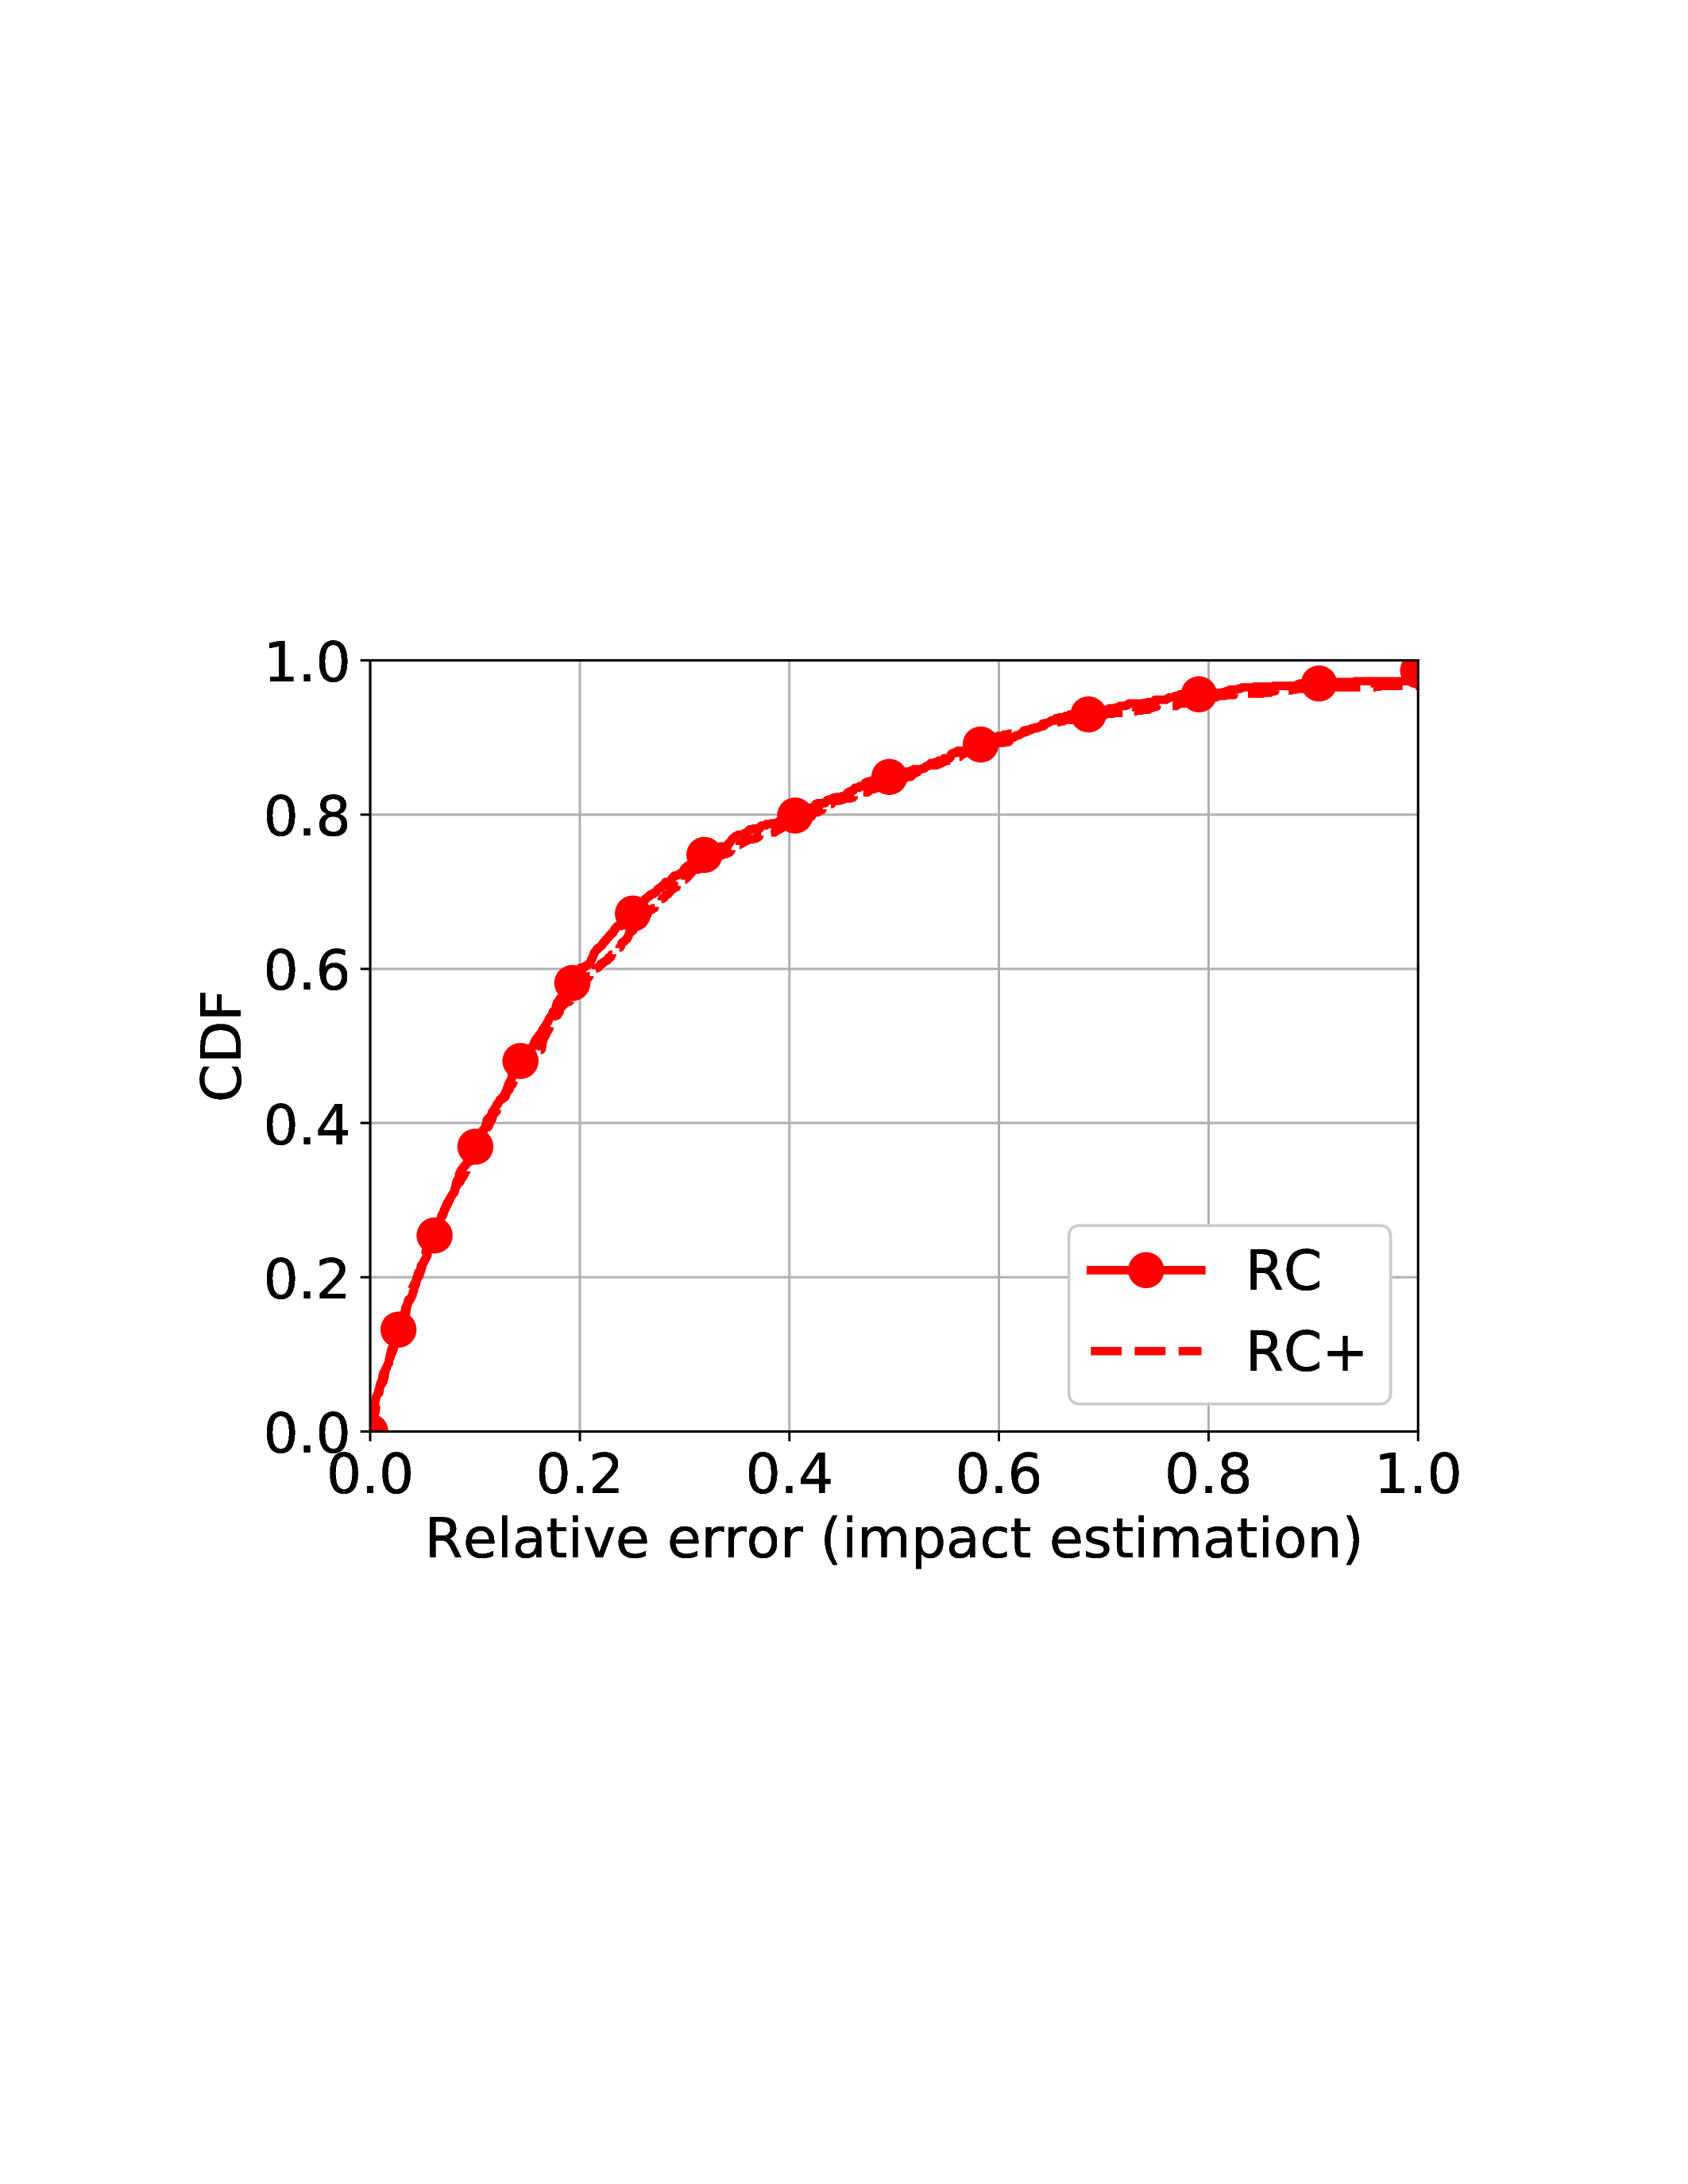}\label{fig:sims-impact-rc-vs-rc+-hijack-type-0}}
\subfigure[Hijack Type-1]{\includegraphics[width=0.33\linewidth]{./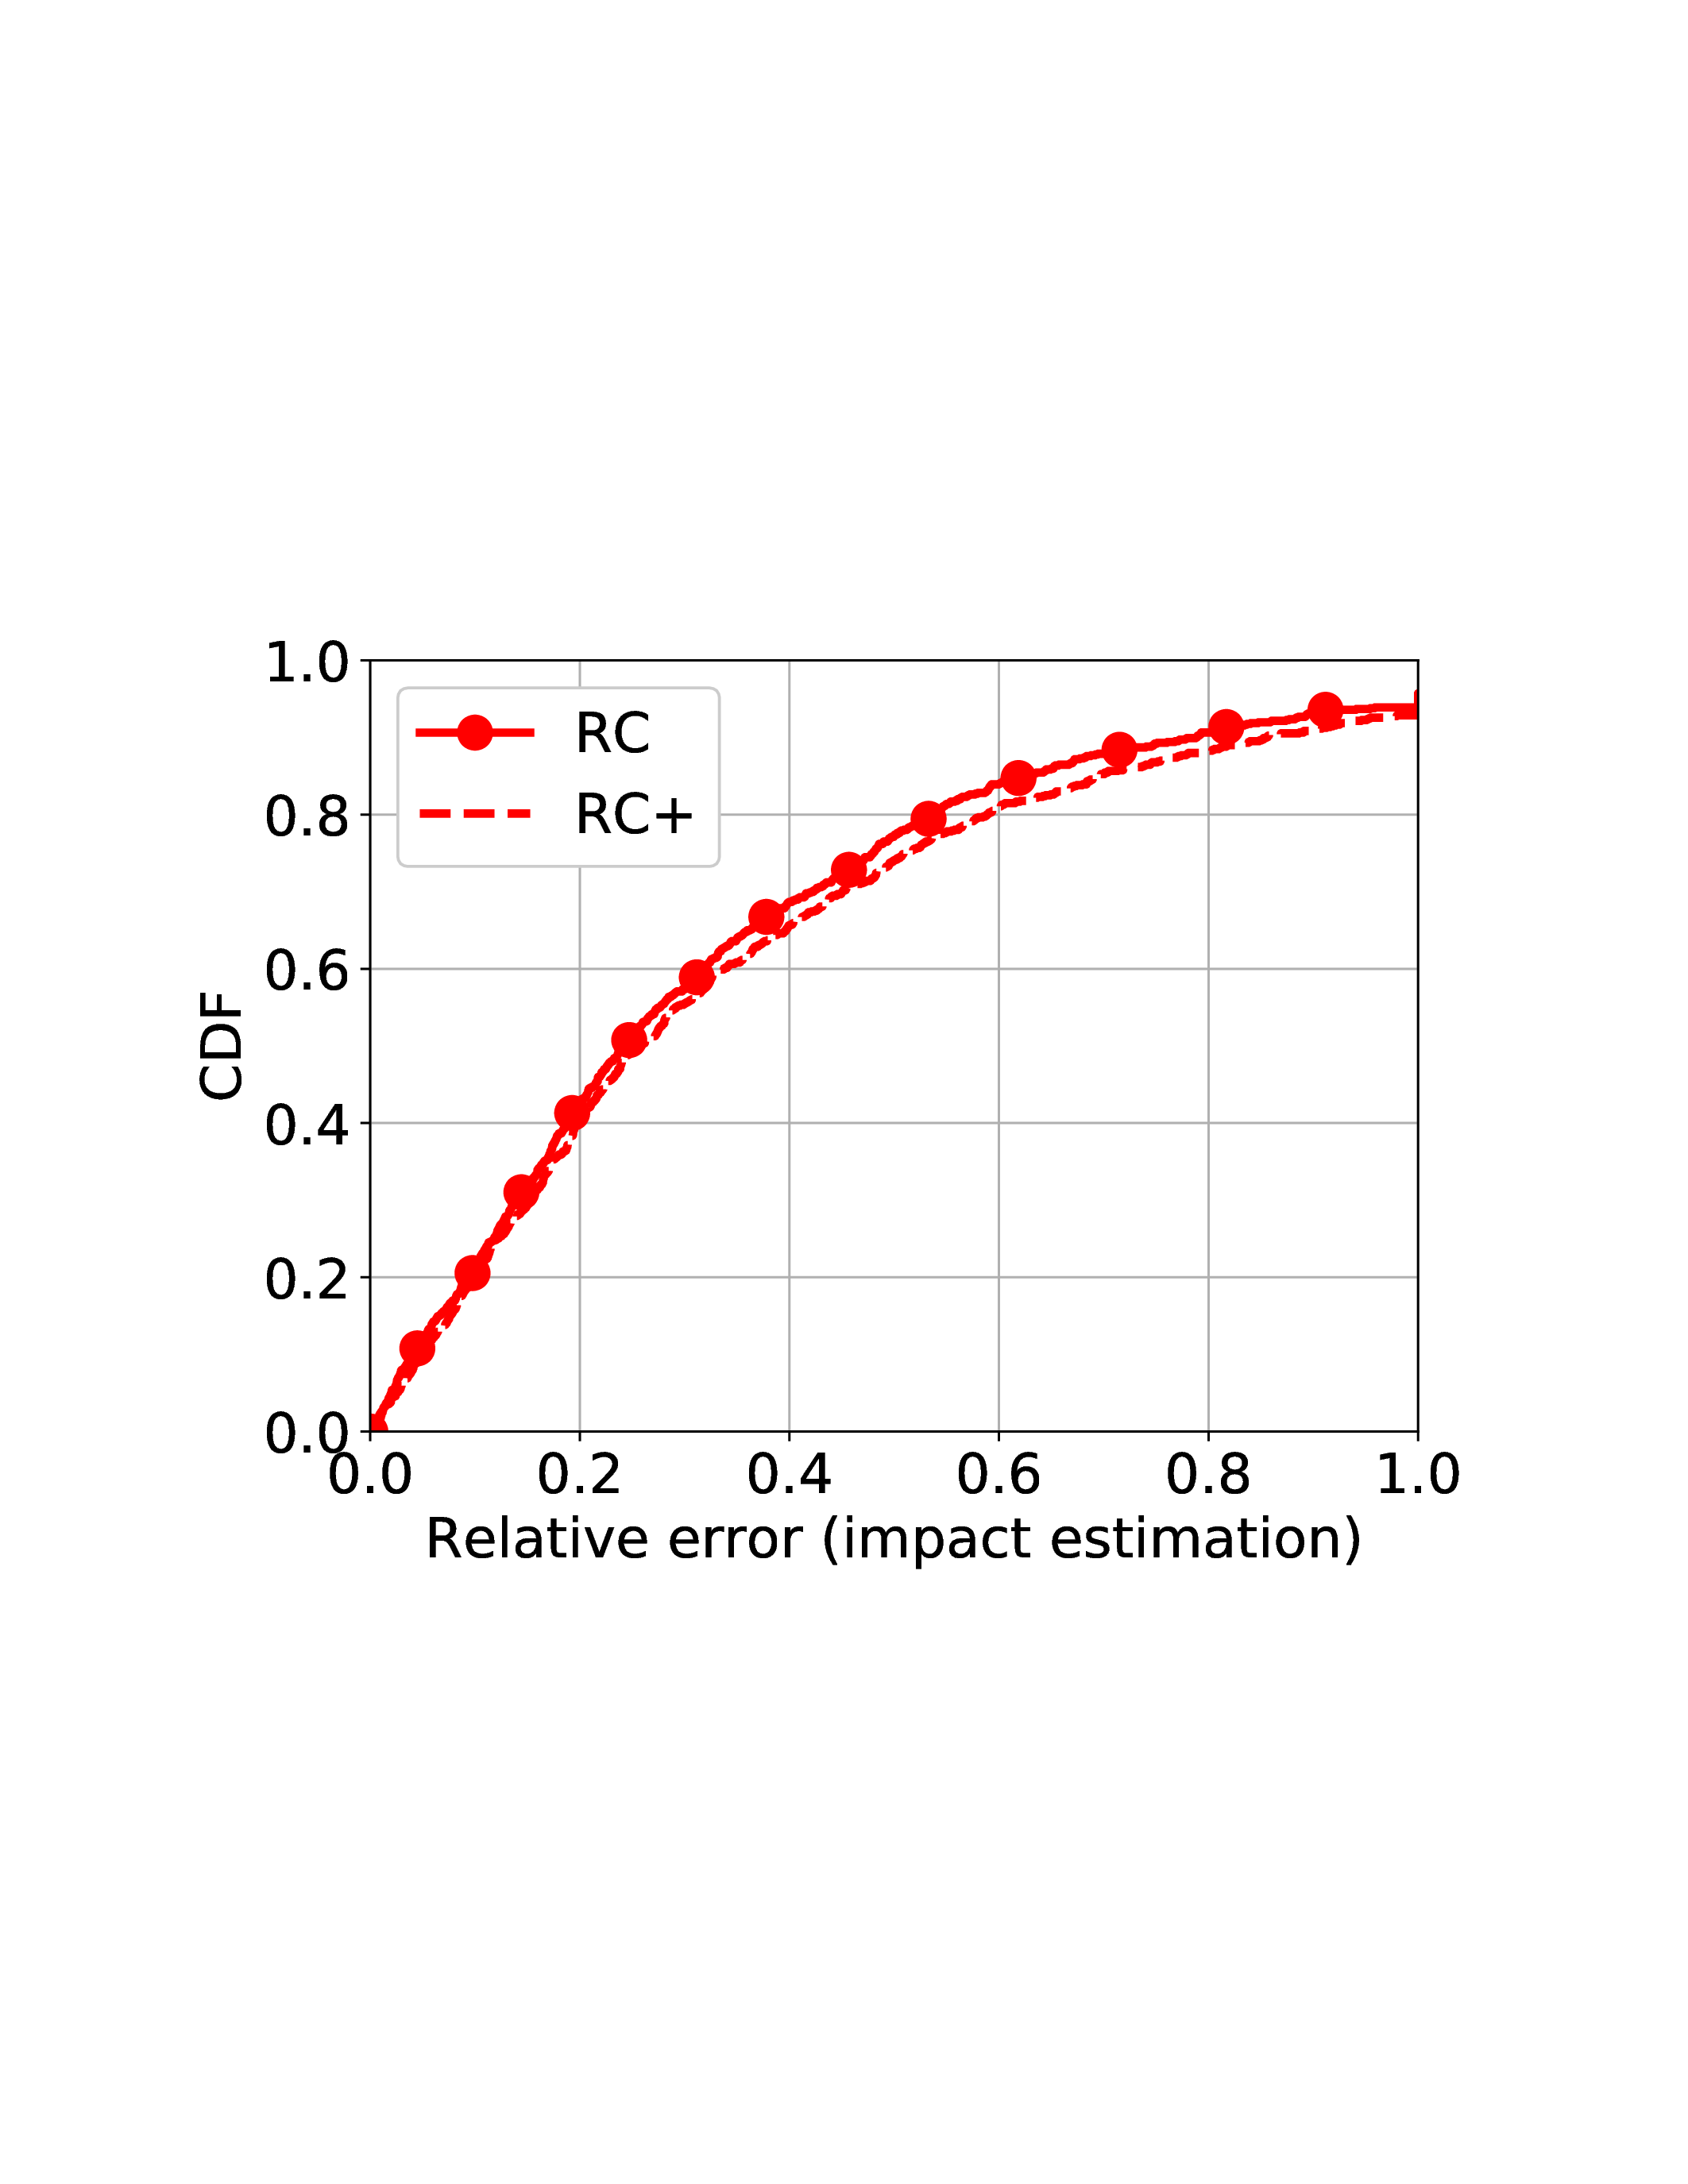}\label{fig:sims-impact-rc-vs-rc+-hijack-type-1}}
\subfigure[Hijack Type-2]{\includegraphics[width=0.33\linewidth]{./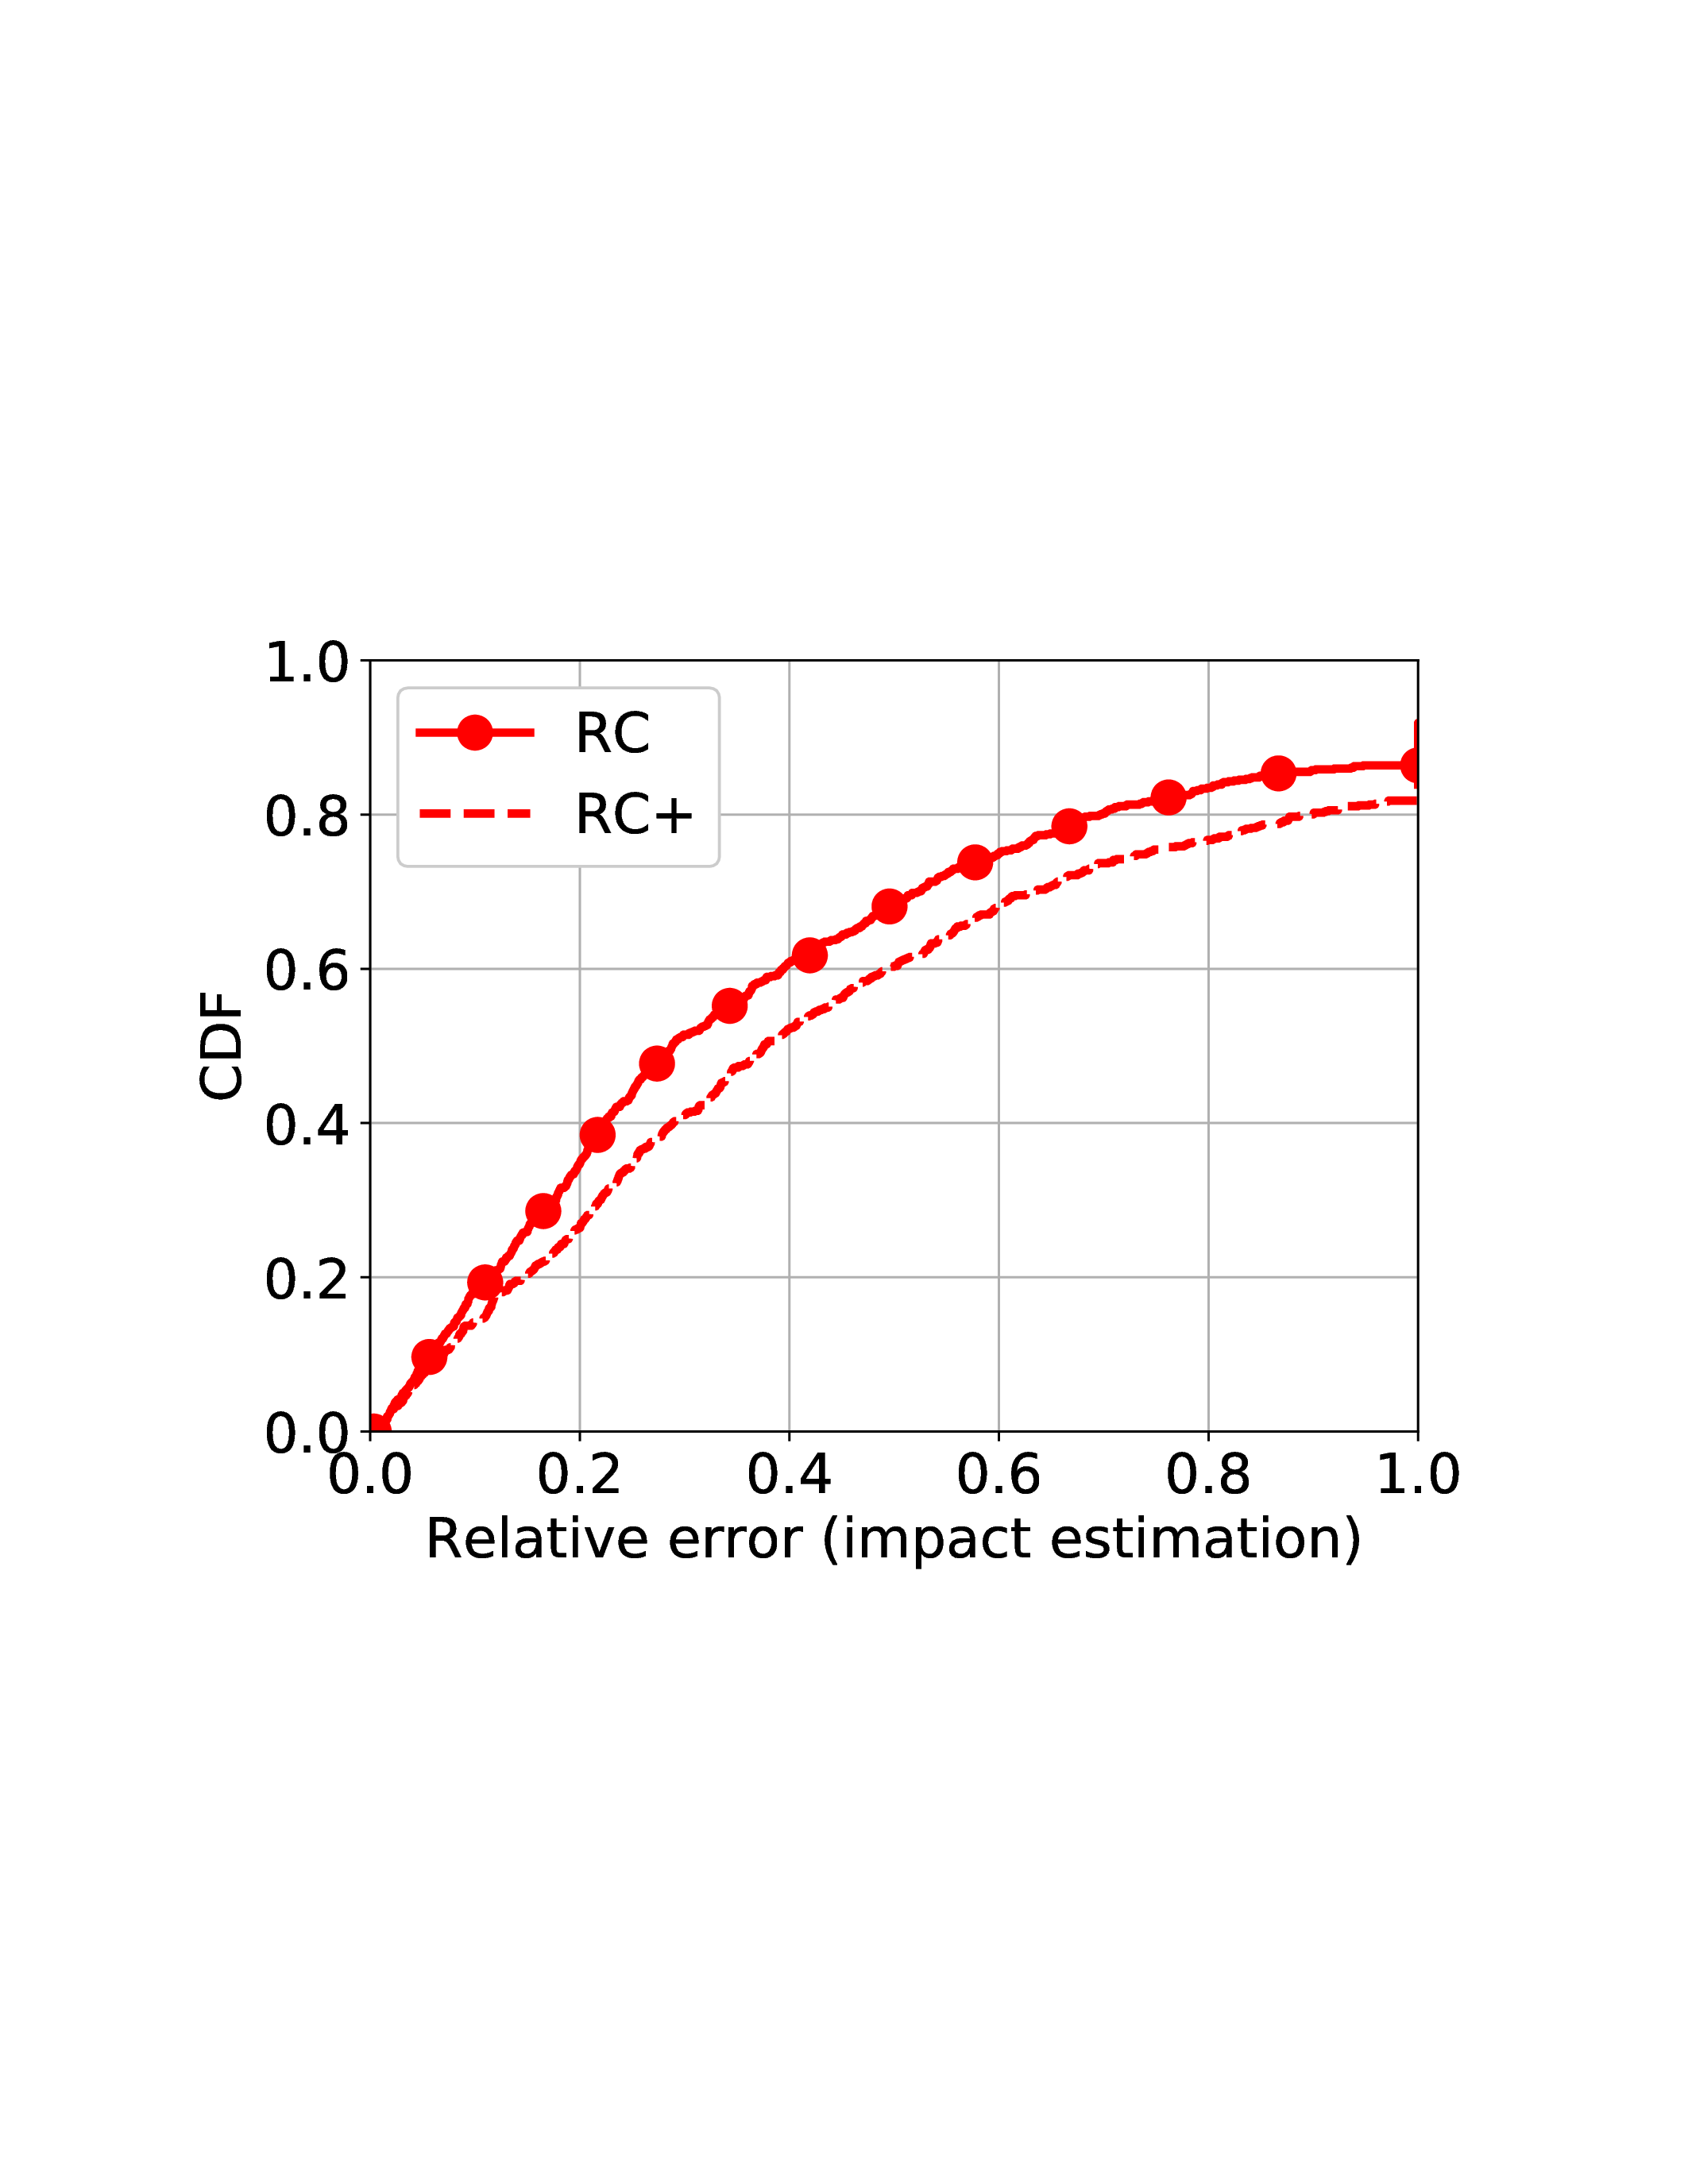}\label{fig:sims-impact-rc-vs-rc+-hijack-type-2}}
\subfigure[Hijack Type-0]{\includegraphics[width=0.33\linewidth]{./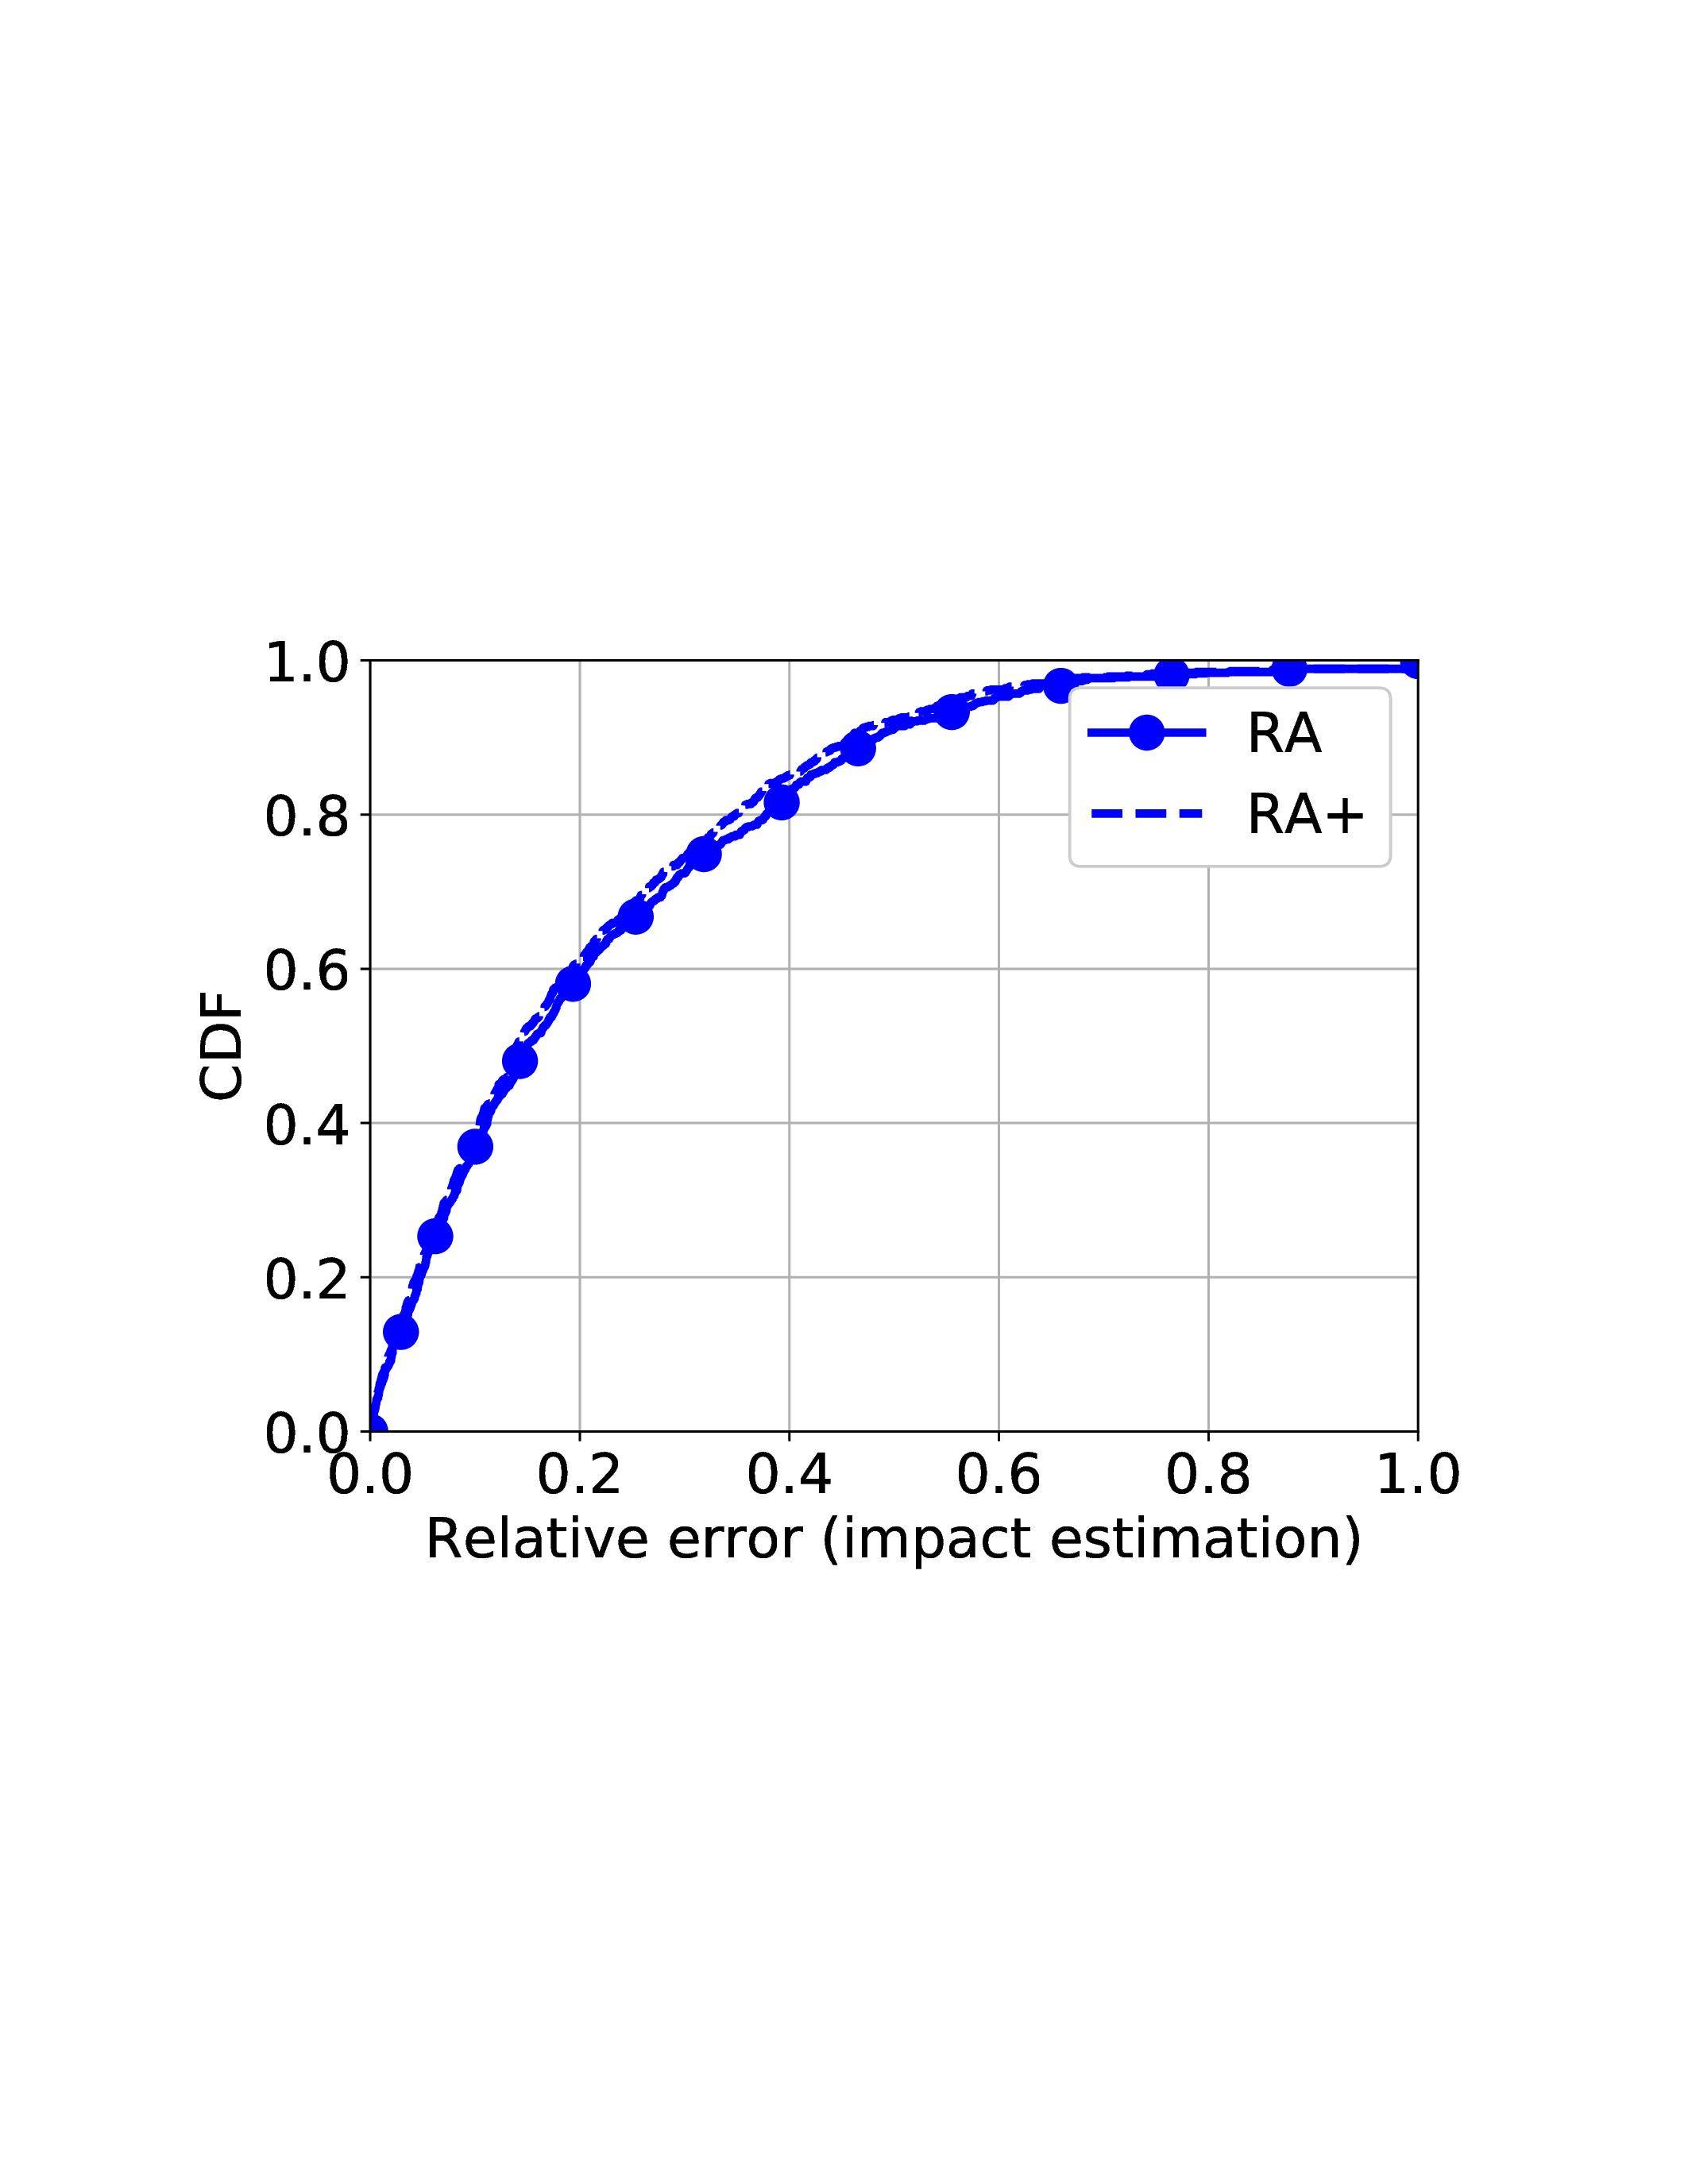}\label{fig:sims-impact-ra-vs-ra+-hijack-type-0}}
\subfigure[Hijack Type-1]{\includegraphics[width=0.33\linewidth]{./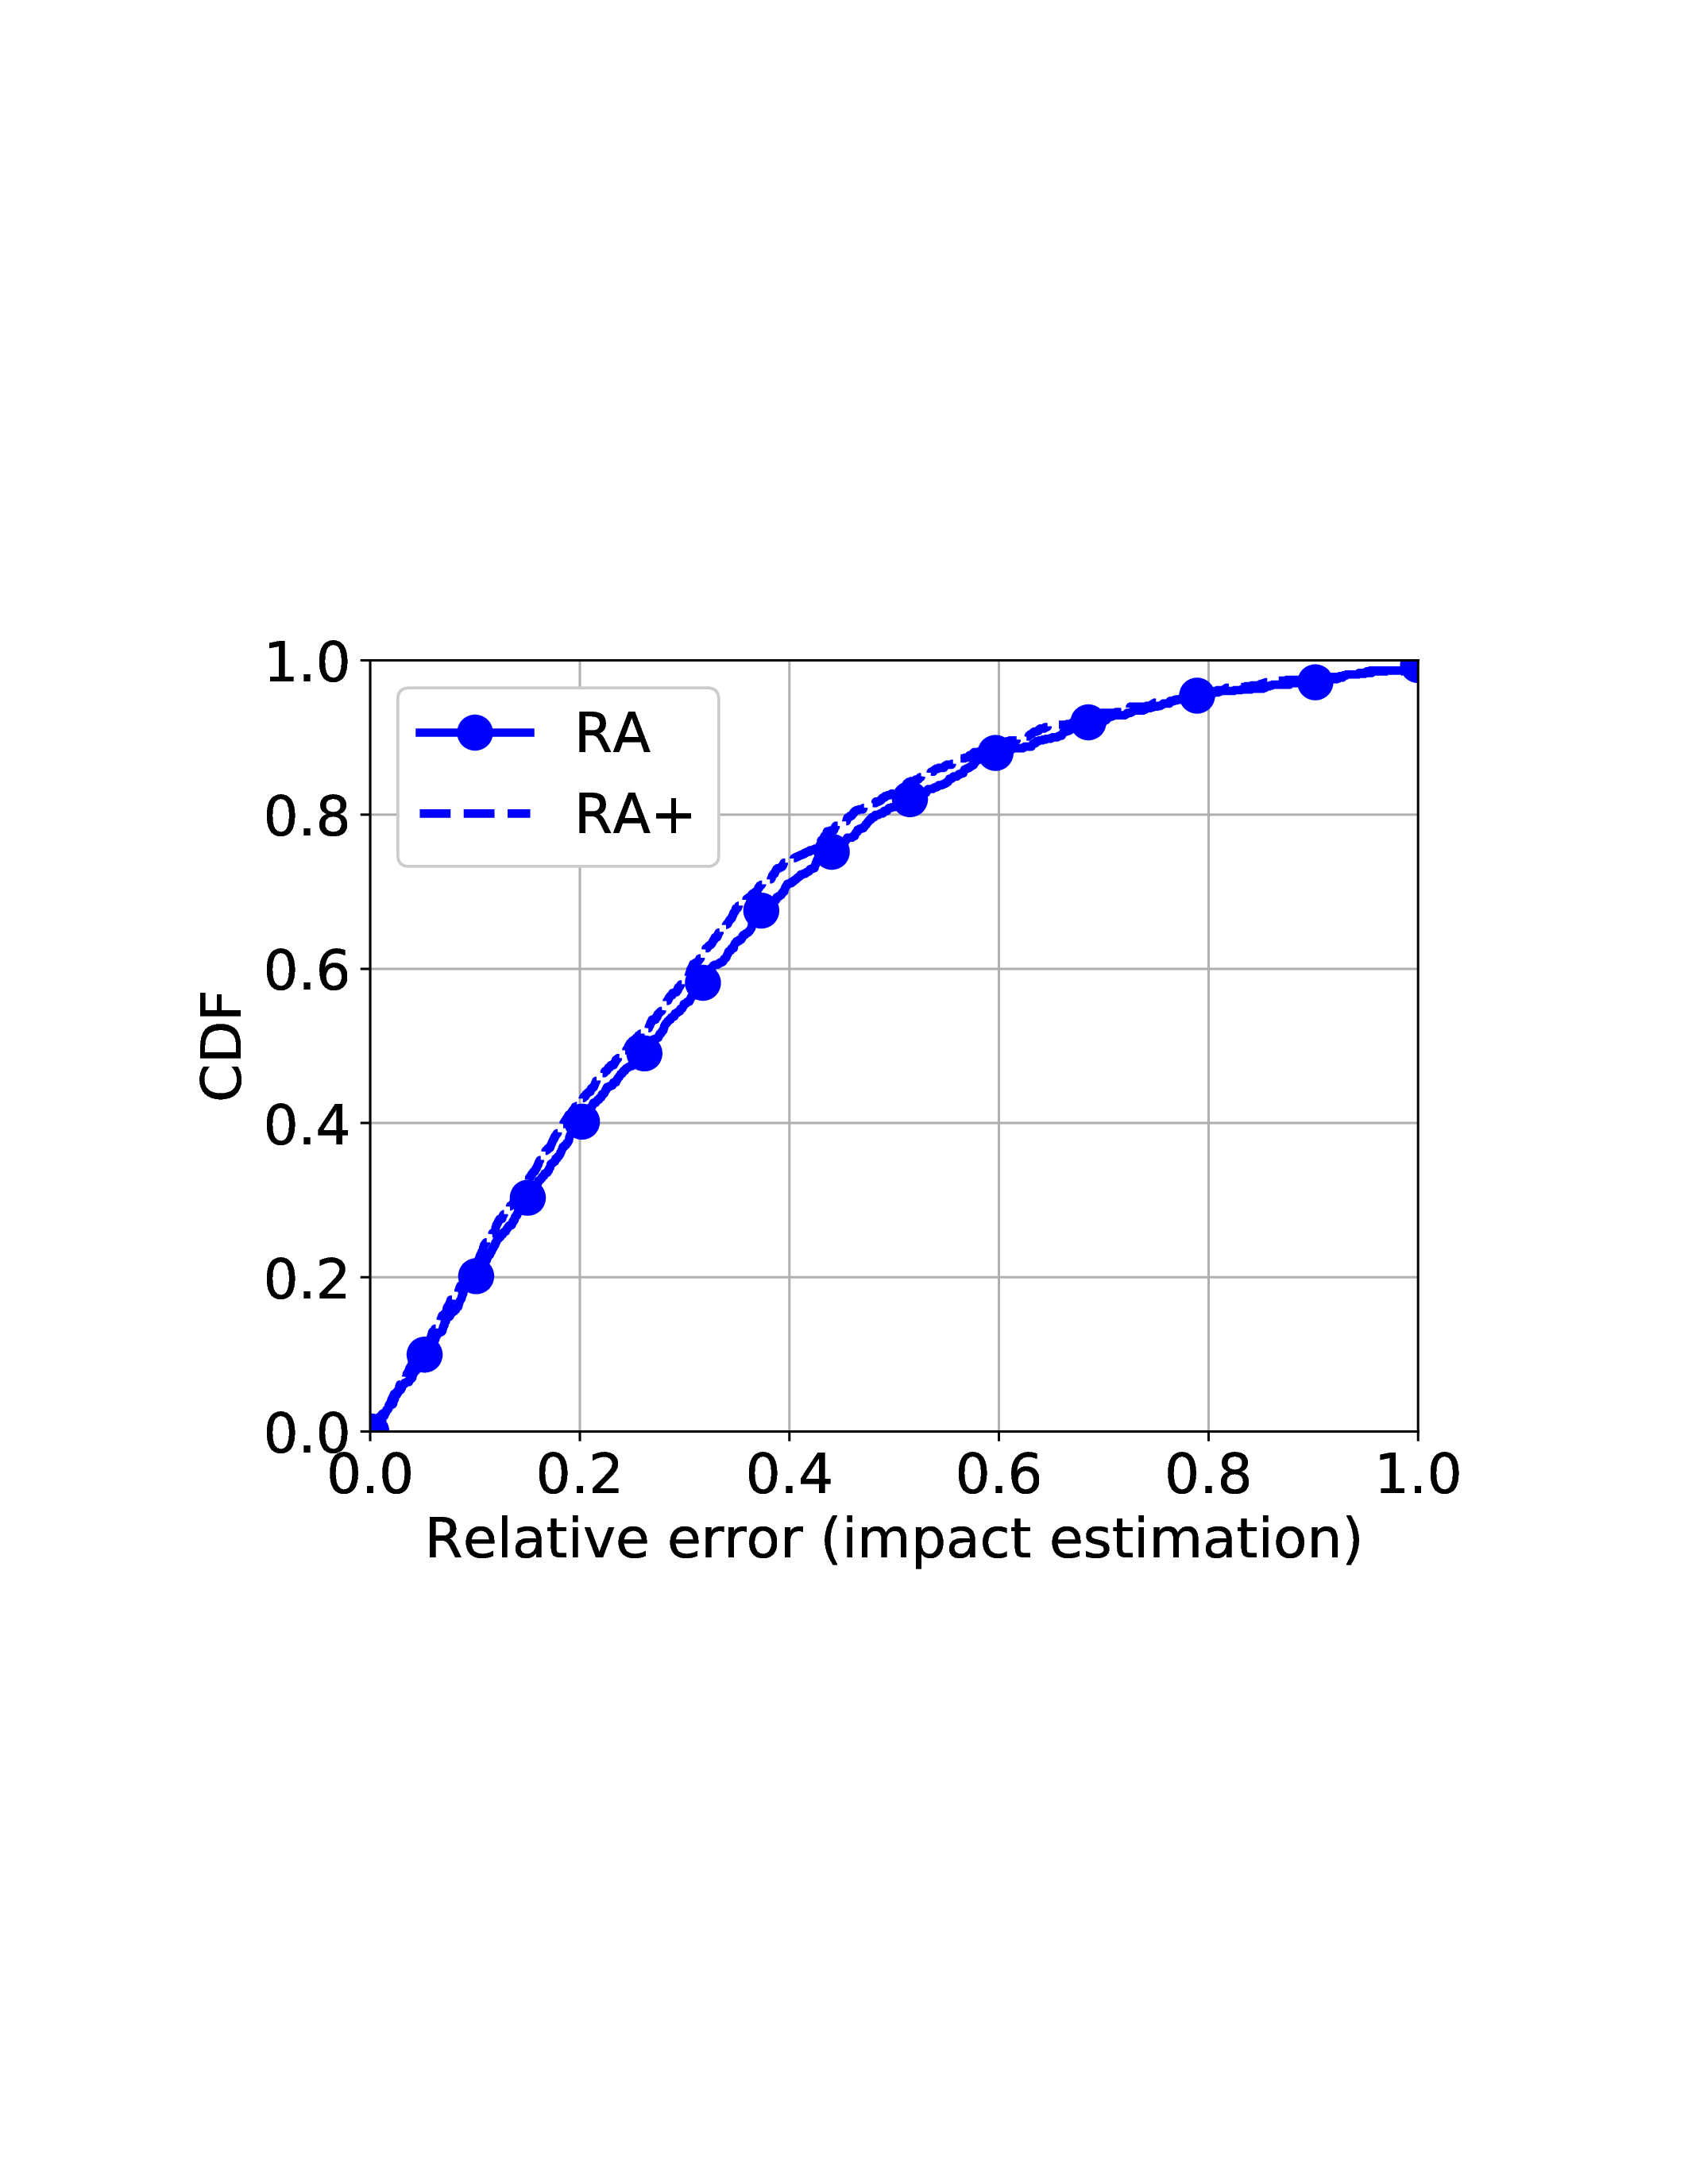}\label{fig:sims-impact-ra-vs-ra+-hijack-type-1}}
\subfigure[Hijack Type-2]{\includegraphics[width=0.33\linewidth]{./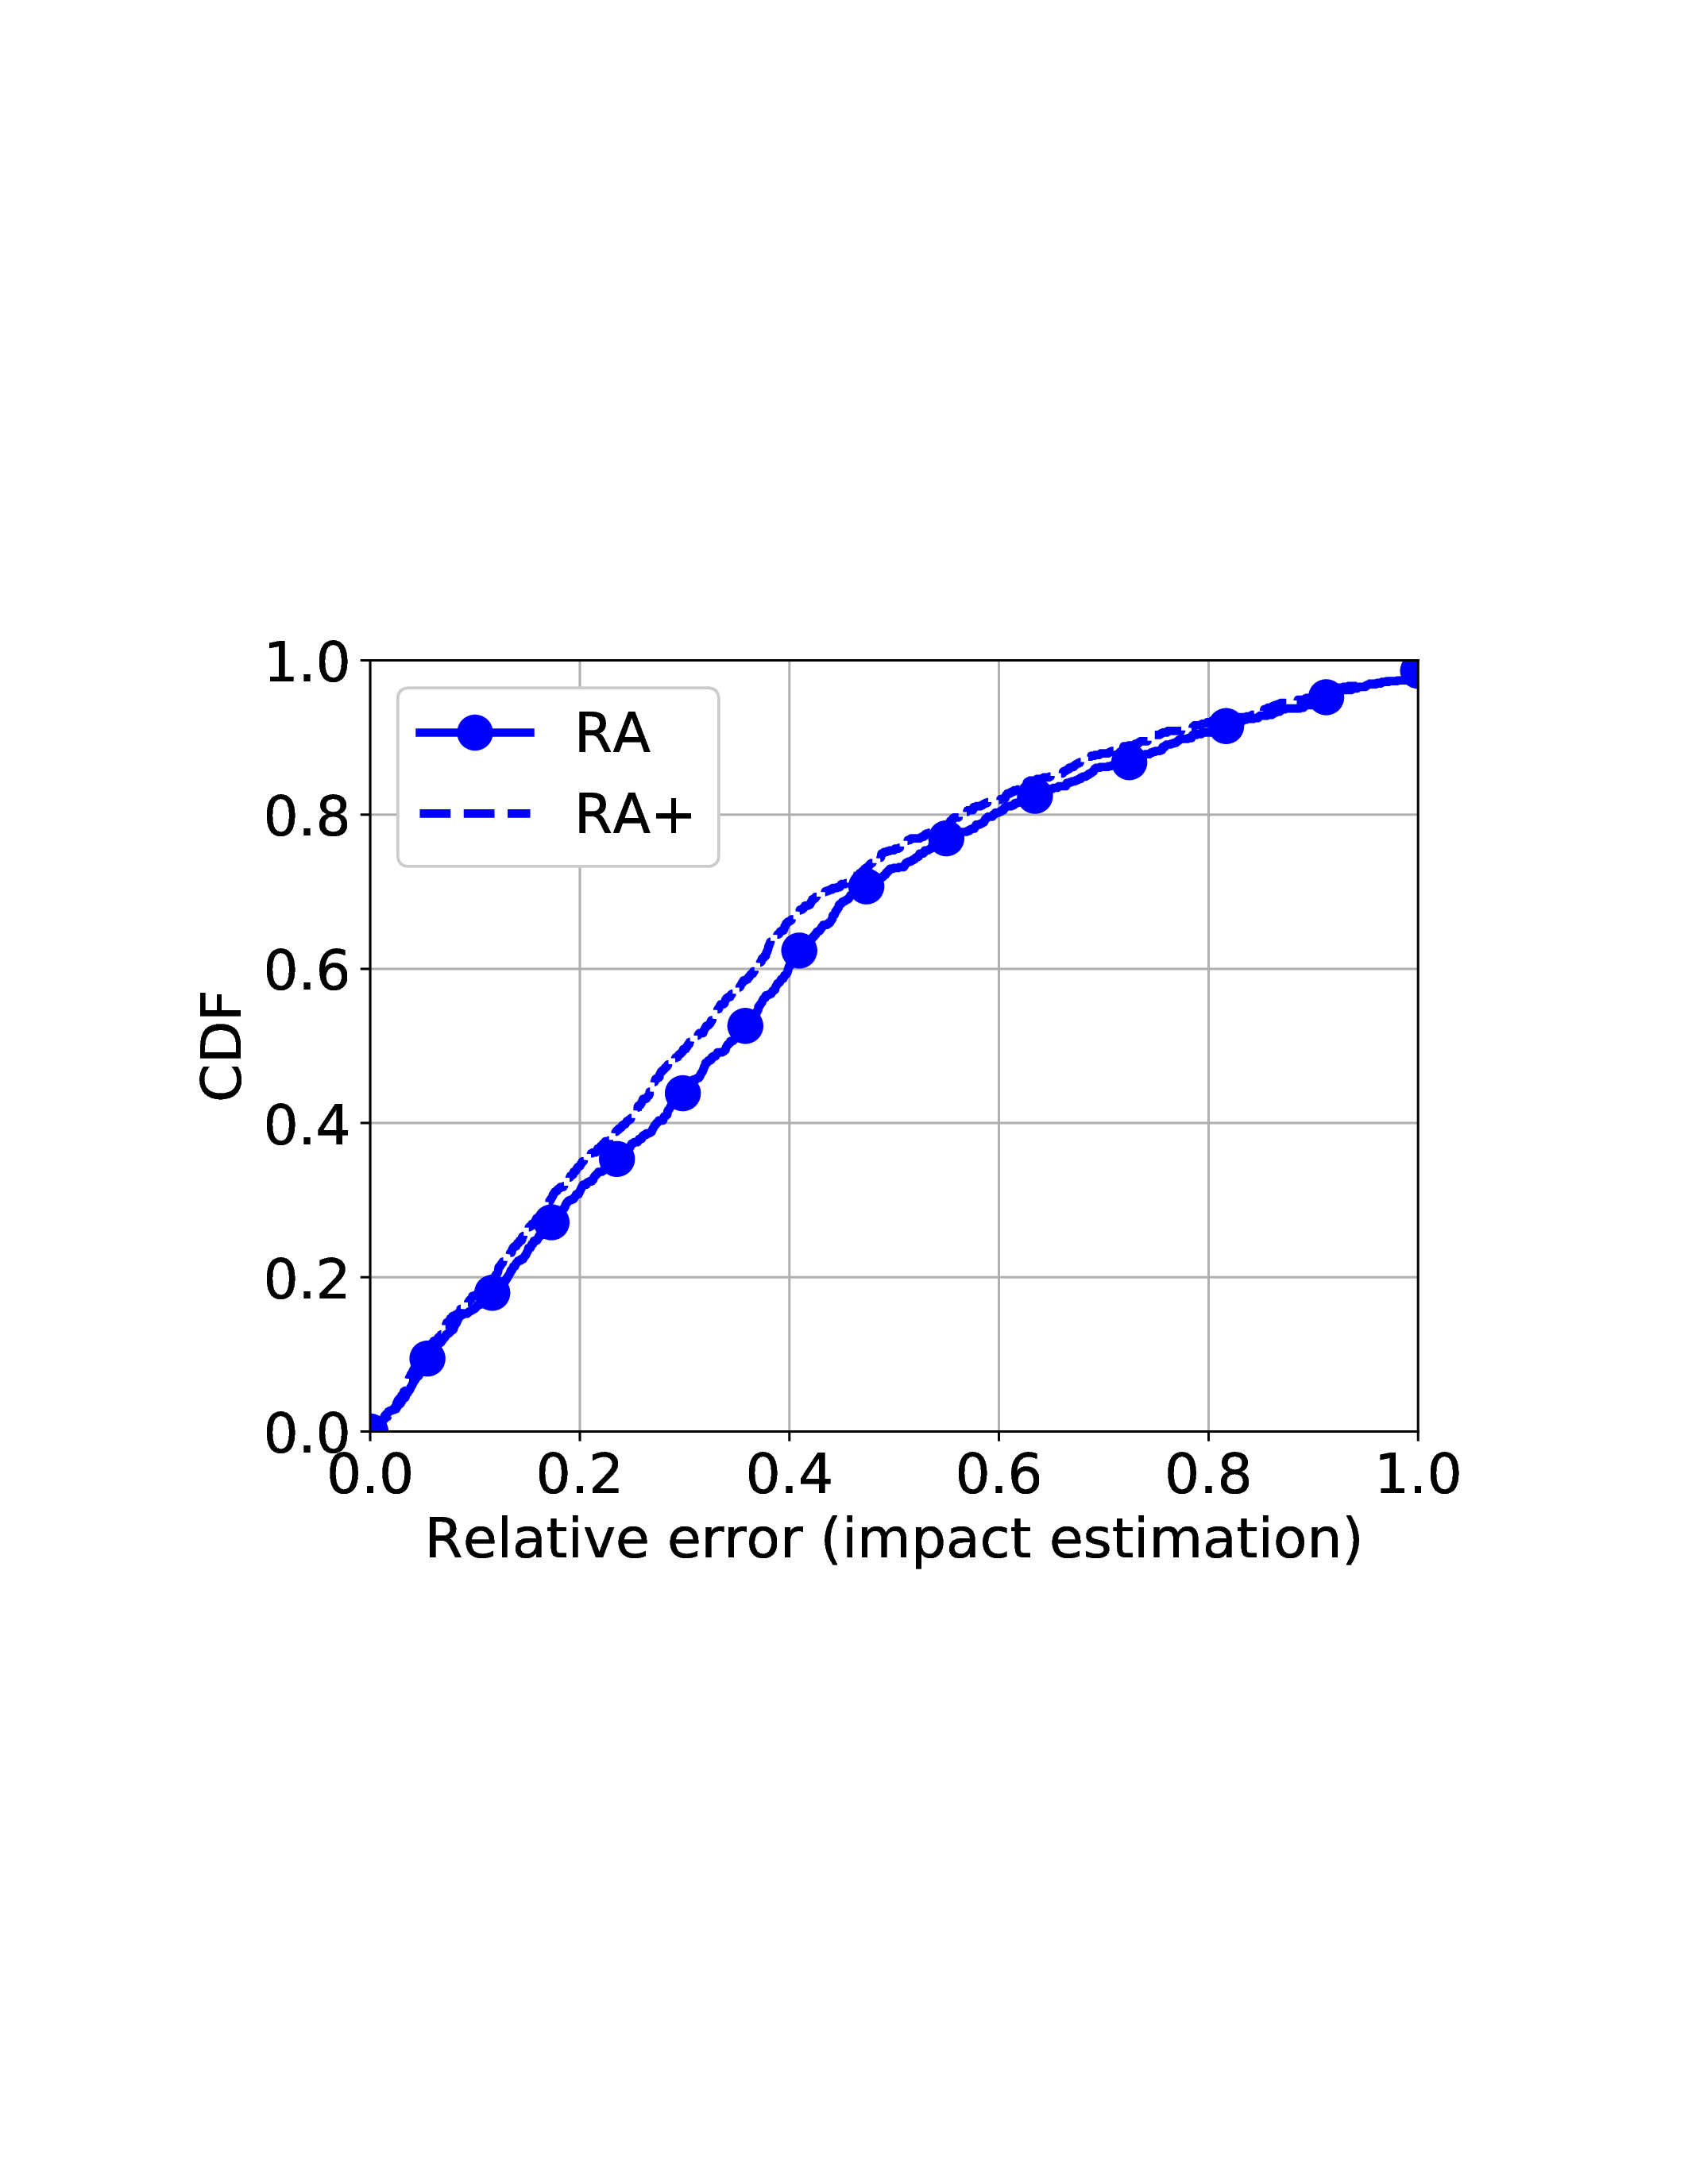}\label{fig:sims-impact-ra-vs-ra+-hijack-type-2}}
\caption{CDF of the relative error of impact estimation for hijacks of Type-0 (left plots), Type-1 (middle plots), and Type-2 (right plots). Comparison of impact estimated by route collector (RC) and RIPE Atlas (RA) measurements (top row); route collector (RC) and route collectors including all ASes in paths (RC+) (middle row); RIPE Atlas (RA) and RIPE Atlas including all ASes in paths (RA+) (bottom row). }
\label{fig:sims-impact-cdfs}
\end{figure*}

\begin{figure*}
\centering
\subfigure[Hijack Type-0]{\includegraphics[width=0.33\linewidth]{./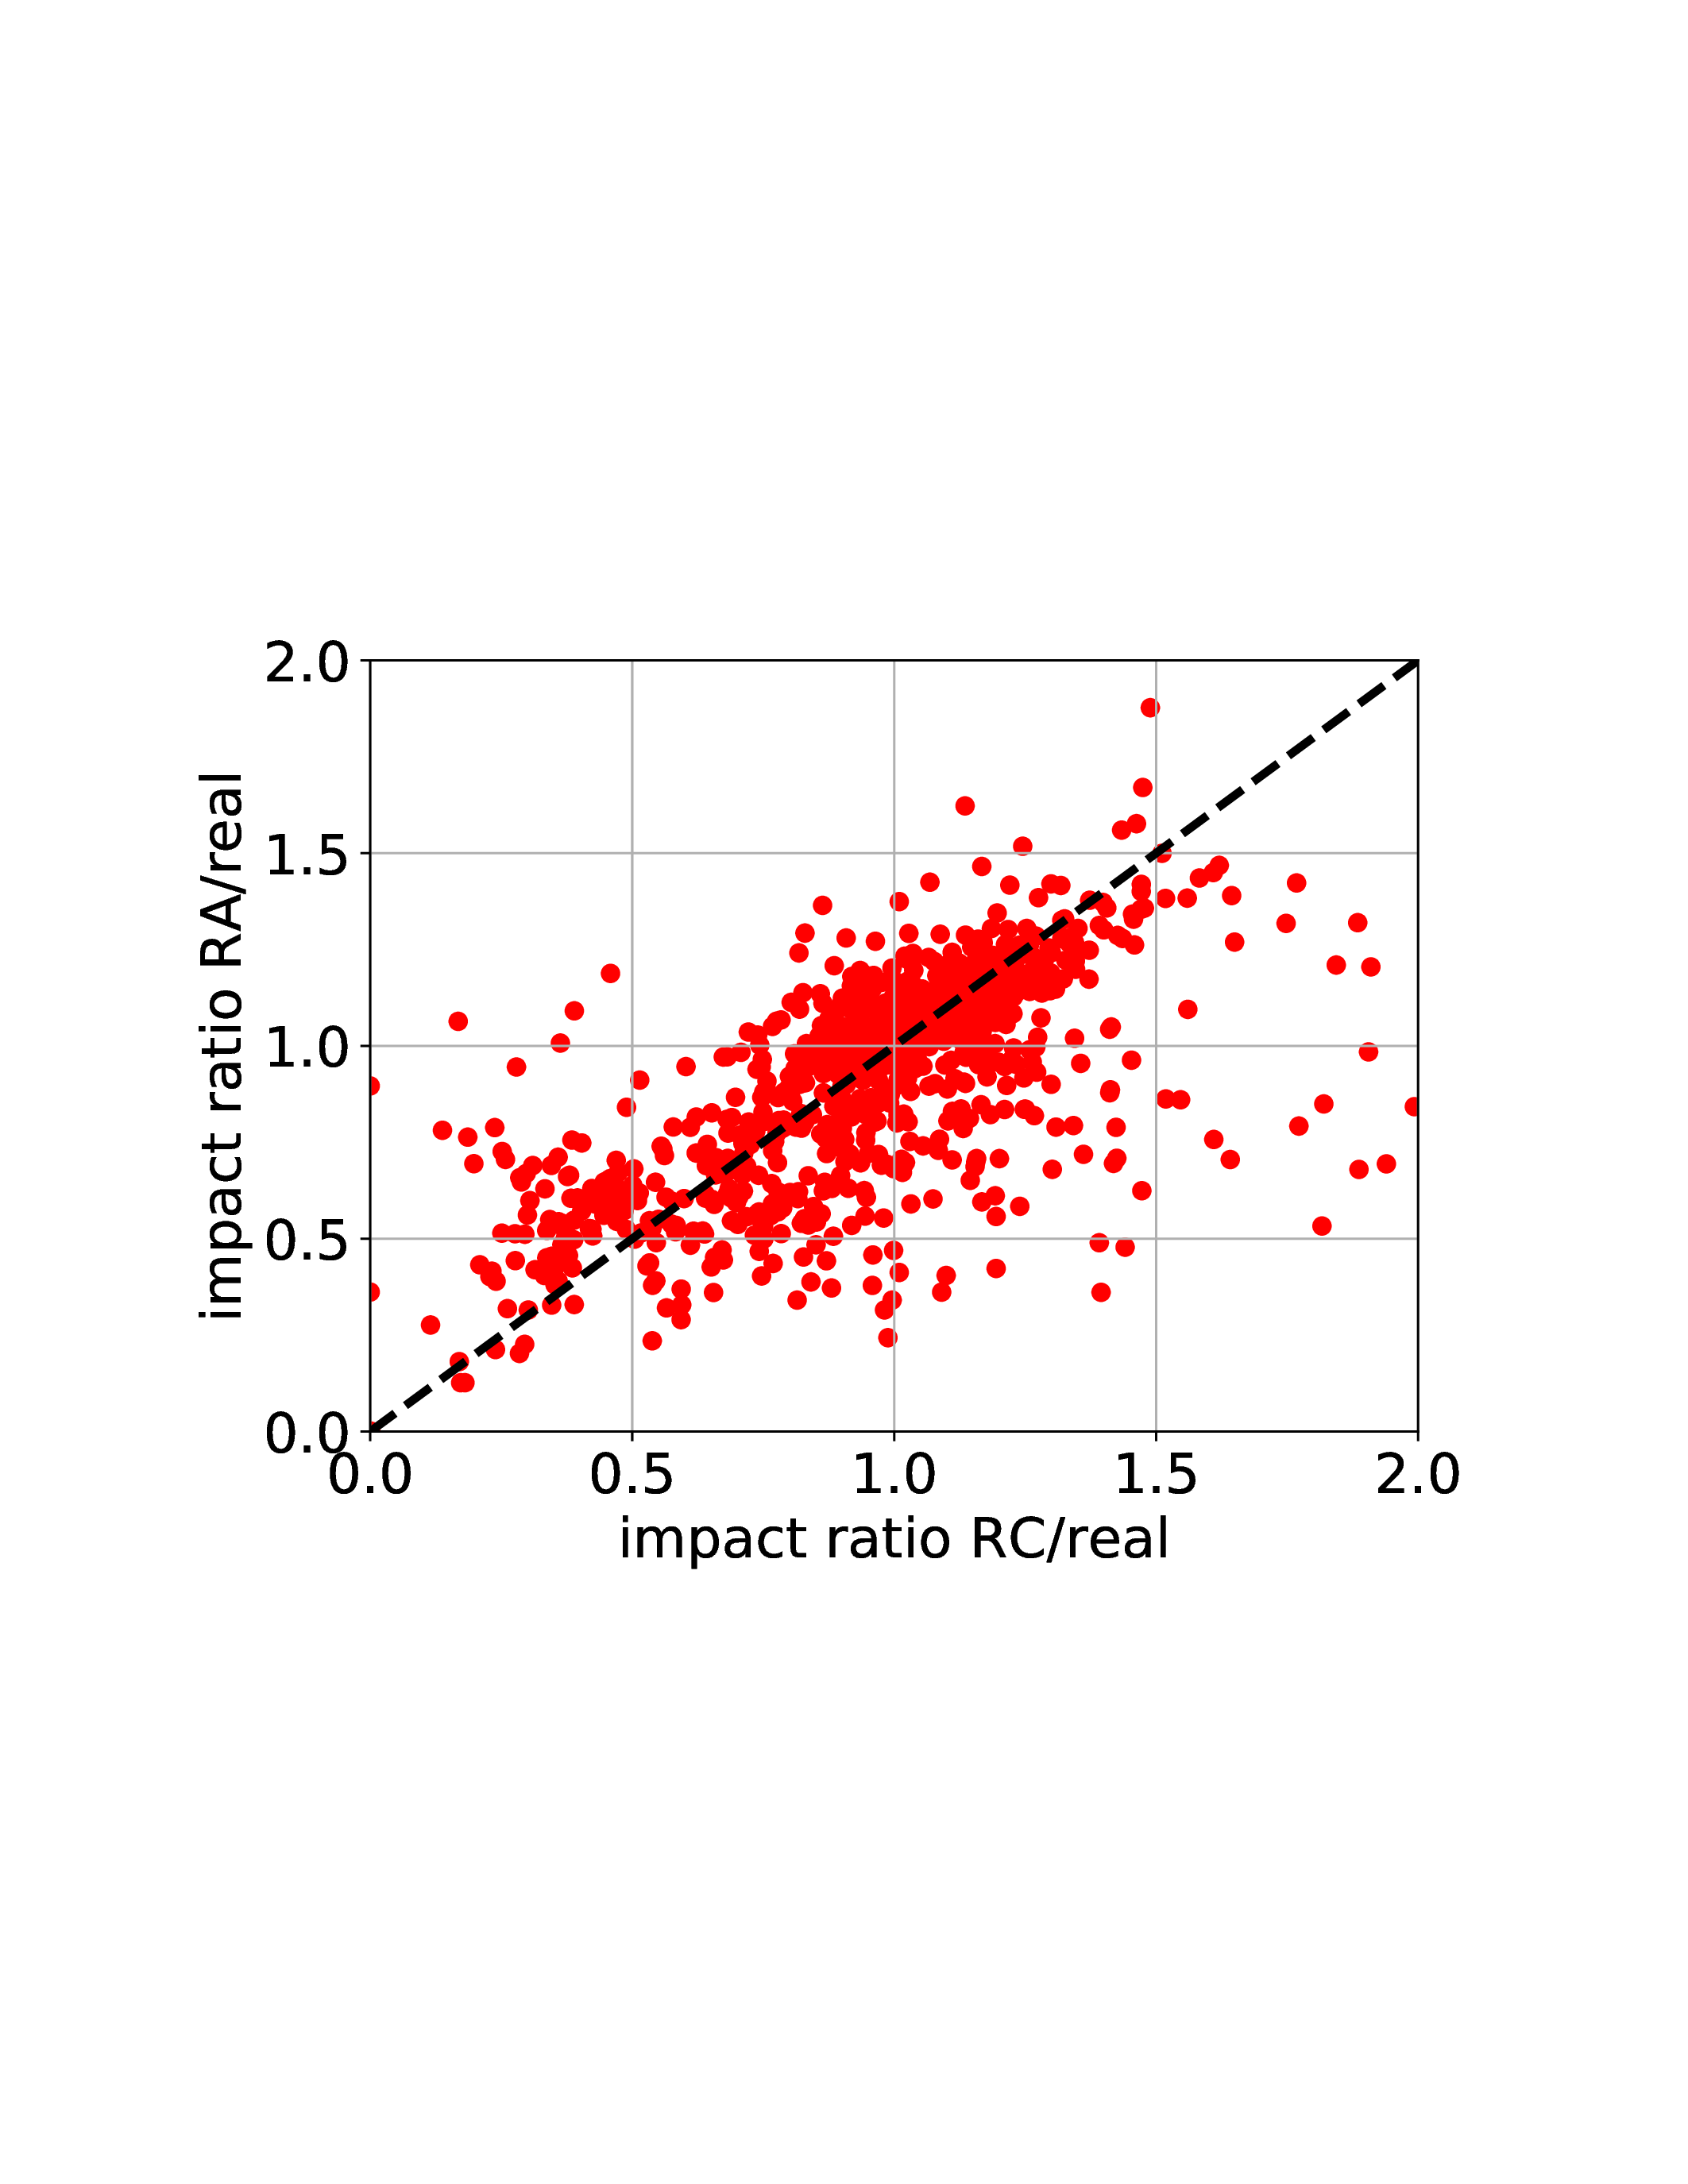}\label{fig:sims-impact-scatter-rc-vs-ra-hijack-type-0}}
\subfigure[Hijack Type-1]{\includegraphics[width=0.33\linewidth]{./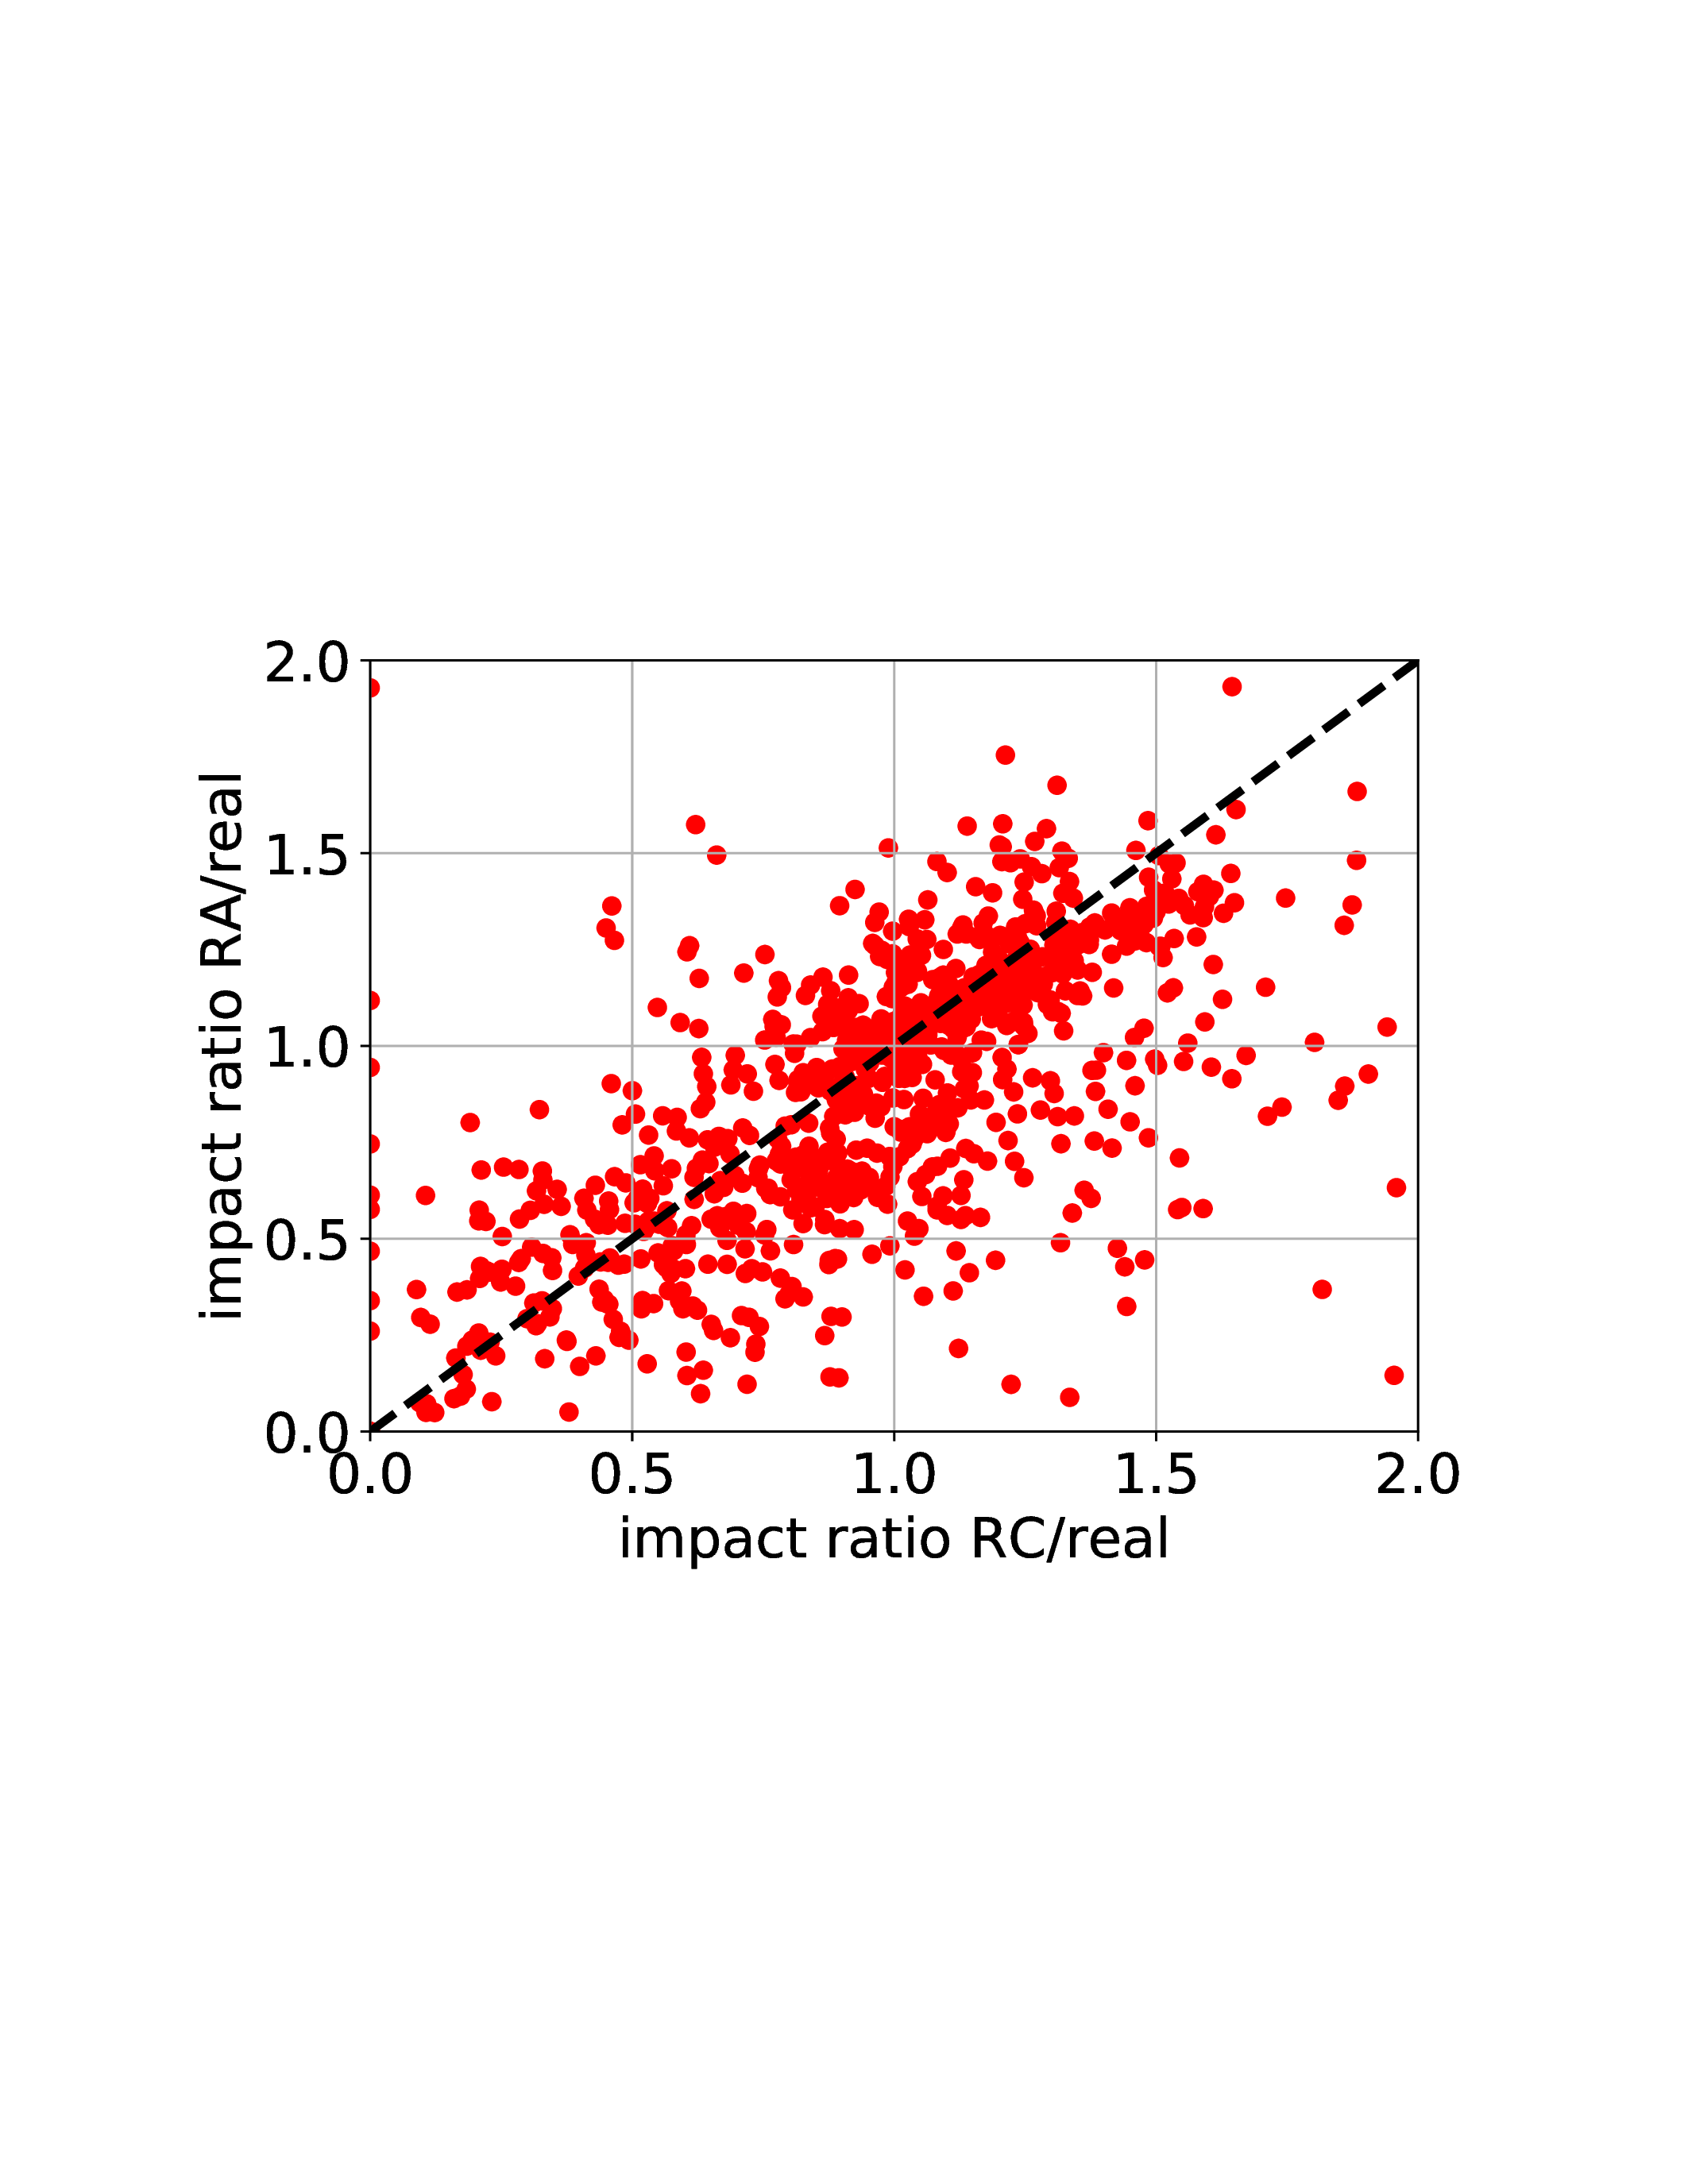}\label{fig:sims-impact-scatter-rc-vs-ra-hijack-type-1}}
\subfigure[Hijack Type-2]{\includegraphics[width=0.33\linewidth]{./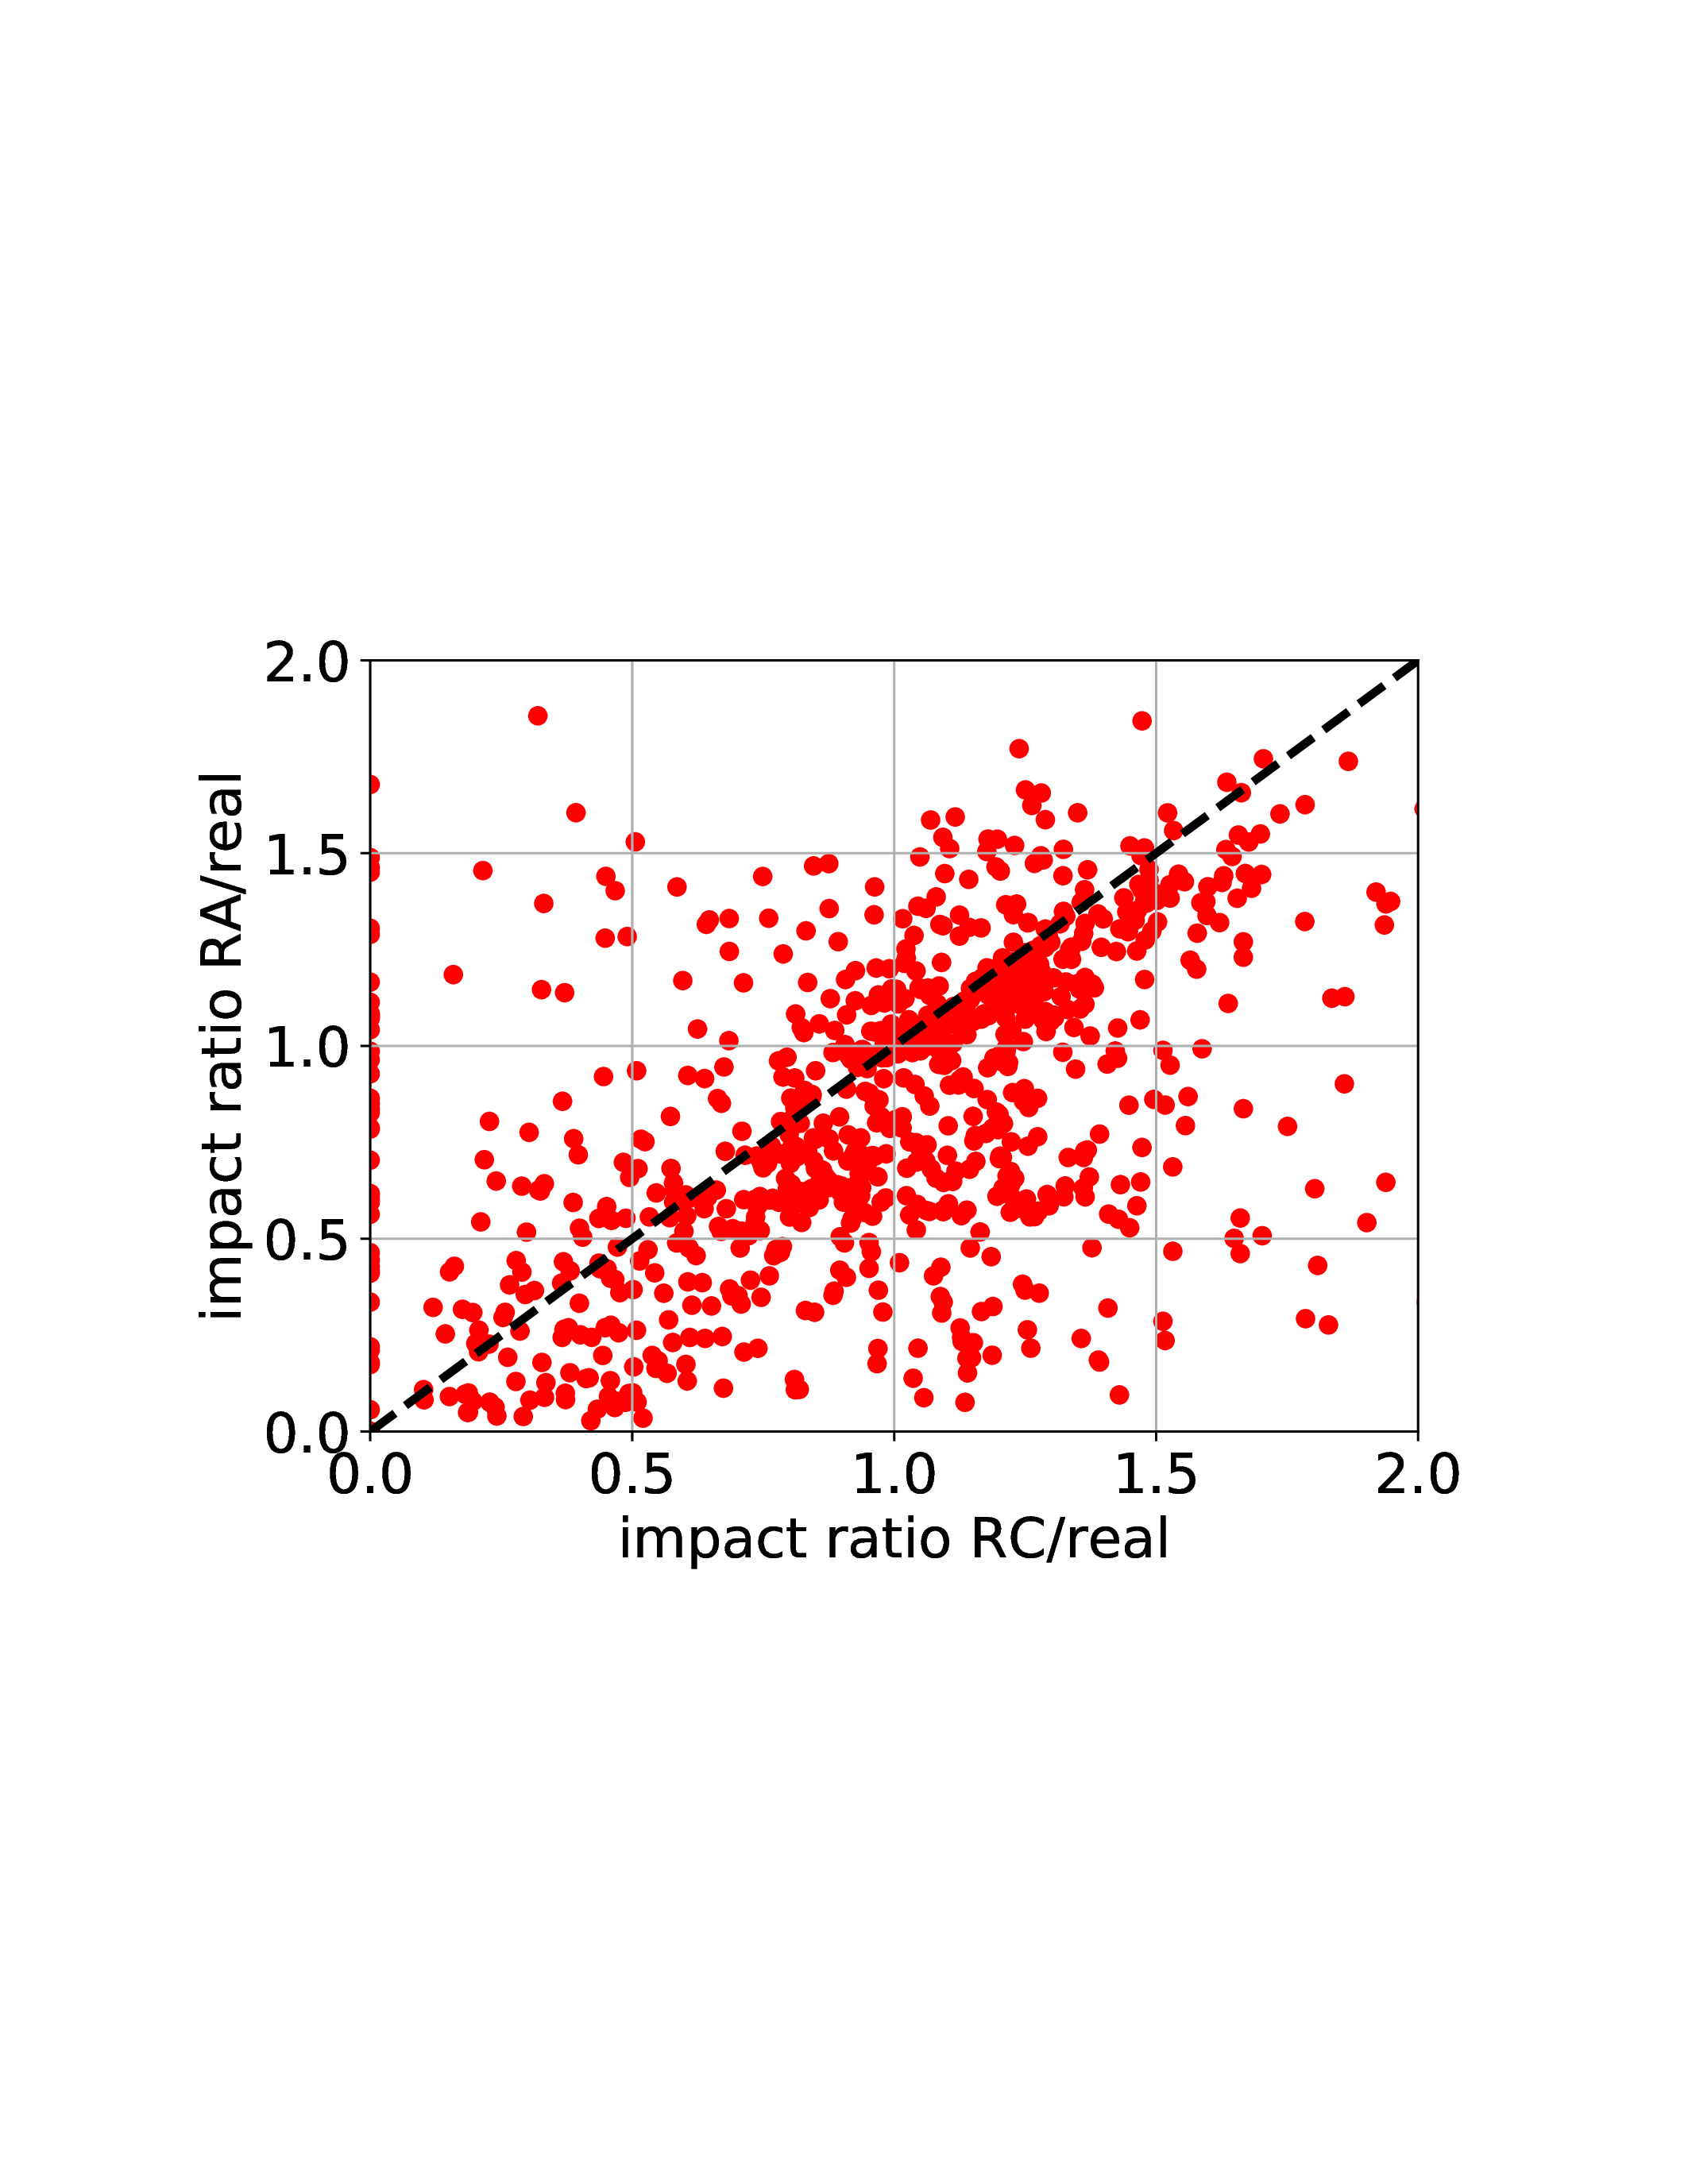}\label{fig:sims-impact-scatter-rc-vs-ra-hijack-type-2}}
\caption{Scatter plot: impact ratio seen from route collectors over real impact ratio (x-axis) vs. impact ratio seen from RIPE Atlas over real impact ratio (y-axis) for hijacks of Type-0, 1, and 2.}
\label{fig:sims-impact-scatter}
\end{figure*}

\begin{figure*}
\centering
\subfigure[NIE (Type-1 hijack)]{\includegraphics[width=0.49\linewidth]{./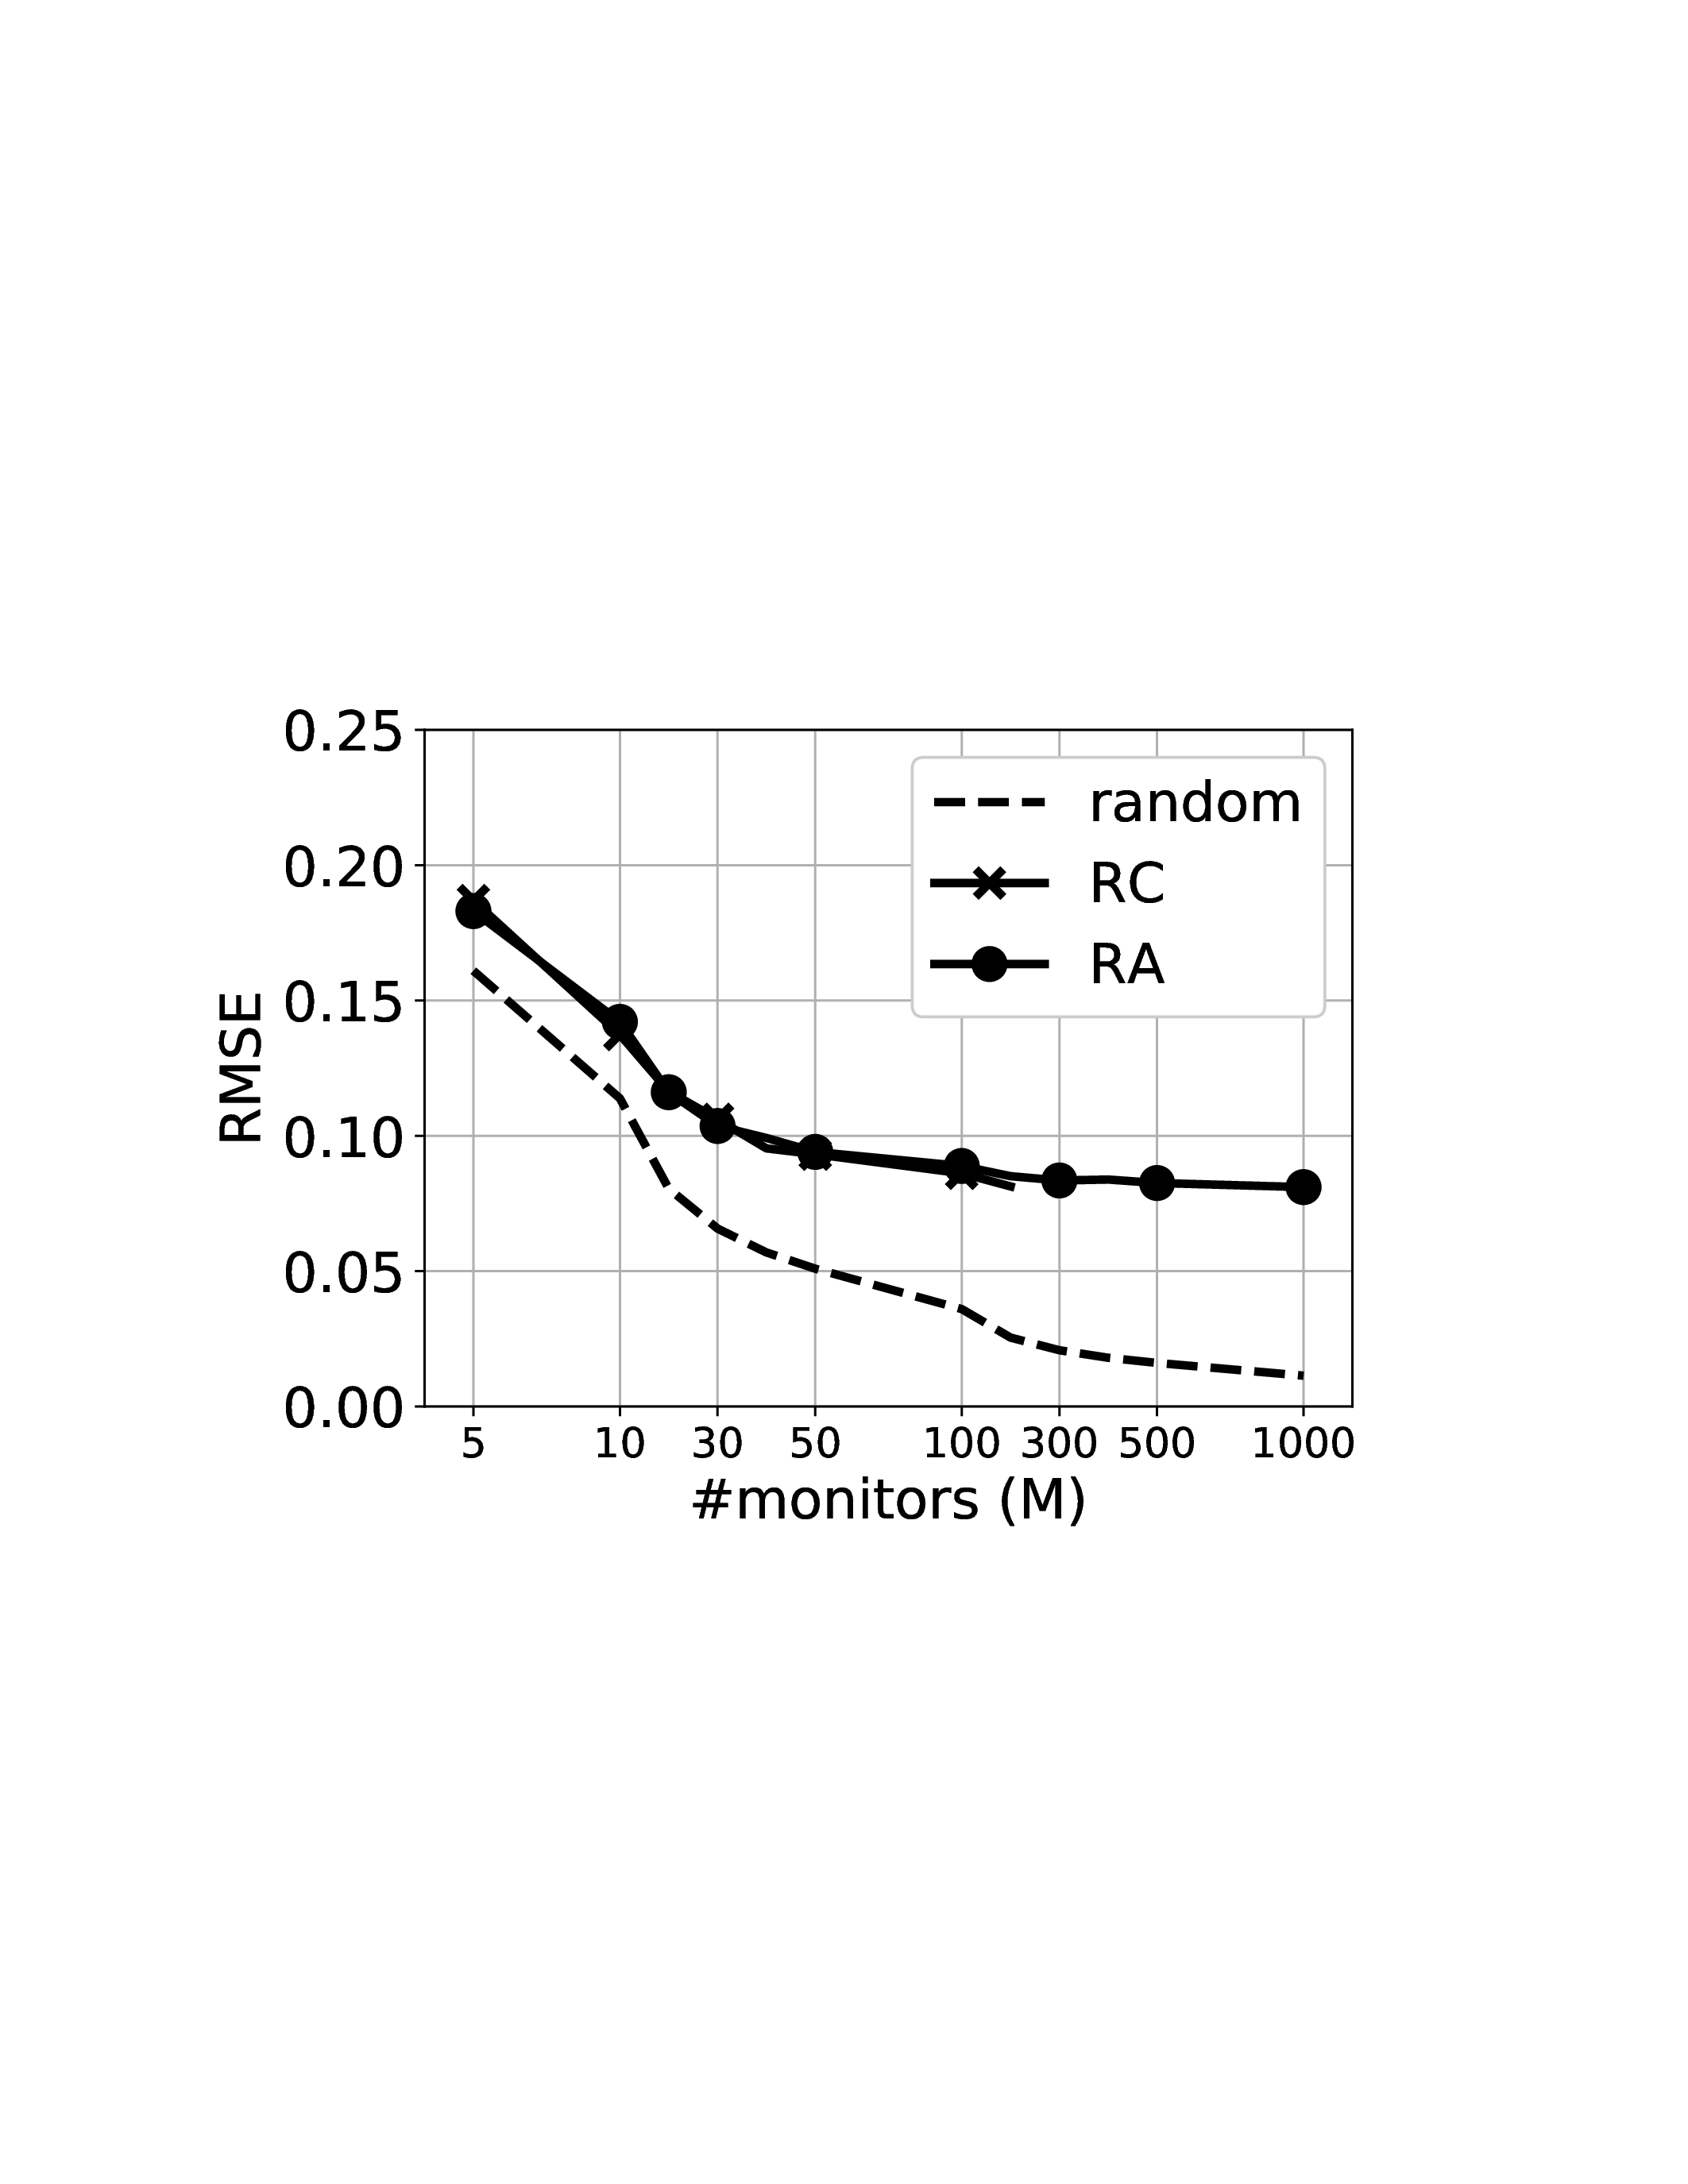}\label{fig:RMSE-NIE-random-RC-RA-vs-nb-monitors-Type1}}
\subfigure[NIE (Type-2 hijack)]{\includegraphics[width=0.49\linewidth]{./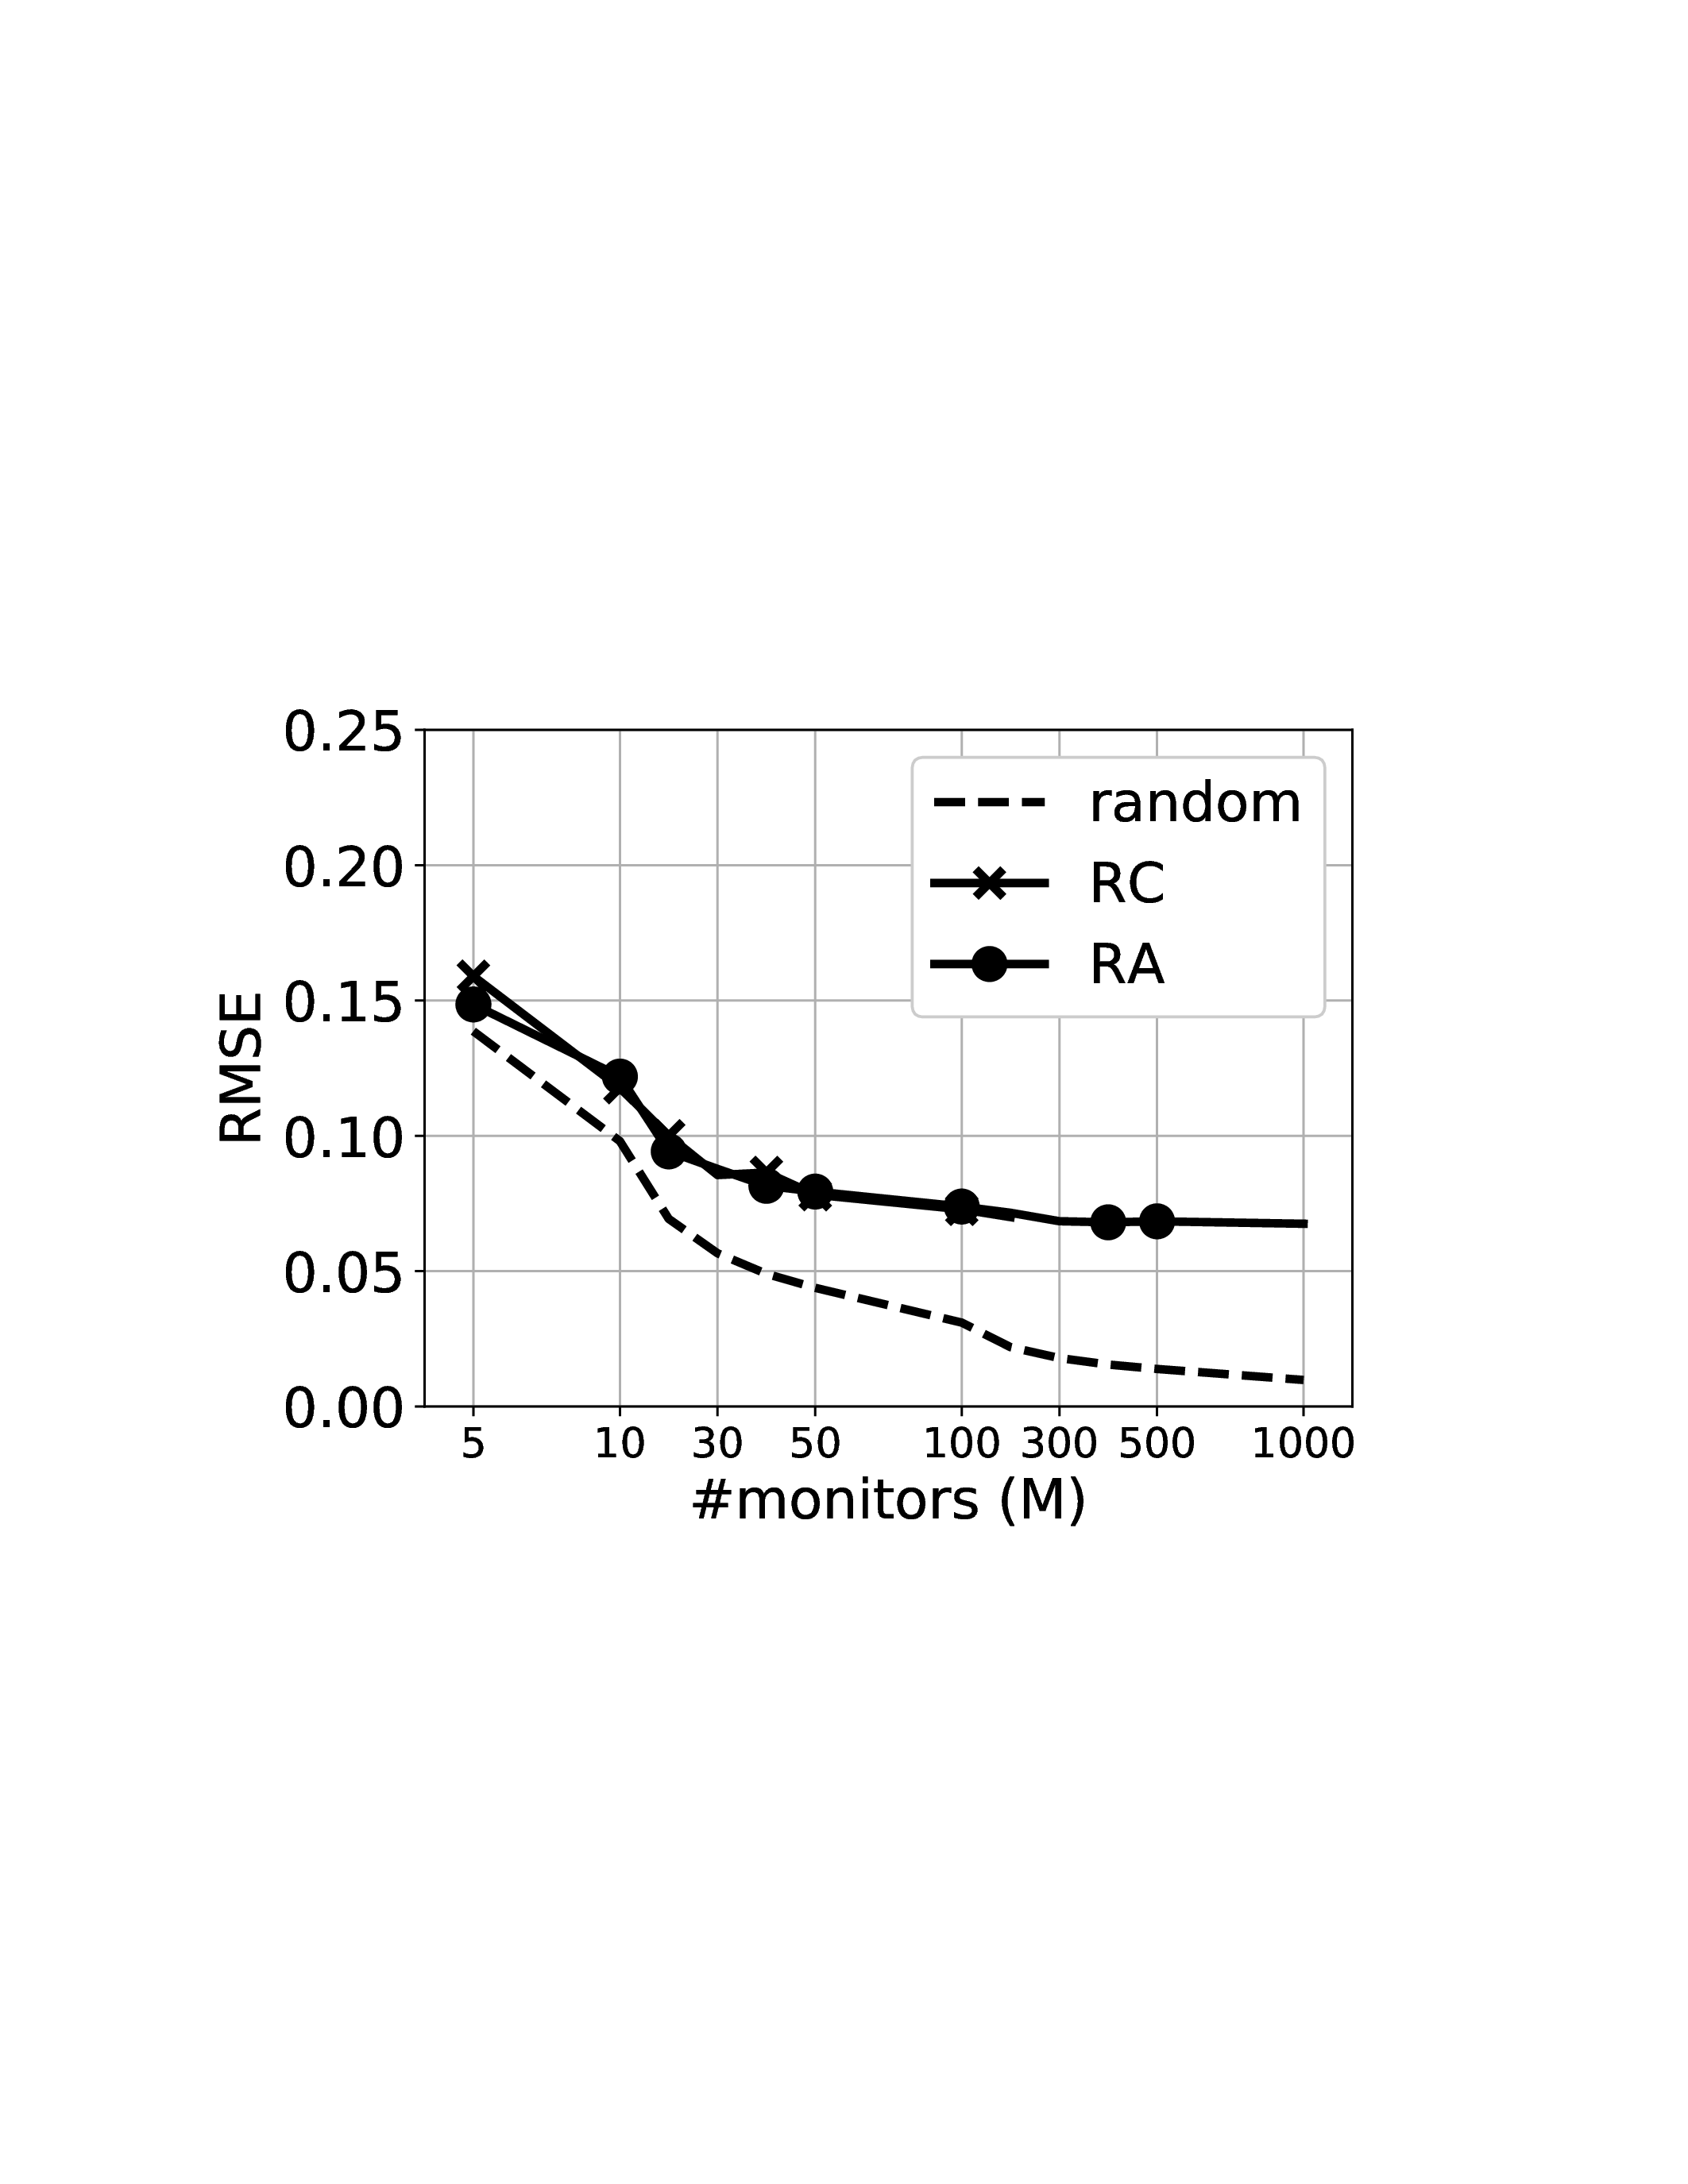}\label{fig:RMSE-NIE-random-RC-RA-vs-nb-monitors-Type2}}
\caption{RMSE of the NIE (y-axis) vs. number of monitors (x-axis) for random sets, RC, and RA monitors for (a) Type-1 and (b) Type-2 hijacks.}
\label{fig:RMSE-NIE-rnd-RC-RA-vs-nb-monitors}
\end{figure*}

\section{Impact Estimation with the R-graph Method}\label{appendix:Rgraph-method}
See Fig.~\ref{fig:sims-impact-Rgraph-cdfs}.

\begin{figure*}
\centering
\subfigure[no measurements]{\includegraphics[width=0.33\linewidth]{./figures/fig_impact_Rgraph_certain_vs_prob_hijackType0_no_measurement.eps}\label{fig:sims-impact-Rgraph-cdfs-no-measurement}}
\subfigure[with RC]{\includegraphics[width=0.33\linewidth]{./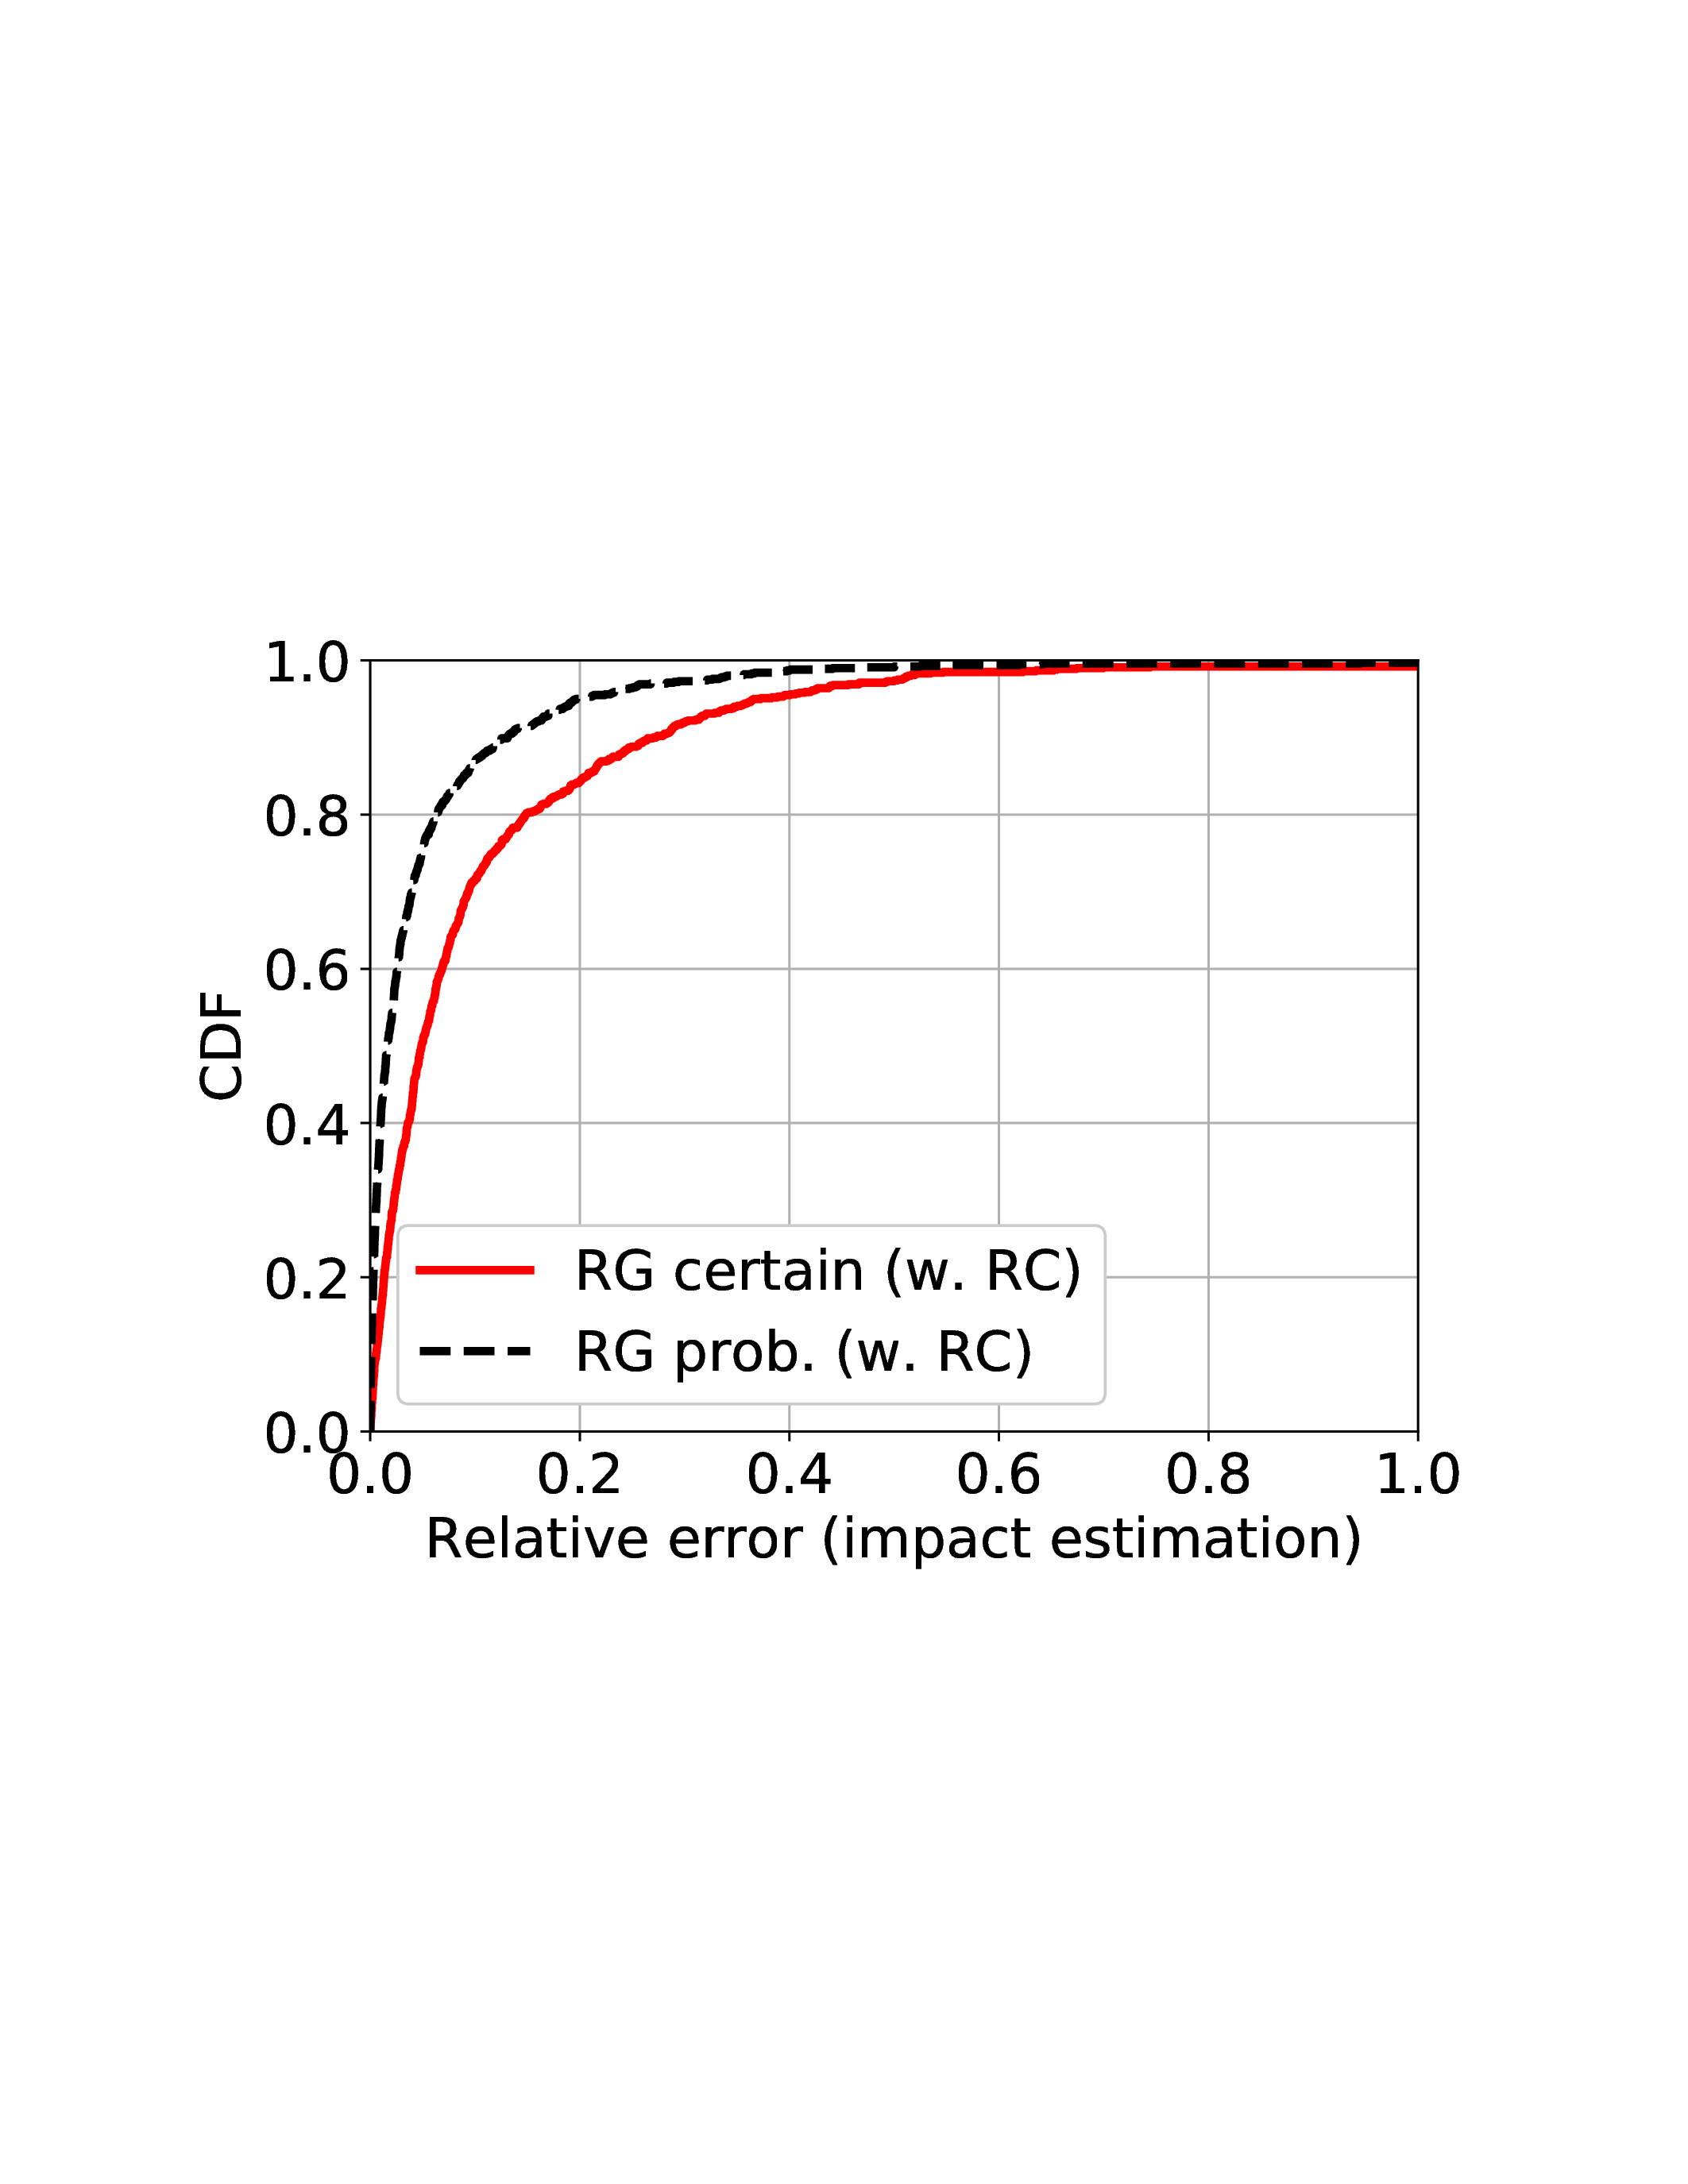}\label{fig:sims-impact-Rgraph-cdfs-with-RC}}
\subfigure[with RA]{\includegraphics[width=0.33\linewidth]{./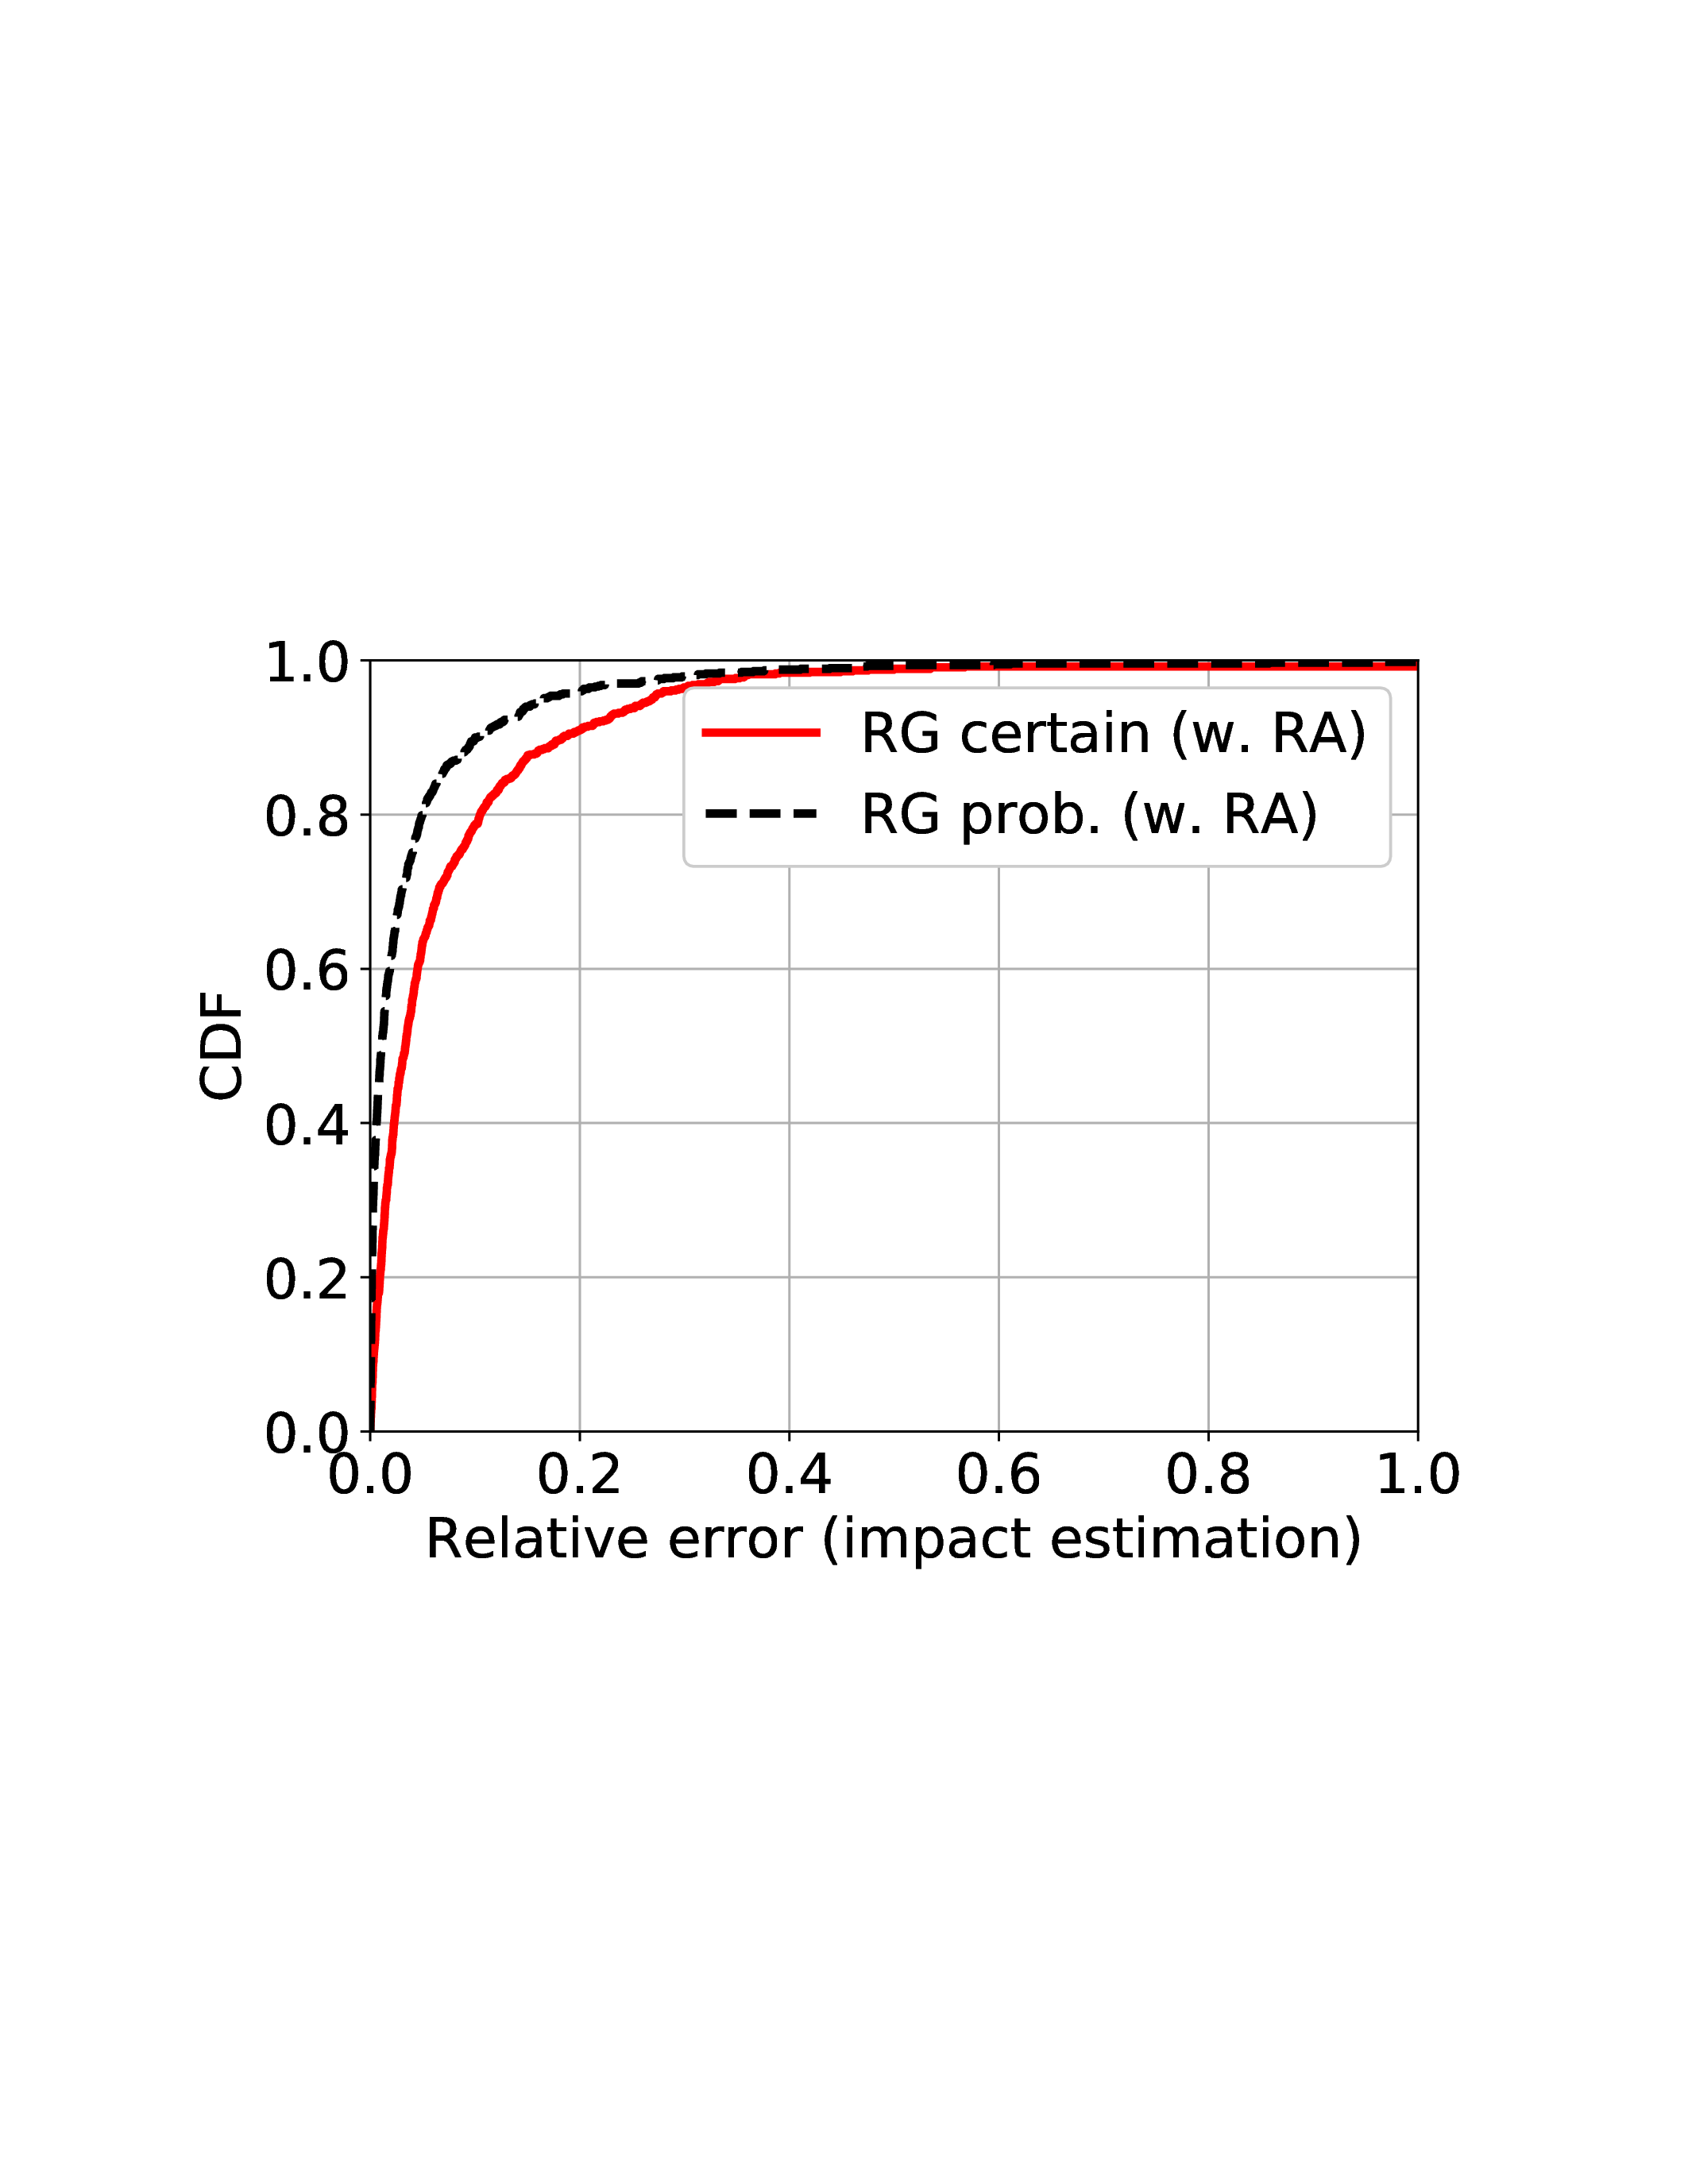}\label{fig:sims-impact-Rgraph-cdfs-with-RA}}
\caption{CDF of the relative error of impact estimation for hijacks of Type-0, with the R-graph based method using as estimator the certain catchment (continuous lines) and the probabilistic catchment (dashed lines), and inference (a) without measurements, (b) enhanced with RC measurements, (c) enhanced with RA measurements.}
\label{fig:sims-impact-Rgraph-cdfs}
\end{figure*}

\section{Monitor Similarity}\label{appendix:monitor-similarity}
See Fig.~\ref{fig:sims-monitor-similarity}.

\begin{figure*}
\centering
\subfigure[RC]{\includegraphics[width=0.49\linewidth]{./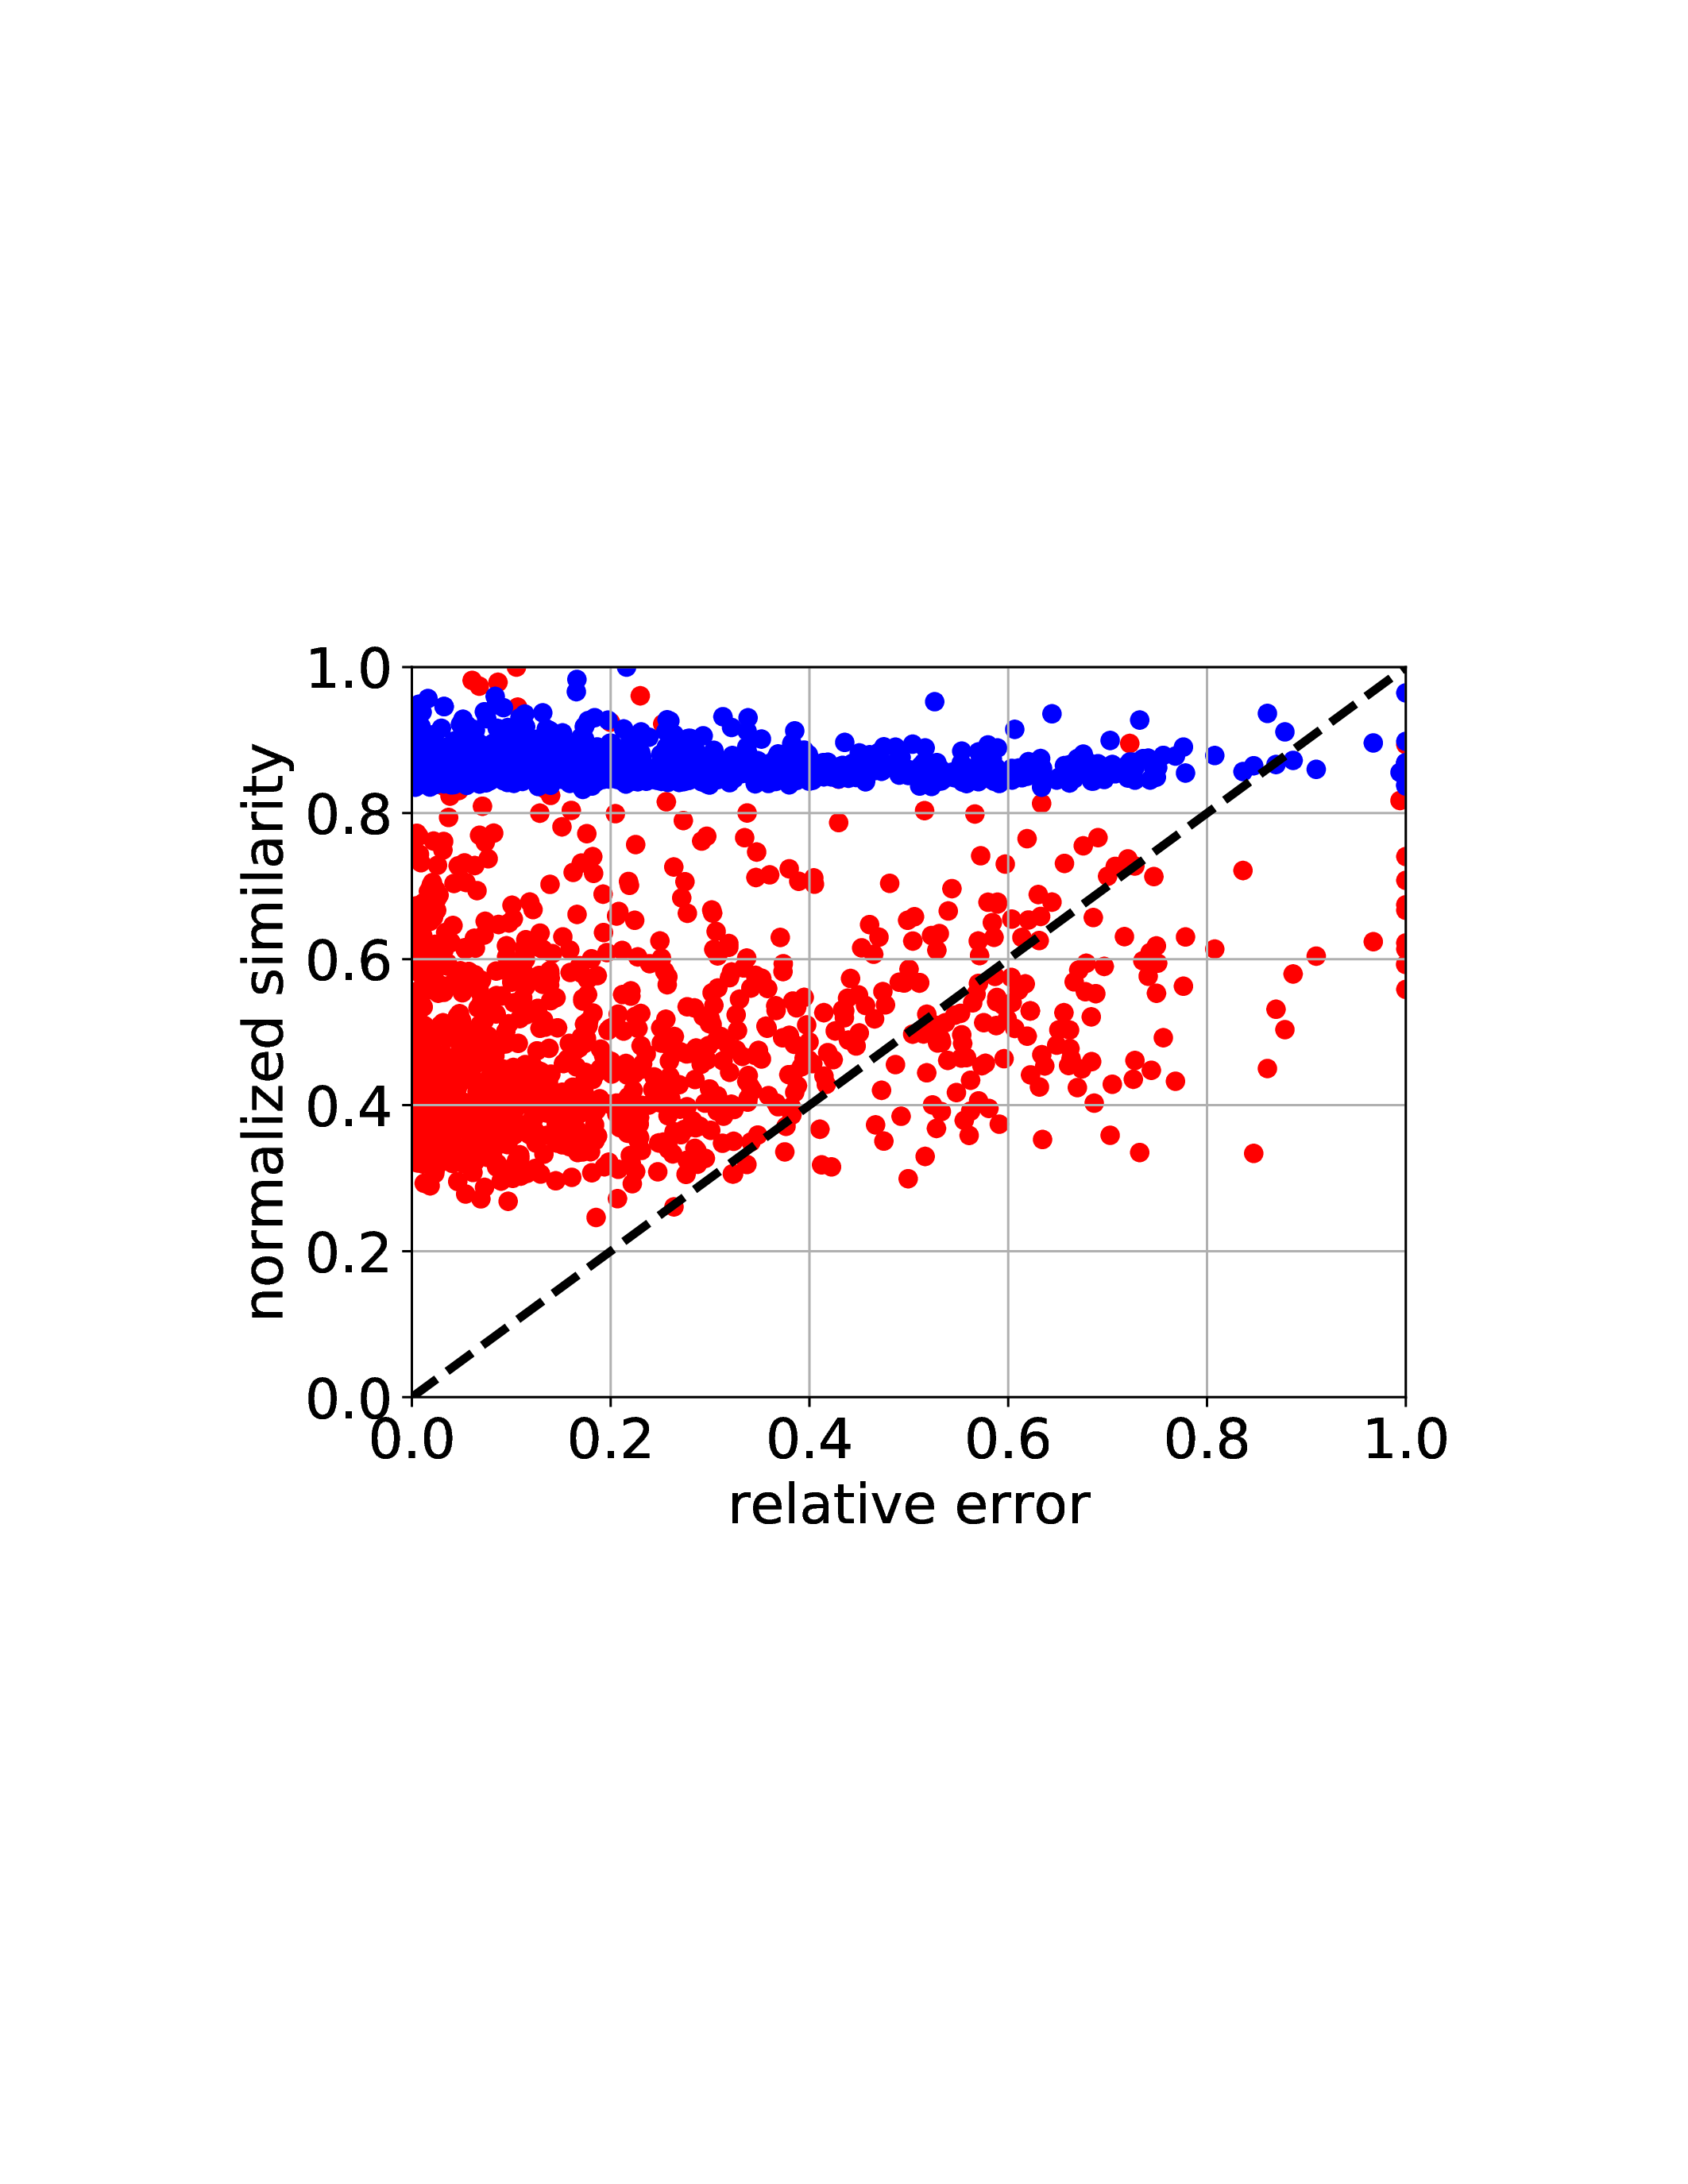}\label{fig:sims-monitor-similarity-RC}}
\subfigure[RA]{\includegraphics[width=0.49\linewidth]{./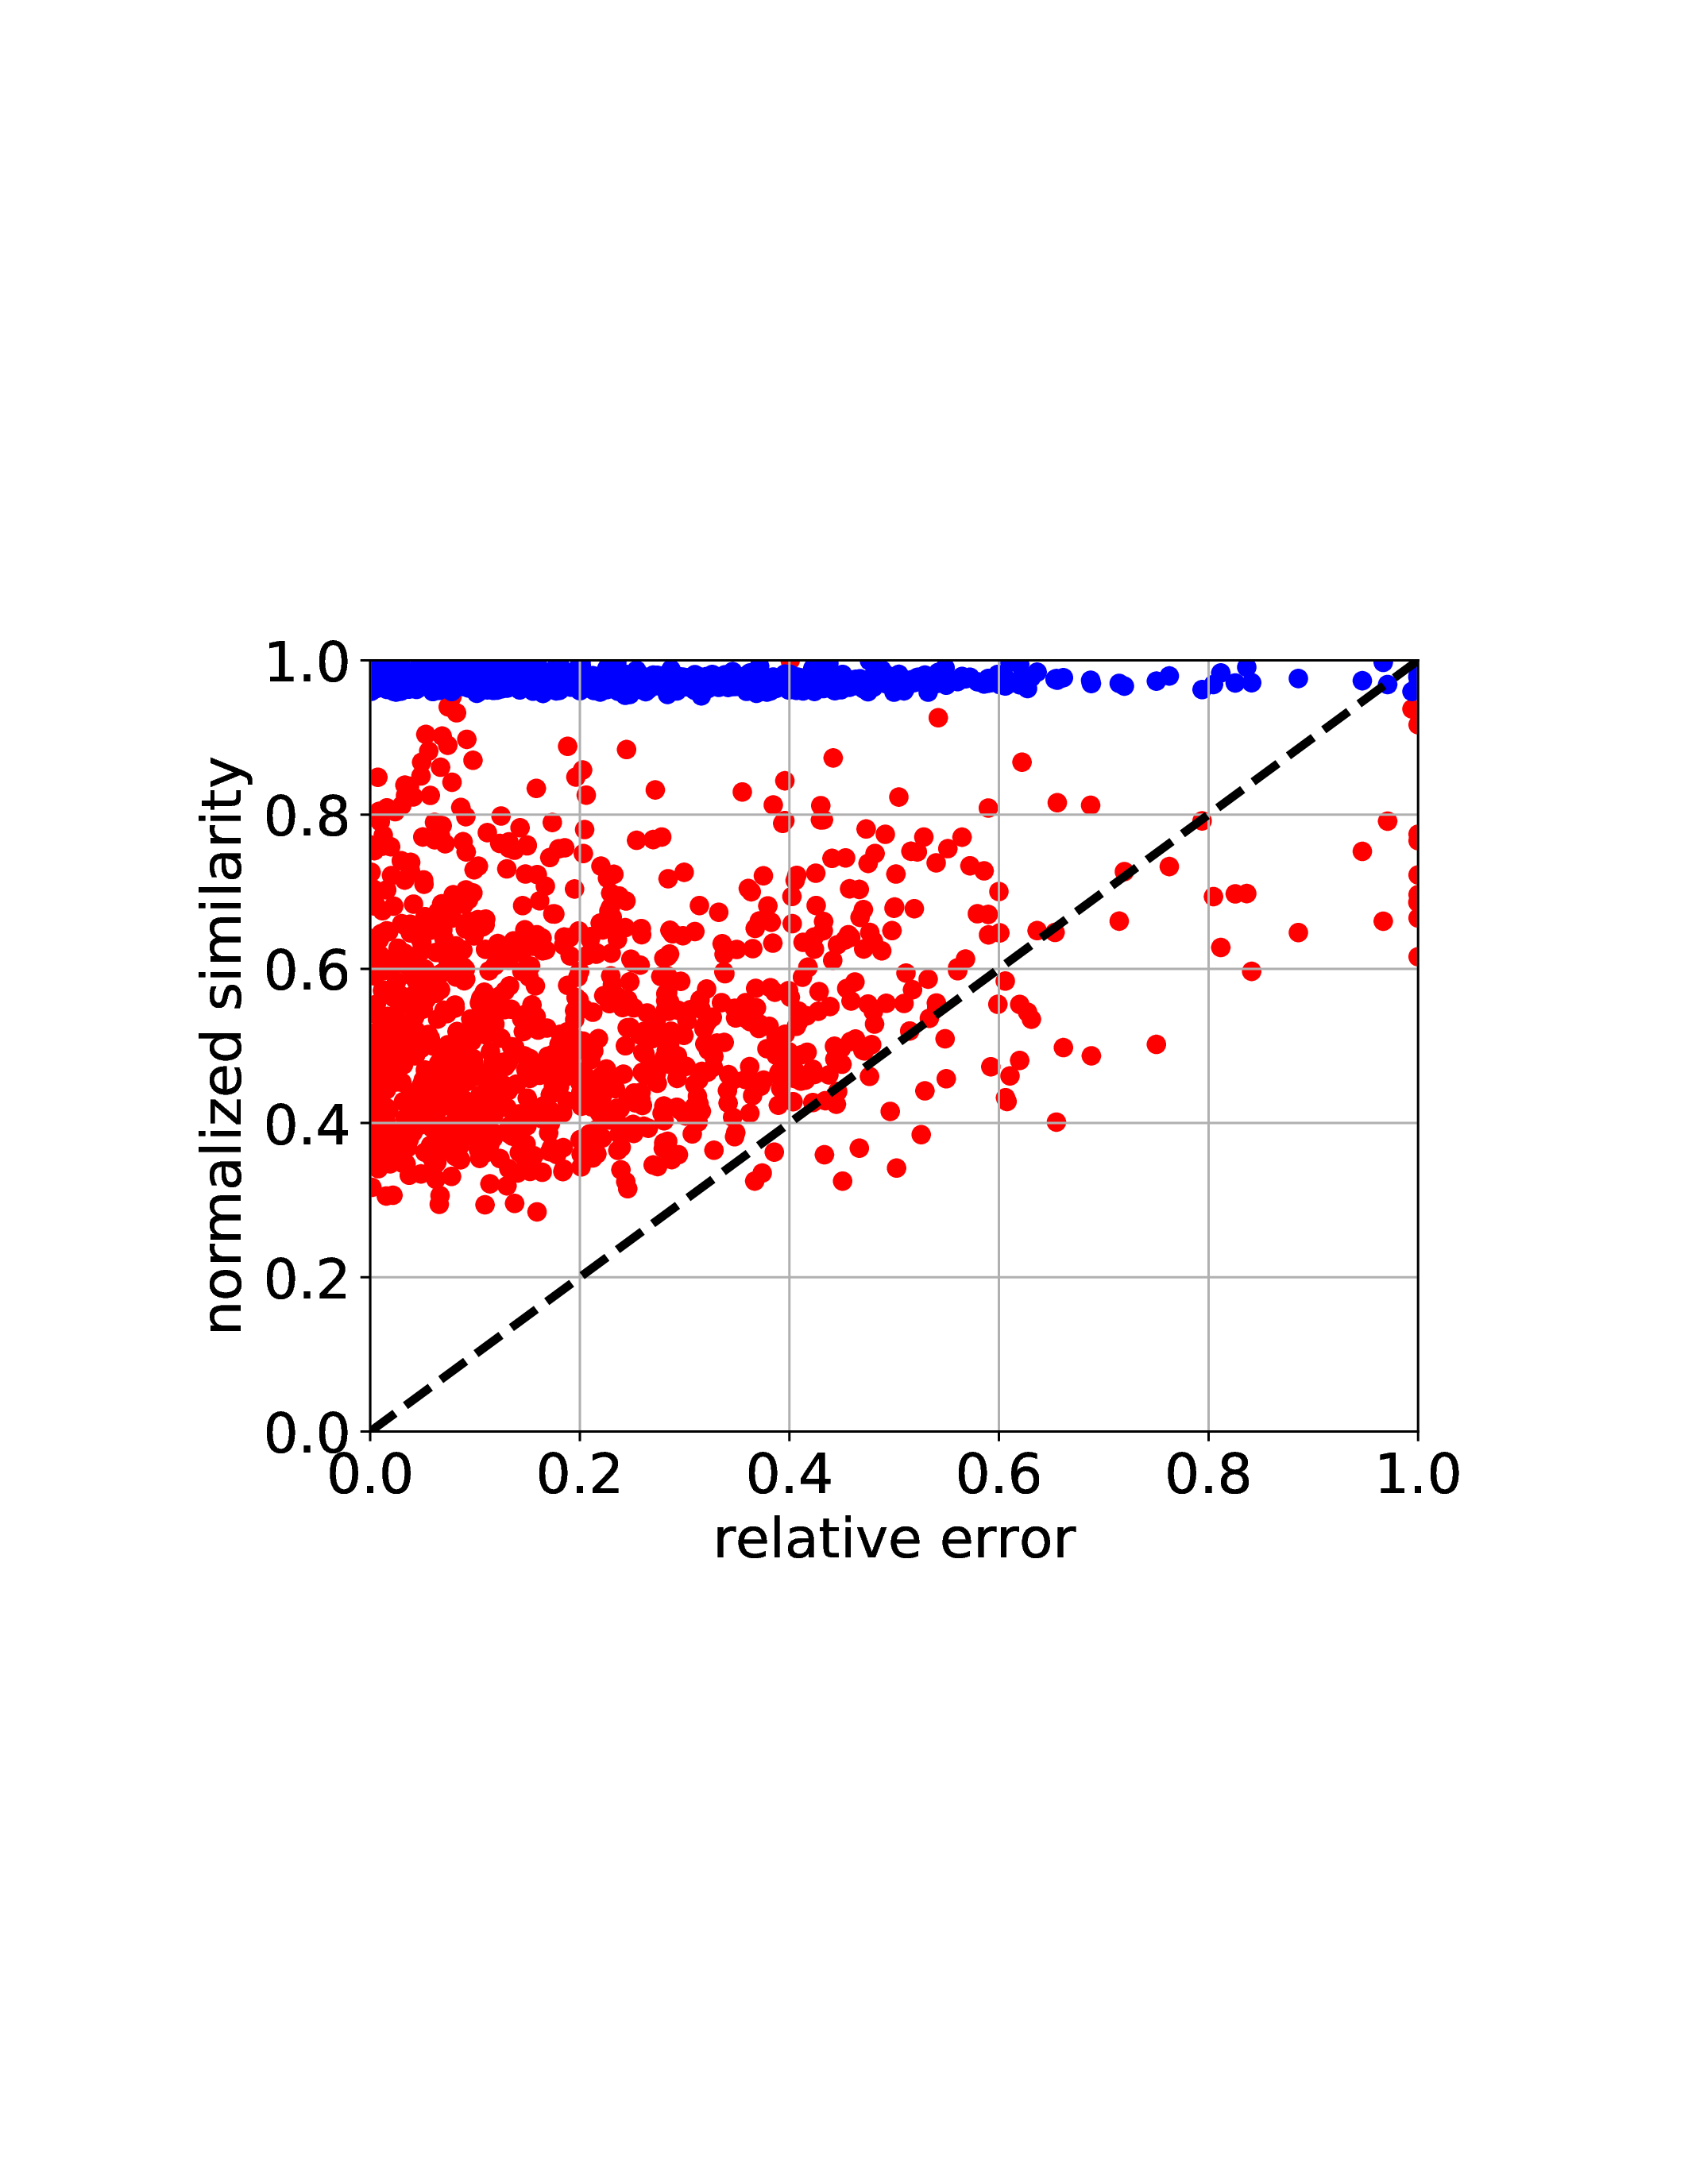}\label{fig:sims-monitor-similarity-RA}}
\caption{Scatter plot: relative error of impact estimation with the ``naive'' method (x-axis) vs. average similarity of monitors (y-axis) for Type-0 hijacks. Similarity measures: Jaccard (red dots) and R-graph (blue dots).}
\label{fig:sims-monitor-similarity}
\end{figure*}
