# Supplementary material for: Estimating the Impact of BGP Prefix Hijacking
Source: arXiv:2105.02346 source file (2021-05-05)
Supplement: Supplementary file 2 [file appendix_ridge.tex]

\pavlos{EXTRA}

\myitem{Discussion.} We tested different approaches to identify and isolate the correlations between the monitors. For instance, we (i) explicitly calculated the correlations between monitors from the matrix $\mathbb{M}=\{m_{i}^{(j)}\}$ and (greedily) selected sets of monitors with lower correlations: the resulting RMSE was similar to or better than those of NIE, but worse than those of LRE. Apart from linear regression we tested several other machine learning models, with results similar or worse than LRE (we preferred LRE due to the benefits of simpler models). Finally, we tested ML models taking into account topology and connectivity information of monitors (path lengths to the victim/hijacker ASes, sequence of AS-links, AS-relationships, etc.).

While the location and connectivity of monitors is known (or, can be inferred based on public datasets), it is unclear how it affects their observations upon a hijacking event. For example, two monitors may be located geographically close, but have very different connectivity

First model how the different topology, connectivity, etc., parameters create correlations between observations, and then use this model to isolate correlations in measurement. However, this two-step approach

Interpretable models come with a number of advantages, which make them preferable (e.g., compared to deep learning techniques that typically are considered as black-boxes) and is in line with the recent efforts for explainable ML models and AI algorithms~\cite{weld2019challenge}.

Specifically, using a linear regression model (i) can help towards understanding of the bias introduced by the deployment of the RC monitors and how it can be mitigated, and thus (ii) it can provide insights for future (analytic) modeling efforts; moreover, (iii) it is simple to implement and adapt, for example, to fine-tune the model using data from real hijacking events whose impact is measured (e.g., from ongoing activities to create a database about hijacking events\pavlos{cite observatory}) or to adapt the model for different hijack settings (e.g., adapting it per AS / potential victim, or focusing on the case of ASes known as serial hijackers~\cite{testart2019profiling}\footnote{In the former example one can simulate hijacks towards the given AS by considering different ASes, and in the latter example, simulate hijacks from one of the serial hijackers and randomly selecting victim.}).

\subsection{Designing an ML-based Hijack Impact Estimator}

\myitem{Interpreting the model.} The linear combination of the features in LRE, enables us to understand the role of each feature from the value of the weights in Table~\ref{tab:LRE-parameters-vs-nbMons-vs-hijackTypes}. In both LRE models, we can see that: (i) NIE plays the major role, by contributing around 70\%-90\% in the prediction. This was expected qualitatively (the values of $w_{NIE}$ quantify its role), since the NIE already can estimate the impact to a certain accuracy, and our goal is just to ``correct'' it and improve its estimations. The role of NIE increases with $M$, where the estimation becomes more robust (see Fig.~\ref{fig:RMSE-NIE-random-RC-RA-vs-nb-monitors-Type0}), while for small $M$ the ``corrections'' in the NIE are larger. (ii) There is a constant factor that contributes around 10\%, i.e., even if none of the measured monitors was infected, the LRE would predict an impact of $w_{0}$. While this term is seemingly counter-intuitive, it corresponds to the (average) value of the impact not seen by any RC monitors; in fact, we tested linear regression models where we forced $w_{0}=0$, and we observed higher RMSE values, thus verifying the role of this constant implicit impact. Moreover, the less the monitors, the higher the probability that none of the $M$ monitors is infected, which explains that $w_{0}$ increases for lower values of $M$. (iii) Both the features $f_{dist}$ and $f_{pref}$, indicate how ``preferrable'' by the RC monitors is the route to the victim compared to the hijacker's route: the higher the value of the feature, the more ``preferred'' is the victim route by the monitors, and thus the more probable is that the impact is underestimated. Hence, the weights $w_{f}$ are positive, to ``correct'' this underestimation. The contribution of $f_{dist}$ and $f_{pref}$ is around 8\% and 10\%, respectively.

\vkotronis{Regarding $f_{pref}$, is it simply a convention that we explain it from the victim's perspective, or sth else? For example, couldn't we interpret this from the hijacker's perspective too? Also, why don't we use both $f_{dist}$ and $f_{pref}$ within the regressor's formula?}

\myitem{Practical Implementation.}

\pavlos{Our results, which we will make public, is the first step towards building a dataset for MOAS events, whose data can be used to fit LRE (or, other) estimators}
