# Supplementary material for: Estimating the Impact of BGP Prefix Hijacking
Source: arXiv:2105.02346 source file (2021-05-05)
Supplement: Supplementary file 3 [file appendix_proofs_long.tex]

\section{Proof of Theorem~\ref{thm:NIE-bias-rmse}}\label{appendix:proof-NIE-bias-rmse}

The hijack impact $I$ is the fraction of ASes that are infected. Hence, choosing randomly the ASes/monitors to be measured, means that the probability that a selected monitor to be infected is $I$ (and $1-I$ to not be infected), i.e., a Bernoulli trial with probability $I$. 

The NIE involves the sum of $M$ independent Bernoulli trials (since in all practical cases $M\ll N\approx 65k$), and thus the sum follows a binomial distribution with parameters $M$  (number of trials) and $I$ (probability of success), i.e., 
\begin{equation}
\sum_{i\in\mathcal{M}}m_{i}\sim Binomial(M,I)
\end{equation}
and thus it holds that
\begin{align}
E\left[\textstyle\sum_{i\in\mathcal{M}}m_{i}\right] &= M\cdot I\label{eq:expectation-binomial}\\
Var\left[\textstyle\sum_{i\in\mathcal{M}}m_{i}\right] &= M\cdot I\cdot (1-I)\label{eq:variance-binomial}
\end{align}

\myitem{Bias.} The bias of an estimator is defined as
\begin{equation}\label{eq:bias-generic}
Bias = E[\hat{I}-I] = E[\hat{I}]-I
\end{equation}

For the NIE it holds that 
\begin{align}
E[\hat{I}]  &= E\left[\frac{1}{M}\cdot \textstyle\sum_{i\in\mathcal{M}}m_{i}\right]\nonumber\\
            &= \frac{1}{M}\cdot E\left[ \textstyle\sum_{i\in\mathcal{M}}m_{i}\right]\nonumber\\
            &= \frac{1}{M}\cdot M\cdot I\nonumber\\
            &=I\label{eq:expectation-nie}
\end{align}
where in the second line we used the expression of \eq{eq:expectation-binomial}. Substituting \eq{eq:expectation-nie} in \eq{eq:bias-generic} gives $Bias=0$, i.e., the NIE is an unbiased estimator.

\vspace{\baselineskip}
\myitem{RMSE.}
The RMSE of NIE, given that the actual hijack impact is $I$, is given
\begin{align}
RMSE(I)   &= \sqrt{E[(\hat{I} - I)^2]}\nonumber\\
            &= \sqrt{E[(\hat{I} - E[\hat{I}])^2]}\nonumber\\
            &= \sqrt{Var[\hat{I}]}\nonumber\\
            &= \sqrt{Var[\frac{1}{M}\textstyle\sum_{i\in\mathcal{M}}m_{i}]}\nonumber\\
            &= \sqrt{\frac{1}{M^{2}}\cdot Var[\sum_{i\in\mathcal{M}}m_{i}]}\nonumber\\
            &= \sqrt{\frac{1}{M^{2}}\cdot M\cdot I\cdot (1-I)}\nonumber\\
            &= \frac{\sqrt{I\cdot (1-I)}}{\sqrt{M}}\label{eq:rmse-i}
\end{align}
where the third line follows from the definition of the variance ($Var(x)=E[(x-E[x])^{2}]$), and in the fifth line we used the expression from \eq{eq:variance-binomial}.

Then,the RMSE of NIE follows by taking the expectation of $RMSE(I)$ (given in \eq{eq:rmse-i}) over the distribution $f(I)$ of the impact $I$
\begin{align}
RMSE    &= \int_{0}^{1} RMSE(I) \cdot f(I)\cdot dI\nonumber\\
        &= \int_{0}^{1} \frac{\sqrt{I\cdot (1-I)}}{\sqrt{M}} \cdot f(I)\cdot dI\nonumber\\ 
        &= \frac{1}{\sqrt{M}} \cdot \int_{0}^{1} \sqrt{I\cdot (1-I)}\cdot f(I)\cdot dI\nonumber\\
        &= \frac{1}{\sqrt{M}} \cdot c_{I}
\end{align}
The probability distribution $f(I)$ of the hijack impact depends on the hijack type $I$ (and the possible victim-hijacker pairs, \{V,H\}, if they are not randomly chosen).

% \subsection{Proof of Proposition~\ref{thm:rmse-vs-mae}}\label{appendix:proof-rmse-vs-mae}
% Let us denote the function $f(x) = \sqrt{x}$ and the variable $X = (\hat{I}-I)^{2}$. Then, we can write
% \begin{align}
%     RMSE    &= \sqrt{E[(\hat{I}-I)^{2}]} = f(E[X])\\
%     MAE     &=E[|\hat{I}-I|] = E[\sqrt{(\hat{I}-I)^2}] = E[f(X)]
% \end{align}
% Since $f$ is a concave function, applying Jensen's inequality gives
% \begin{equation*}
% f(E[X]) \geq E[f(X)] \Rightarrow RMSE \geq MAE
% \end{equation*}

\section{Bias of NIE for random \{V,H\} pairs}\label{appendix:unbiased-NIE-generic}
% \subsection{Proof of Corollary~\ref{thm:unbiased-NIE-generic}}\label{appendix:unbiased-NIE-generic}
\begin{corollary}\label{thm:unbiased-NIE-generic}
$Bias_{NIE(\mathcal{M})} = E[\hat{I}-I] =0,~\forall \mathcal{M}$, when the expectation is taken over all possible \{V,H\} node pairs.
\end{corollary}
\begin{proof}
Let $I_{12}$ ($\hat{I}_{12}$) be the impact (estimation) for the node pair $\{V=n1, H=n2\}$, $I_{21}$ ($\hat{I}_{21}$) the impact (estimation) for the node pair $\{V=n2, H=n1\}$. Since it holds that $I_{12}+I_{21}=1$ and $\hat{I}_{12}+\hat{I}_{21}=1$, when both \{V,H\} pairs are equally probable, the bias of NIE is given by 
\begin{align*}
E[\hat{I}-I] 
&= \frac{1}{2}\cdot(\hat{I}_{12}-I_{12}) + \frac{1}{2}\cdot(\hat{I}_{21}-I_{21})\\
&= \frac{1}{2}\cdot(\hat{I}_{12}+\hat{I}_{21}) - \frac{1}{2}\cdot(I_{12}+I_{21})\\
&= \frac{1}{2}-\frac{1}{2} =0
\end{align*}
The corollary straightforwardly follows by generalizing the above all all possible \{V,H\} pairs, since for each pair \{V=i,H=j\} there exists a pair \{V=j,H=i\}, and every AS pair is equally probable to be the victim-hijacker pair.
\end{proof}

\section{Proof of Theorem~\ref{thm:NIE-bias-rmse-p}}\label{appendix:proof-NIE-bias-rmse-p}

If $m_{i}=1$, then $\hat{m}_{i}$ is $1$ as well. However, if $m_{i}=0$, then $\hat{m}_{i}$ is $1$ with probability $p$ (by Definition~\ref{def:ping-failure}) and $\hat{m}_{i}$ is $0$ with probability $1-p$. Taking into account also the fact that the indicator $m_{i}$ follows a Bernoulli trial with probability $I$ (see Appendix~\ref{appendix:proof-NIE-bias-rmse}), i.e., $P\{m_{i}=1\}=I$ and $P\{m_{i}=0\}=1-I$., the expectation of the indicator $\hat{m}_{i}$ can be calculated as follows
\begin{align}
E[\hat{m}_{i}] 
&= 1\cdot P\{m_{i}=1\} + 1\cdot P\{m_{i}=0\}\cdot P\{\hat{m}_{i}=1 | m_{i}=0\} \nonumber\\
& ~\hspace{1cm}+ 0\cdot P\{m_{i}=0\}\cdot P\{\hat{m}_{i}=0 | m_{i}=0\} \nonumber\\
&= 1\cdot I + 1\cdot (1-I)\cdot p + 0\cdot (1-I)\cdot (1-p) \nonumber\\
&= I + (1-I)\cdot p \label{eq:expectation-hat-m}
\end{align}

In the case of measurement failures, the expression of NIE is calculated from the indicators $\hat{m}_{i}$ (rather than the indicators $m_{i}$). Hence, the expected value of NIE is given by
\begin{align}
E[\hat{I}] 
&= E[\frac{1}{M}\sum_{i\in\mathcal{M}} \hat{m}_{i}] \nonumber\\
&= \frac{1}{M}\cdot E[\sum_{i\in\mathcal{M}} \hat{m}_{i}] \nonumber\\
% &= \frac{1}{M}\cdot M\cdot Prob\{no-response\}\nonumber\\
&= \frac{1}{M}\cdot M\cdot \left(I+(1-I)\cdot p\right) \nonumber\\ 
&= I+(1-I)\cdot p \label{eq:expectation-nie-failures}
\end{align}
where the third line follows by using the expression of \eq{eq:expectation-hat-m}.

\textit{Remark:} In fact, the expression of \eq{eq:expectation-nie-failures} can also be directly calculated by observing that the indicator $\hat{m}_{i}$ follows a Bernoulli trial with probability $I+(1-I)\cdot p$, i.e.,
\begin{equation}\label{eq:prob-hat-m}
P\{\hat{m}_{i}=1\} =     I+(1-I)\cdot p
\end{equation}

\vspace{\baselineskip}
\myitem{Bias.} The bias of the NIE follows straightforwardly by substituting \eq{eq:expectation-nie-failures} in the definition of the bias (\eq{eq:bias-generic}):
\begin{align}
Bias_{NIE} = E[\hat{I}-I] = (1-I)\cdot p
\end{align}

\vspace{\baselineskip}
\myitem{RMSE.} The RMSE of NIE, given that the actual hijack impact is $I$, is calculated as
\begin{align}
RMSE(I)
&= \sqrt{E[(\hat{I} - I)^2]}\nonumber\\
&= \sqrt{E[\hat{I}^2] + I^{2} - 2\cdot I\cdot E[\hat{I}]} 
\end{align}
Using the expression for the variance $Var(x) = E[x^2]-(E[x])^{2}$, gives
\begin{align}
RMSE(I) &= \sqrt{Var[\hat{I}]+(E[\hat{I}])^{2} + I^{2} - 2\cdot I\cdot E[\hat{I}]} \nonumber\\
&= \sqrt{Var[\hat{I}]+(E[\hat{I}]-I)^{2}}\nonumber\\
&= \sqrt{Var[\frac{1}{M}\cdot\sum_{i\in\mathcal{M}} \hat{m}_{i}]+(I+(1-I)\cdot p-I)^{2}} \nonumber\\
&= \sqrt{\frac{1}{M^{2}}\cdot Var[\sum_{i\in\mathcal{M}} \hat{m}_{i}]+((1-I)\cdot p)^{2}} \label{eq:rmse-I-failure-intermediate}
\end{align}
The quantity $\sum_{i\in\mathcal{M}} \hat{m}_{i}$ is the sum of $M$ independent Bernoulli trials with probability given by \eq{eq:prob-hat-m}, and thus it follows a binomial distribution with parameters $M$  (number of trials) and $I+(1-I)\cdot p$ (probability of success), i.e., 
\begin{equation*}
\sum_{i\in\mathcal{M}} \hat{m}_{i}\sim Binomial(M,I+(1-I)\cdot p)
\end{equation*}
and thus its variance is given by 
\begin{align}
Var&[\sum_{i\in\mathcal{M}} \hat{m}_{i}] 
= M\cdot P\{\hat{m}_{i}=1\}\cdot (1-P\{\hat{m}_{i}=1\})   \nonumber\\
&= M\cdot (I+(1-I)\cdot p)\cdot (1-I+(1-I)\cdot p) \label{eq:variance-sum-hat-m}
\end{align}
Substituting \eq{eq:variance-sum-hat-m} in \eq{eq:rmse-I-failure-intermediate}, gives
\begin{align}
&RMSE(I)=\nonumber\\
&= \sqrt{\frac{M\cdot\left(I+(1-I)\cdot p\right)\cdot \left(1-I-(1-I)\cdot p\right)}{M^{2}}  +((1-I)\cdot p)^{2}} \nonumber\\
&= \sqrt{\frac{1}{M}\cdot\left(I+(1-I)\cdot p\right)\cdot(1-I)\cdot (1-p) +(1-I)^{2}\cdot p^{2}} \nonumber\\
&= \sqrt{\frac{A_{I,p}}{M} + B_{I,p}} \label{eq:rmse-I-failure-final}
\end{align}
where 
\begin{align}
A_{I,p} &= \left(I+(1-I)\cdot p\right)\cdot(1-I)\cdot (1-p)\\
B_{I,p} &= (1-I)^{2}\cdot p^{2}    
\end{align}

Using \eq{eq:rmse-I-failure-final} and taking the expectation over the impact distribution $f(I)$, gives the expression of the Theorem.

\vspace{\baselineskip}
\myitem{Proof of Corollary~\ref{corollary:rmse-inf}.}
Corollary is proved by simply using $M\rightarrow\infty$ in \eq{eq:rmse-I-failure-final}:  For a large number of measurements (large $M$, or formally $M\rightarrow\infty$), we get
\begin{equation}
RMSE(I) \leq RMSE(I)_{M\rightarrow\infty} = (1-I)\cdot p    
\end{equation}
